# Supplementary material for: No learning rates needed: Introducing SALSA -- Stable Armijo Line Search Adaptation
Source: arXiv:2407.20650 source file (2024-07-30)
Supplement: Supplementary file 1 [file appendix.tex]

\subsection{Batch Size Scaling}

\begin{wrapfigure}{r}{0.5\textwidth}
 %\vspace{-0.05\textwidth}
    \subfloat[step size]{\includegraphics[width = 0.48\textwidth]{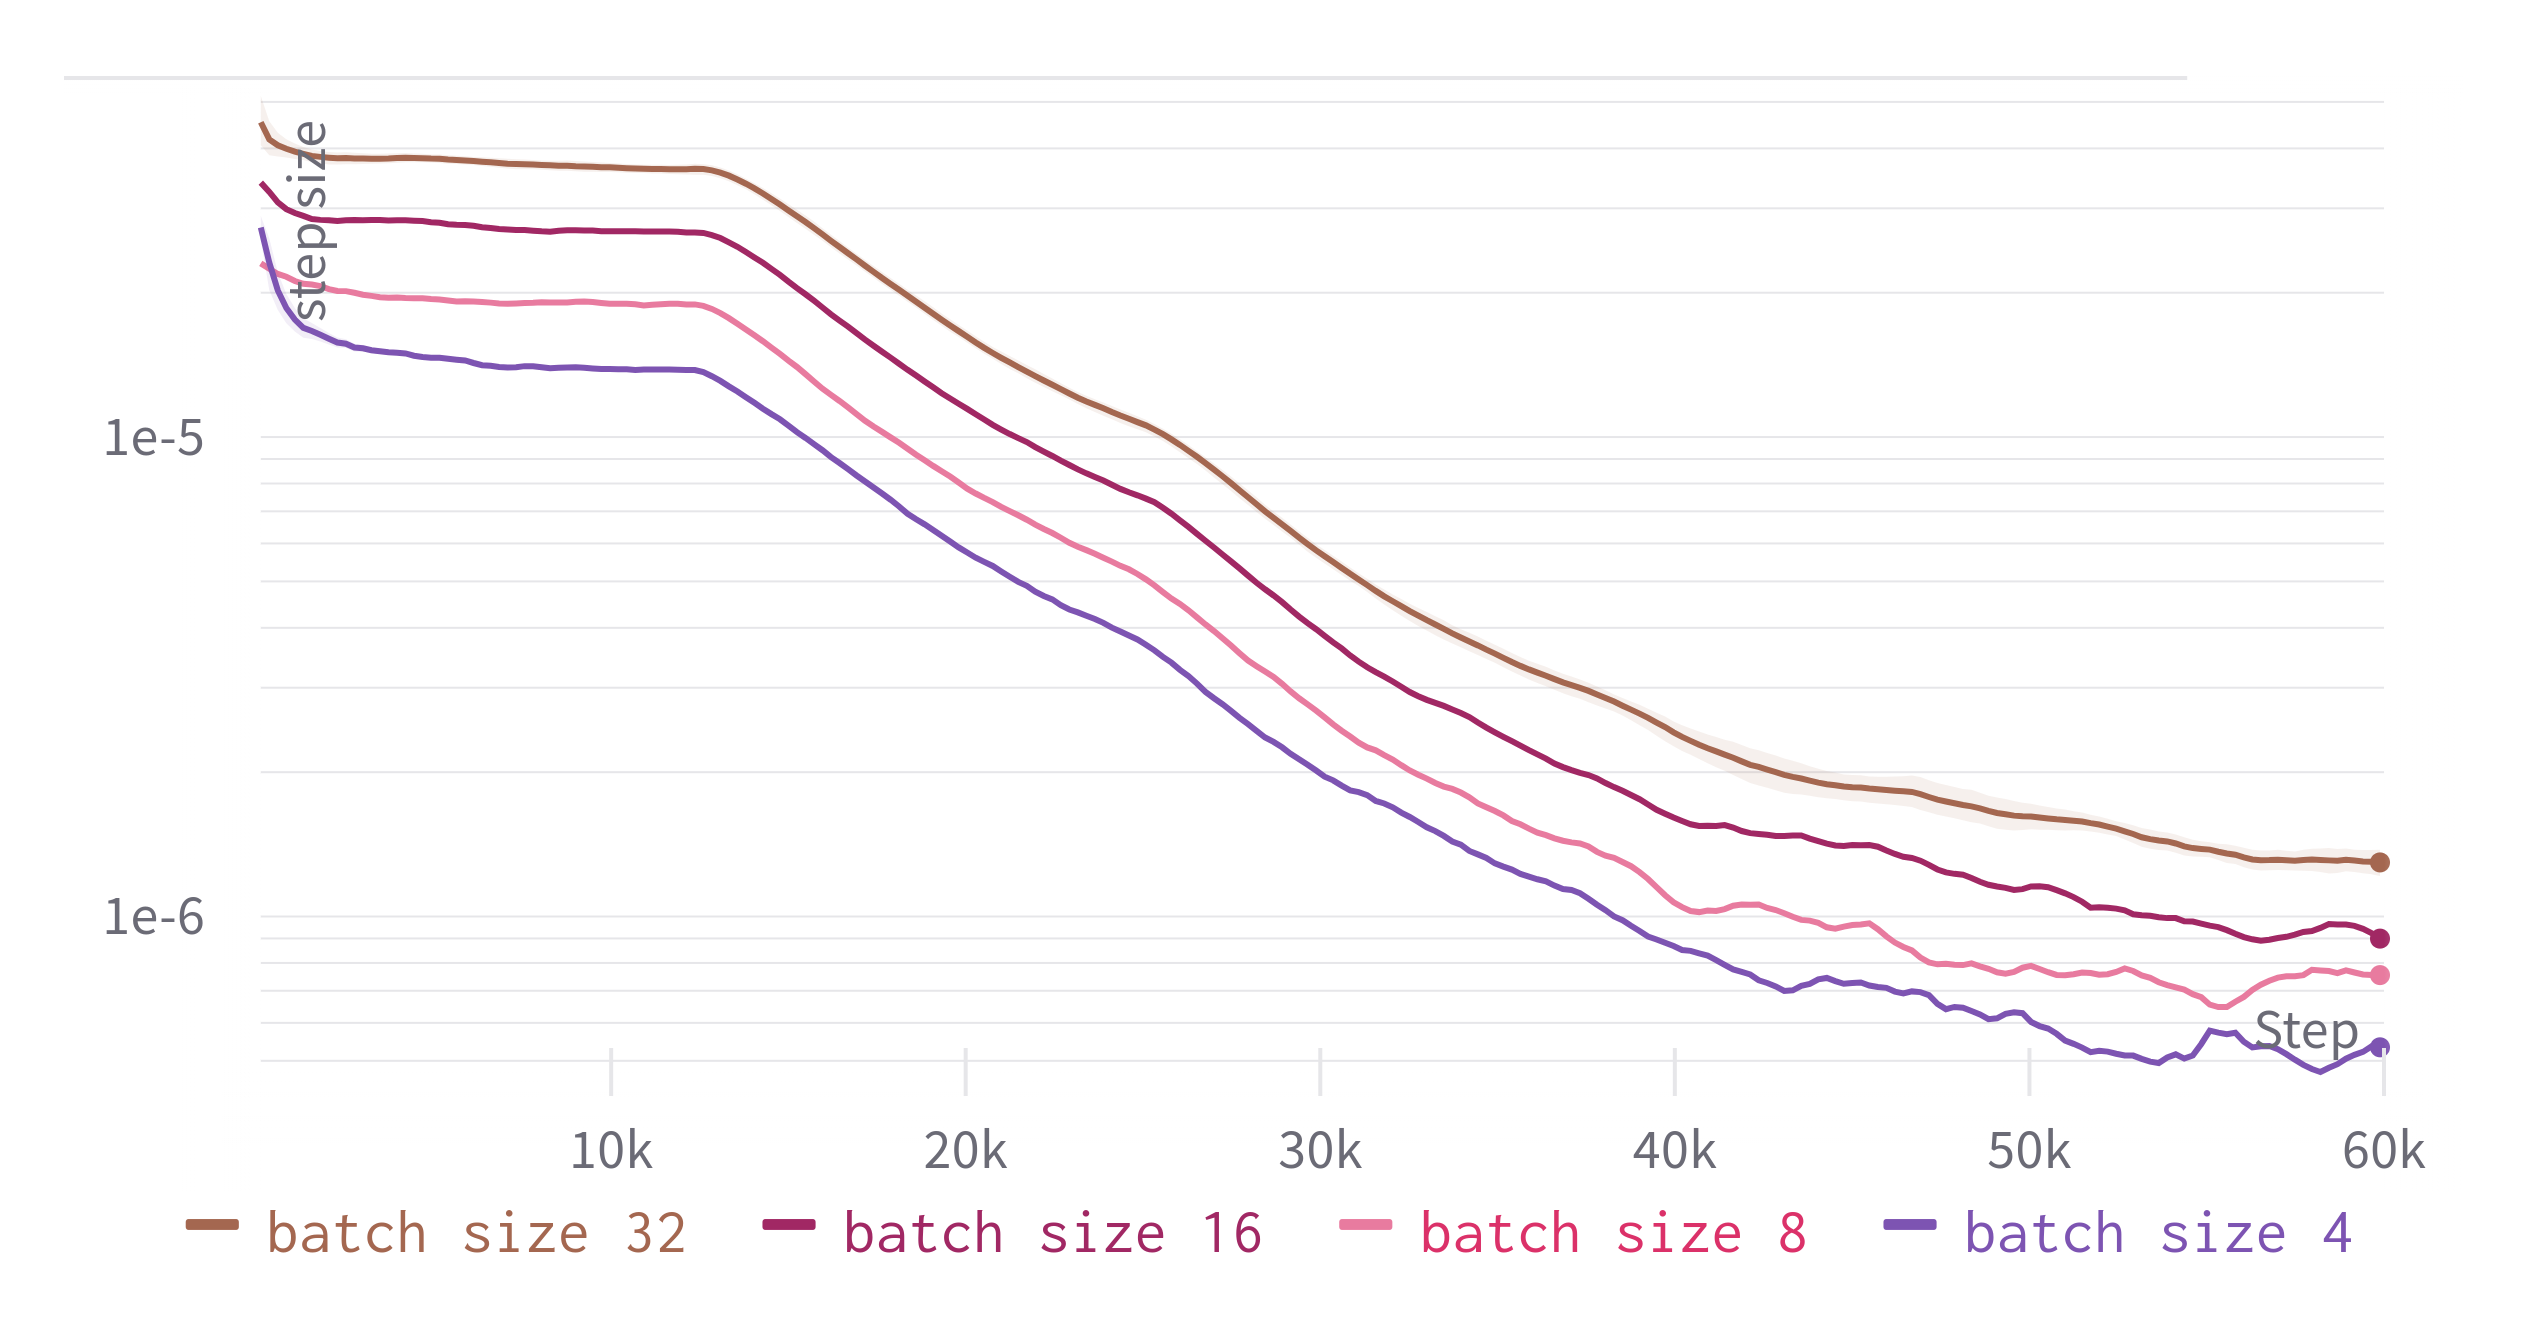}} \\
\subfloat[loss decrease]{\includegraphics[width = 0.24\textwidth]{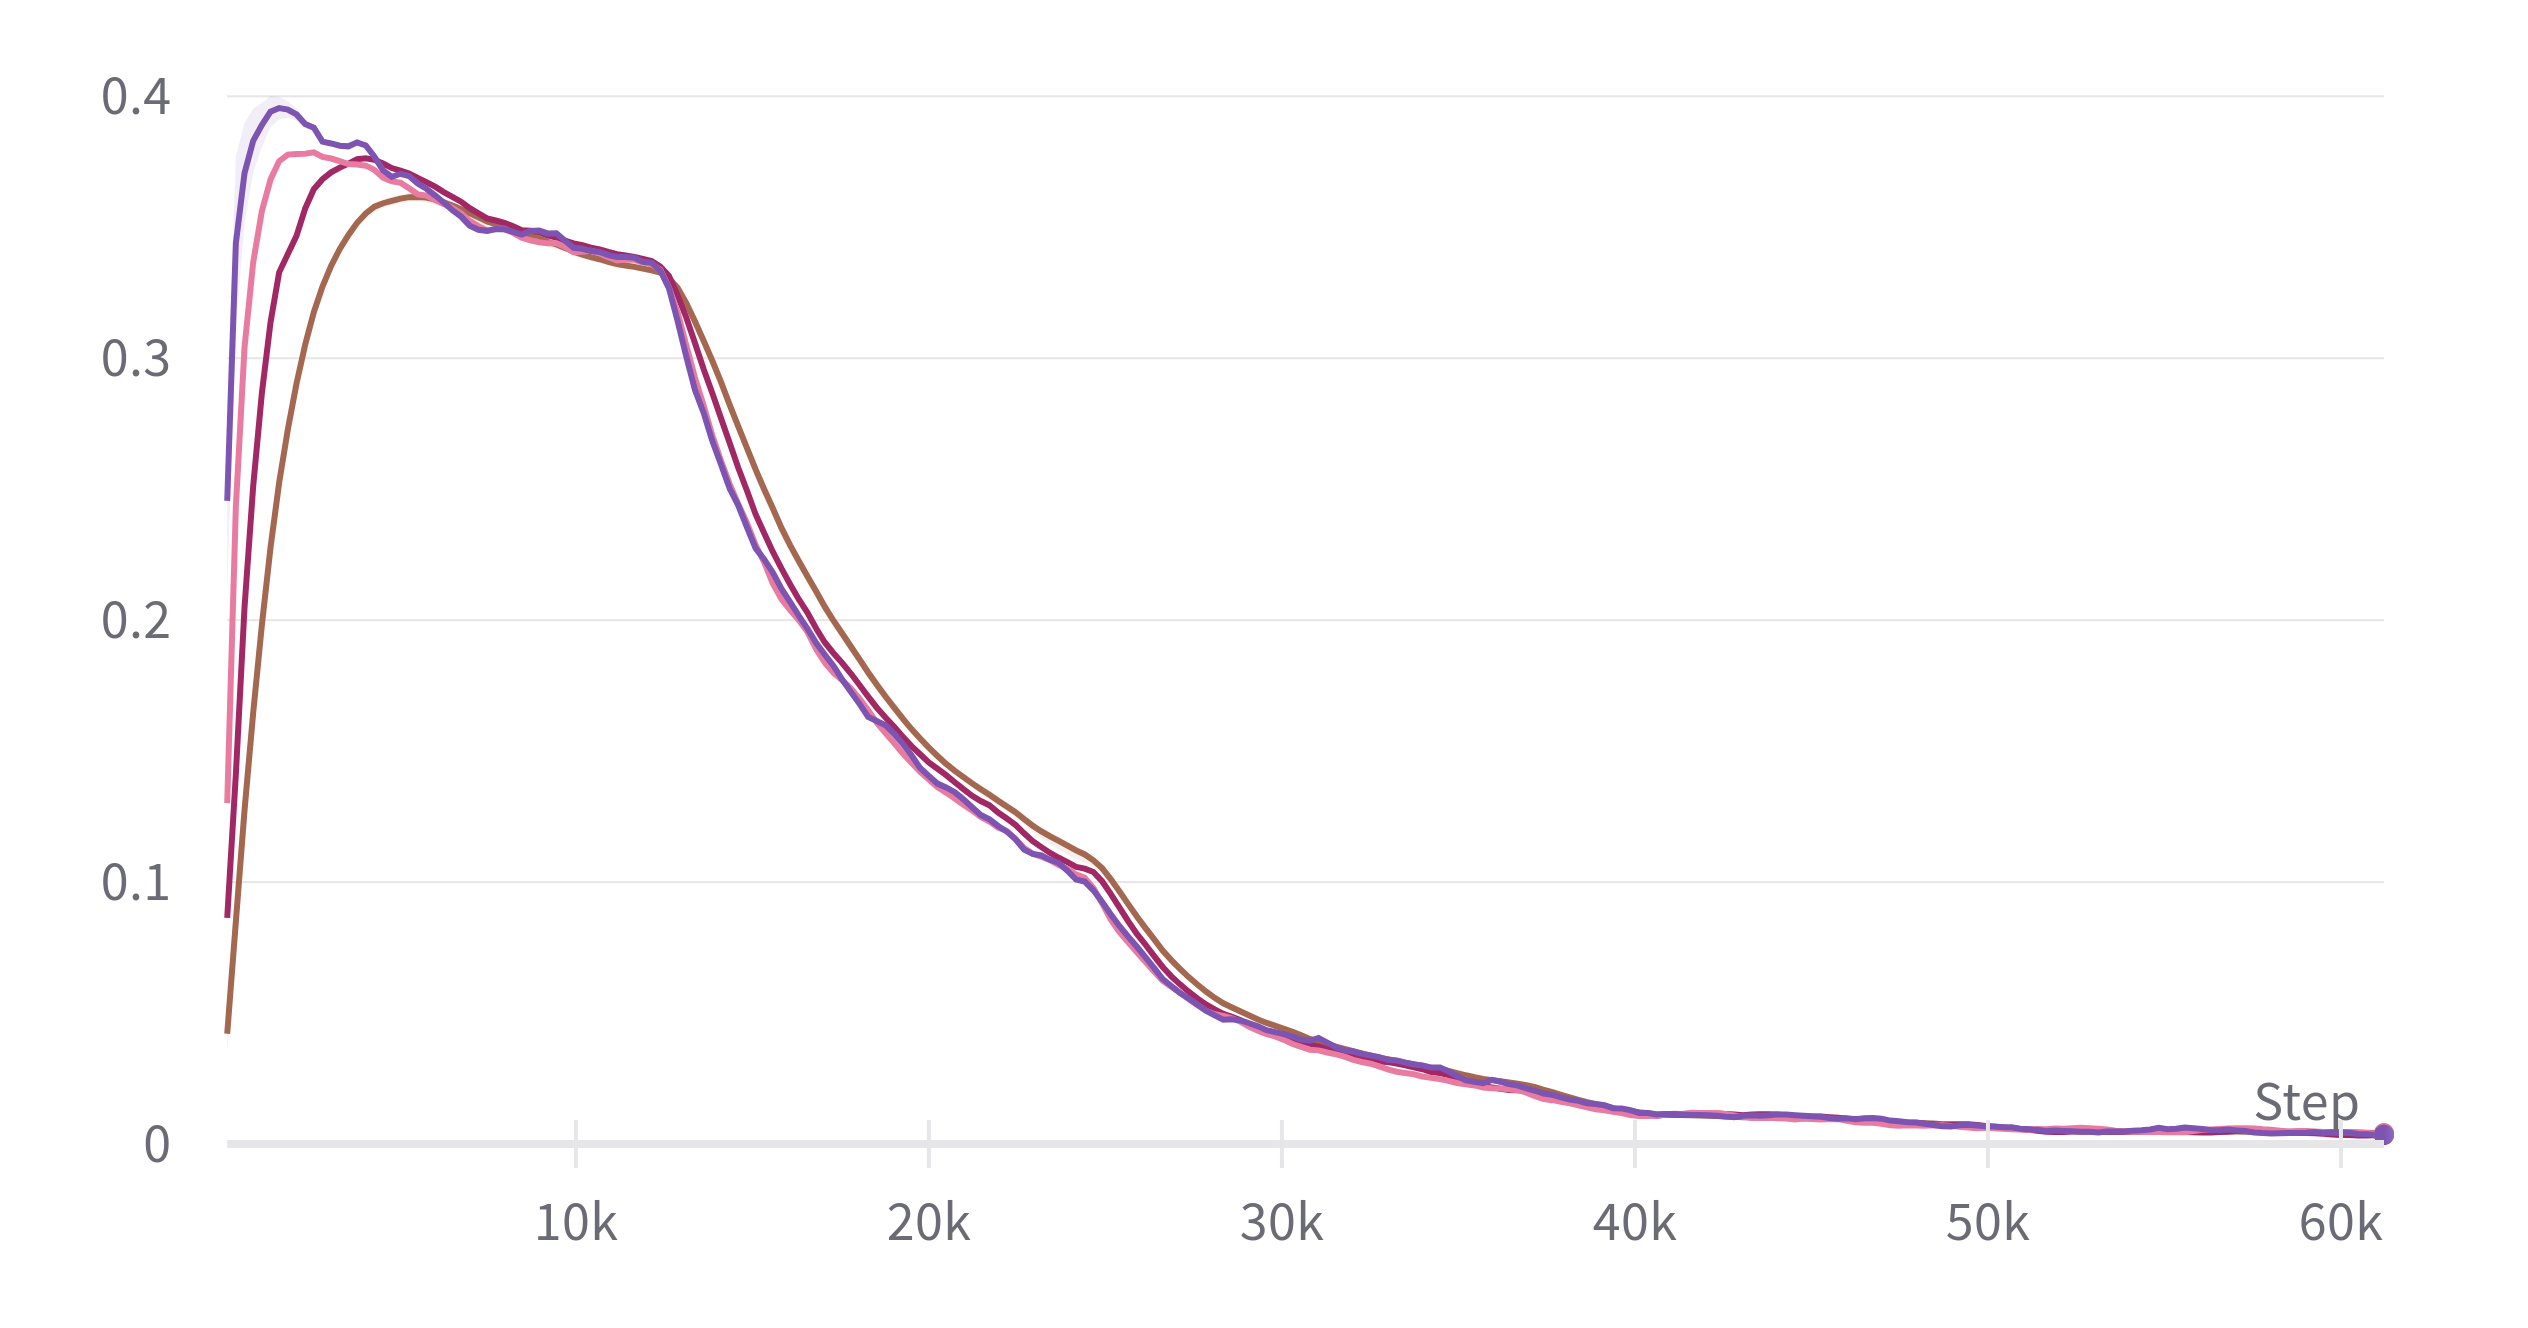}}  
\subfloat[gradient norm]{\includegraphics[width = 0.24\textwidth]{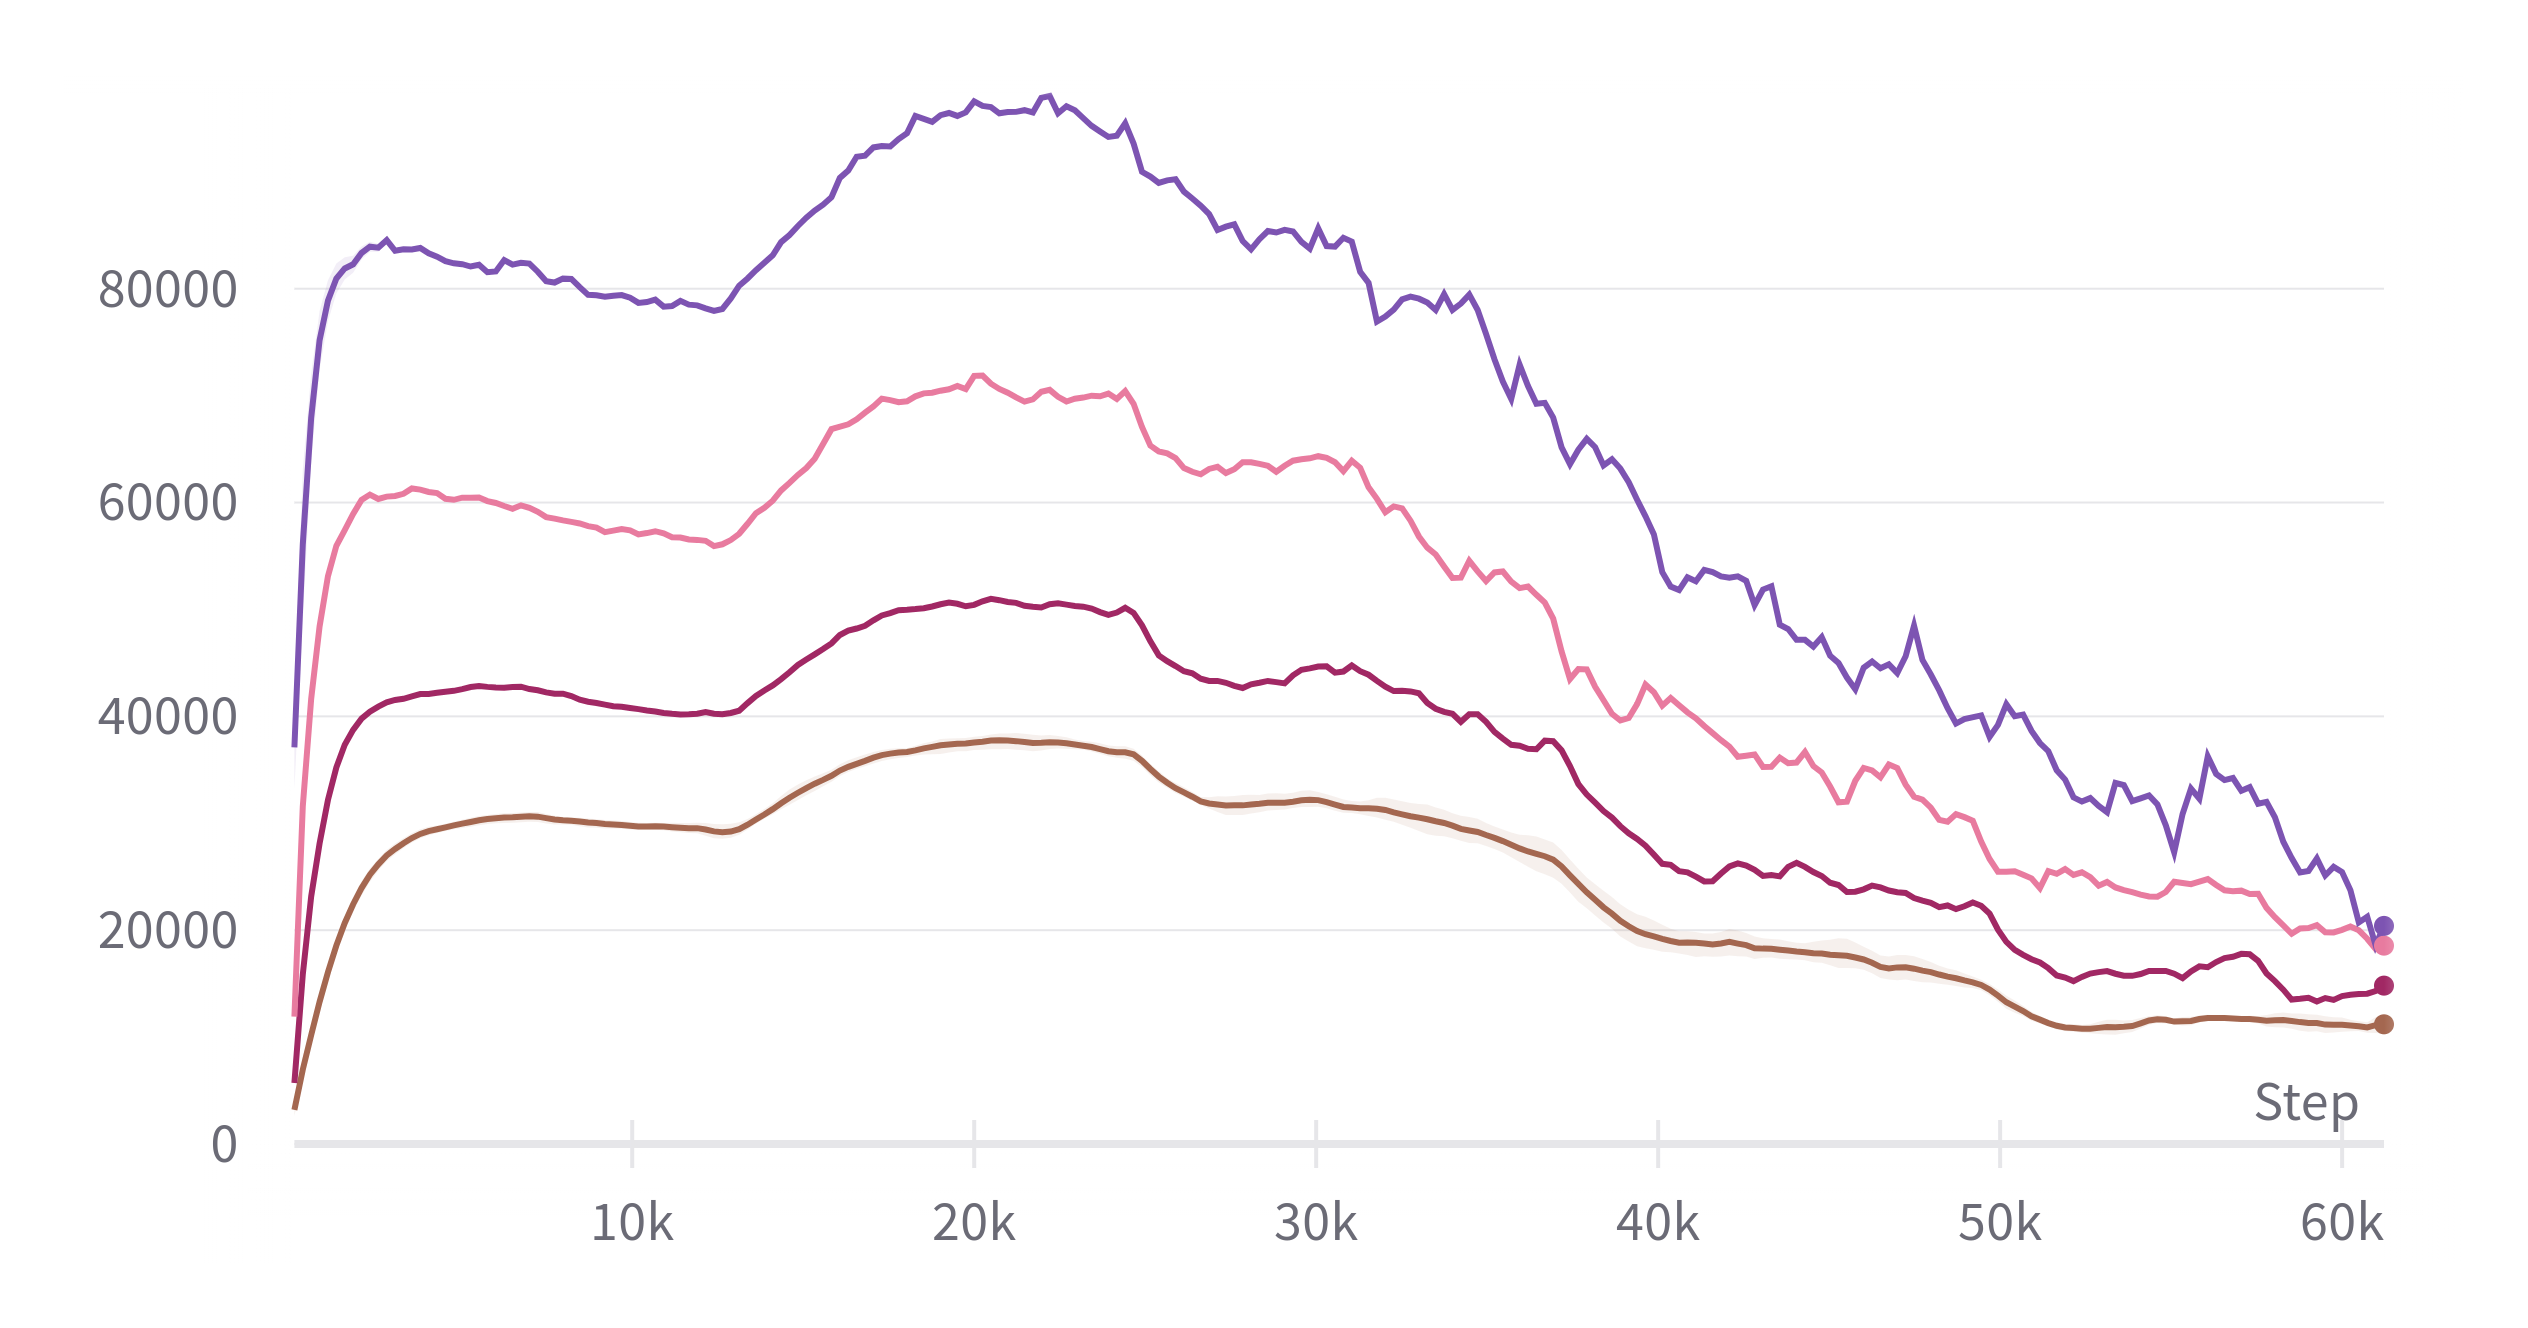}} 
\caption{Comparison of learning rates of ADAM + SaLSa dependent on the batch size on the MNLI dataset. Figure (b) depicts the loss decrease $h_k$ dependend on the batch size, here no great changes are present. Figure (c) depicts the gradient norm $s_k$ dependent on the batch size. Larger batches result in smaller gradient norms.}
\label{fig:batchcompare}
 %\vspace{-0.05\textwidth}
\end{wrapfigure}

In a previous study by \cite{batchnoise}, the impact of batch size on the optimal step size was examined. Theoretical findings indicated that for optimization methods such as SGD, the optimal step size scales linearly with the batch size,tthods like ADAM or AMSGRAD, the scaling follows a square root relationship.

To investigate the behavior of the step size to batch size ratio in the ADAM + SaLSa optimizer, we conducted training runs with varying batch sizes. Remarkably, we observed that the step size to batch size ratio remained relatively constant throughout the training process. Moreover, the step size exhibited a scaling behavior of approximately $\eta \sim \sqrt{2}$, which aligns with the theoretically predicted optimal value described in \citet{batchnoise}. In Table \ref{Fig:batchsizescaling}, we present the average multiplicative factor by which the step size increased with respect to the batch size.

%These findings provide encouraging evidence for the generalization capabilities of our method.

We take this as encouraging sign for the generalization abilities of our method.

The Armijo criterion \ref{eq:armijo} determines the step size by the ratio of loss decrease to gradient norm, visualized in \ref{fig:batchcompare}.
Notably, we observed that the primary factor influencing the reduction of step size is the increase in gradient norm, for lower batch sizes.
%We observe that the gradient norm increasing is the main factor for decreasing the step size, dependent on the batch size. 
%We show in Figure \ref{fig:batchcompare}, that ADAM + SaLSa result in roughly the same scaling rules, which further shows that the line search is robust and widely applicable. The resulting average scaling can be seen in Table \ref{Fig:batchsizescaling}. 

\begin{table}[h] 
  \centering
  \caption{Resulting average ratio of step size to previous step size of ADAM + SaLSa for doubling the batch size}
  \label{Fig:batchsizescaling}
  \begin{tabular}{ccc c}
    \toprule
    4$\Rightarrow$8 &  8$\Rightarrow$16 & 16$\Rightarrow$32 & optimal from \cite{batchnoise} \\
 \cmidrule(r){1-3}   \cmidrule(r){4-4}  
 1.325 & 1.423 & 1.420 & $\sqrt{2} \approx 1.414$ \\
    \bottomrule
  \end{tabular}
\end{table}

%\subsection{Discussion}
%In conclusion, we observe that SaLSa outperforms SLS or a tuned learning rate scheudle for Transformer fine-tuning and convolutional neural networks. For tabular datasets we see less clear results, here our optimization methods does not yield better performance. Furthermore, we show that SaLSa exhibits desirable properties in terms of step size to batch size scaling.

\newpage
\subsection{Additional Experimental Results}
\label{sec:additionalexp}
Below we show additional accuracy and loss curves for the experiments.

\begin{table*}[h] 
  \centering
  \caption{Ranking of classification accuracies, for all datasets and optimization methods. Best performing optimization method is marked in \textbf{bold}. }
  \label{Fig:accranking}
  \begin{tabular}{c cccccc}
    \toprule
 & ADAM & SGD & ADAM  & SGD  & ADAM  & SGD  \\
 & - & - & SLS & SLS &  SaLSa &  SaLSa \\
 \cmidrule(r){1-1}   \cmidrule(r){2-7} 
\it{MNLI} & 3 & 6 & \textbf{1}  & 5 & 2 & 4    \\
\it{QNLI} & \textbf{1} & 5 & 3  & 6 & \textbf{1} & 4   \\
\it{MRPC} & 6 & 4 & 2  & 4 & \textbf{1} & 3   \\
\it{SST2} & \textbf{1} & 4 & 2  & 6 & 5  & 3   \\
 \cmidrule(r){1-1}   \cmidrule(r){2-7} 

 ResNet34 \\
\it{CIFAR10} & 5 & 6 & 2 & \textbf{1}  & 3 & 4   \\
\it{CIFAR100} & 6 & 4& \textbf{1} & 5 & 2  & 3  \\
 ResNet50 \\
\it{ImageNet} & 3 & 5 & 6 & 4 & \textbf{1} & 2   \\
 \cmidrule(r){1-1}   \cmidrule(r){2-7} 
% \it{electric} & 0.6452 & 0.4640 & 0.6670  & 0.4693 & \textbf{0.678} & 0.5210    \\
% \it{pol} & \textbf{0.9914} & 0.9897 & 0.9826  & 0.9701 & 0.9826 & 0.9651    \\
% \it{covertype} & \textbf{0.6443} & 0.6406 & 0.6343 & 0.6151 & 0.6343 & 0.6231   \\
%  \cmidrule(r){1-1}   \cmidrule(r){2-7} 

average & 3.57 & 4.86 & 2.42 & 4.43 & \textbf{2.14} & 3.28    \\
    \bottomrule
  \end{tabular}
\end{table*}

\begin{table*}
  \centering
  \caption{Ranking of final losses, for all datasets and optimization methods. Best performing optimization method is marked in \textbf{bold}. }
  \label{Fig:lossranking}
  \begin{tabular}{c cccccc}
    \toprule
 & ADAM & SGD & ADAM  & SGD  & ADAM  & SGD  \\
 & - & - & SLS &  SLS &  SaLSa &  SaLSa \\
 \cmidrule(r){1-1}   \cmidrule(r){2-7} 
\it{MNLI} & 2 & 6 & 4  & 5 & \textbf{1} &  3  \\
\it{QNLI} & 2 & 5 & 3  & 6 & \textbf{1} & 4\\
\it{MRPC} & 3 & 4 & 2  & 6 & \textbf{1}  & 5  \\
\it{SST2} & \textbf{1} & 5 & 3 & 6 & 2 & 4  \\
GPT-2 & 2 & 6 & 3  & 5 & \textbf{1} & 4  \\
 \cmidrule(r){1-1}   \cmidrule(r){2-7} 
ResNet34\\
\it{CIFAR10} & 5 & 4 & \textbf{1} & 6 & 2  & 3  \\
\it{CIFAR100} & 5 & 2 & 3  & 6 & \textbf{1} & 4  \\
ResNet50\\
\it{ImageNet} & 2 & 4 & 6 & 5 & \textbf{1}  &  3 \\
 \cmidrule(r){1-1}   \cmidrule(r){2-7} 
%$MNIST$ & 0.00002213 & 0.001333 & 0.01695 & \textbf{0.00001173} & not converged & not converged \\
% \it{electric} & \textbf{0.4109} & 0.4632 & 0.4566  & 0.4921 & 0.4548 & 0.4771 \\
% \it{pol} & \textbf{0.00757} & 0.02302 & 0.02676 & 0.07148  & 0.02585 & 0.08677 \\
% \it{covertype} & 0.1554 & \textbf{0.1311} & 0.1488  & 0.2564 & 0.1697 & 0.2039 \\
%  \cmidrule(r){1-1}   \cmidrule(r){2-7} 

average & 2.75 & 4.625 & 3.125  & 5.5 & \textbf{1.25} & 3.75 \\
    \bottomrule
  \end{tabular}
\end{table*}

% \begin{figure}[h!]

% \subfloat[Electric]{\includegraphics[width = 0.33\textwidth]{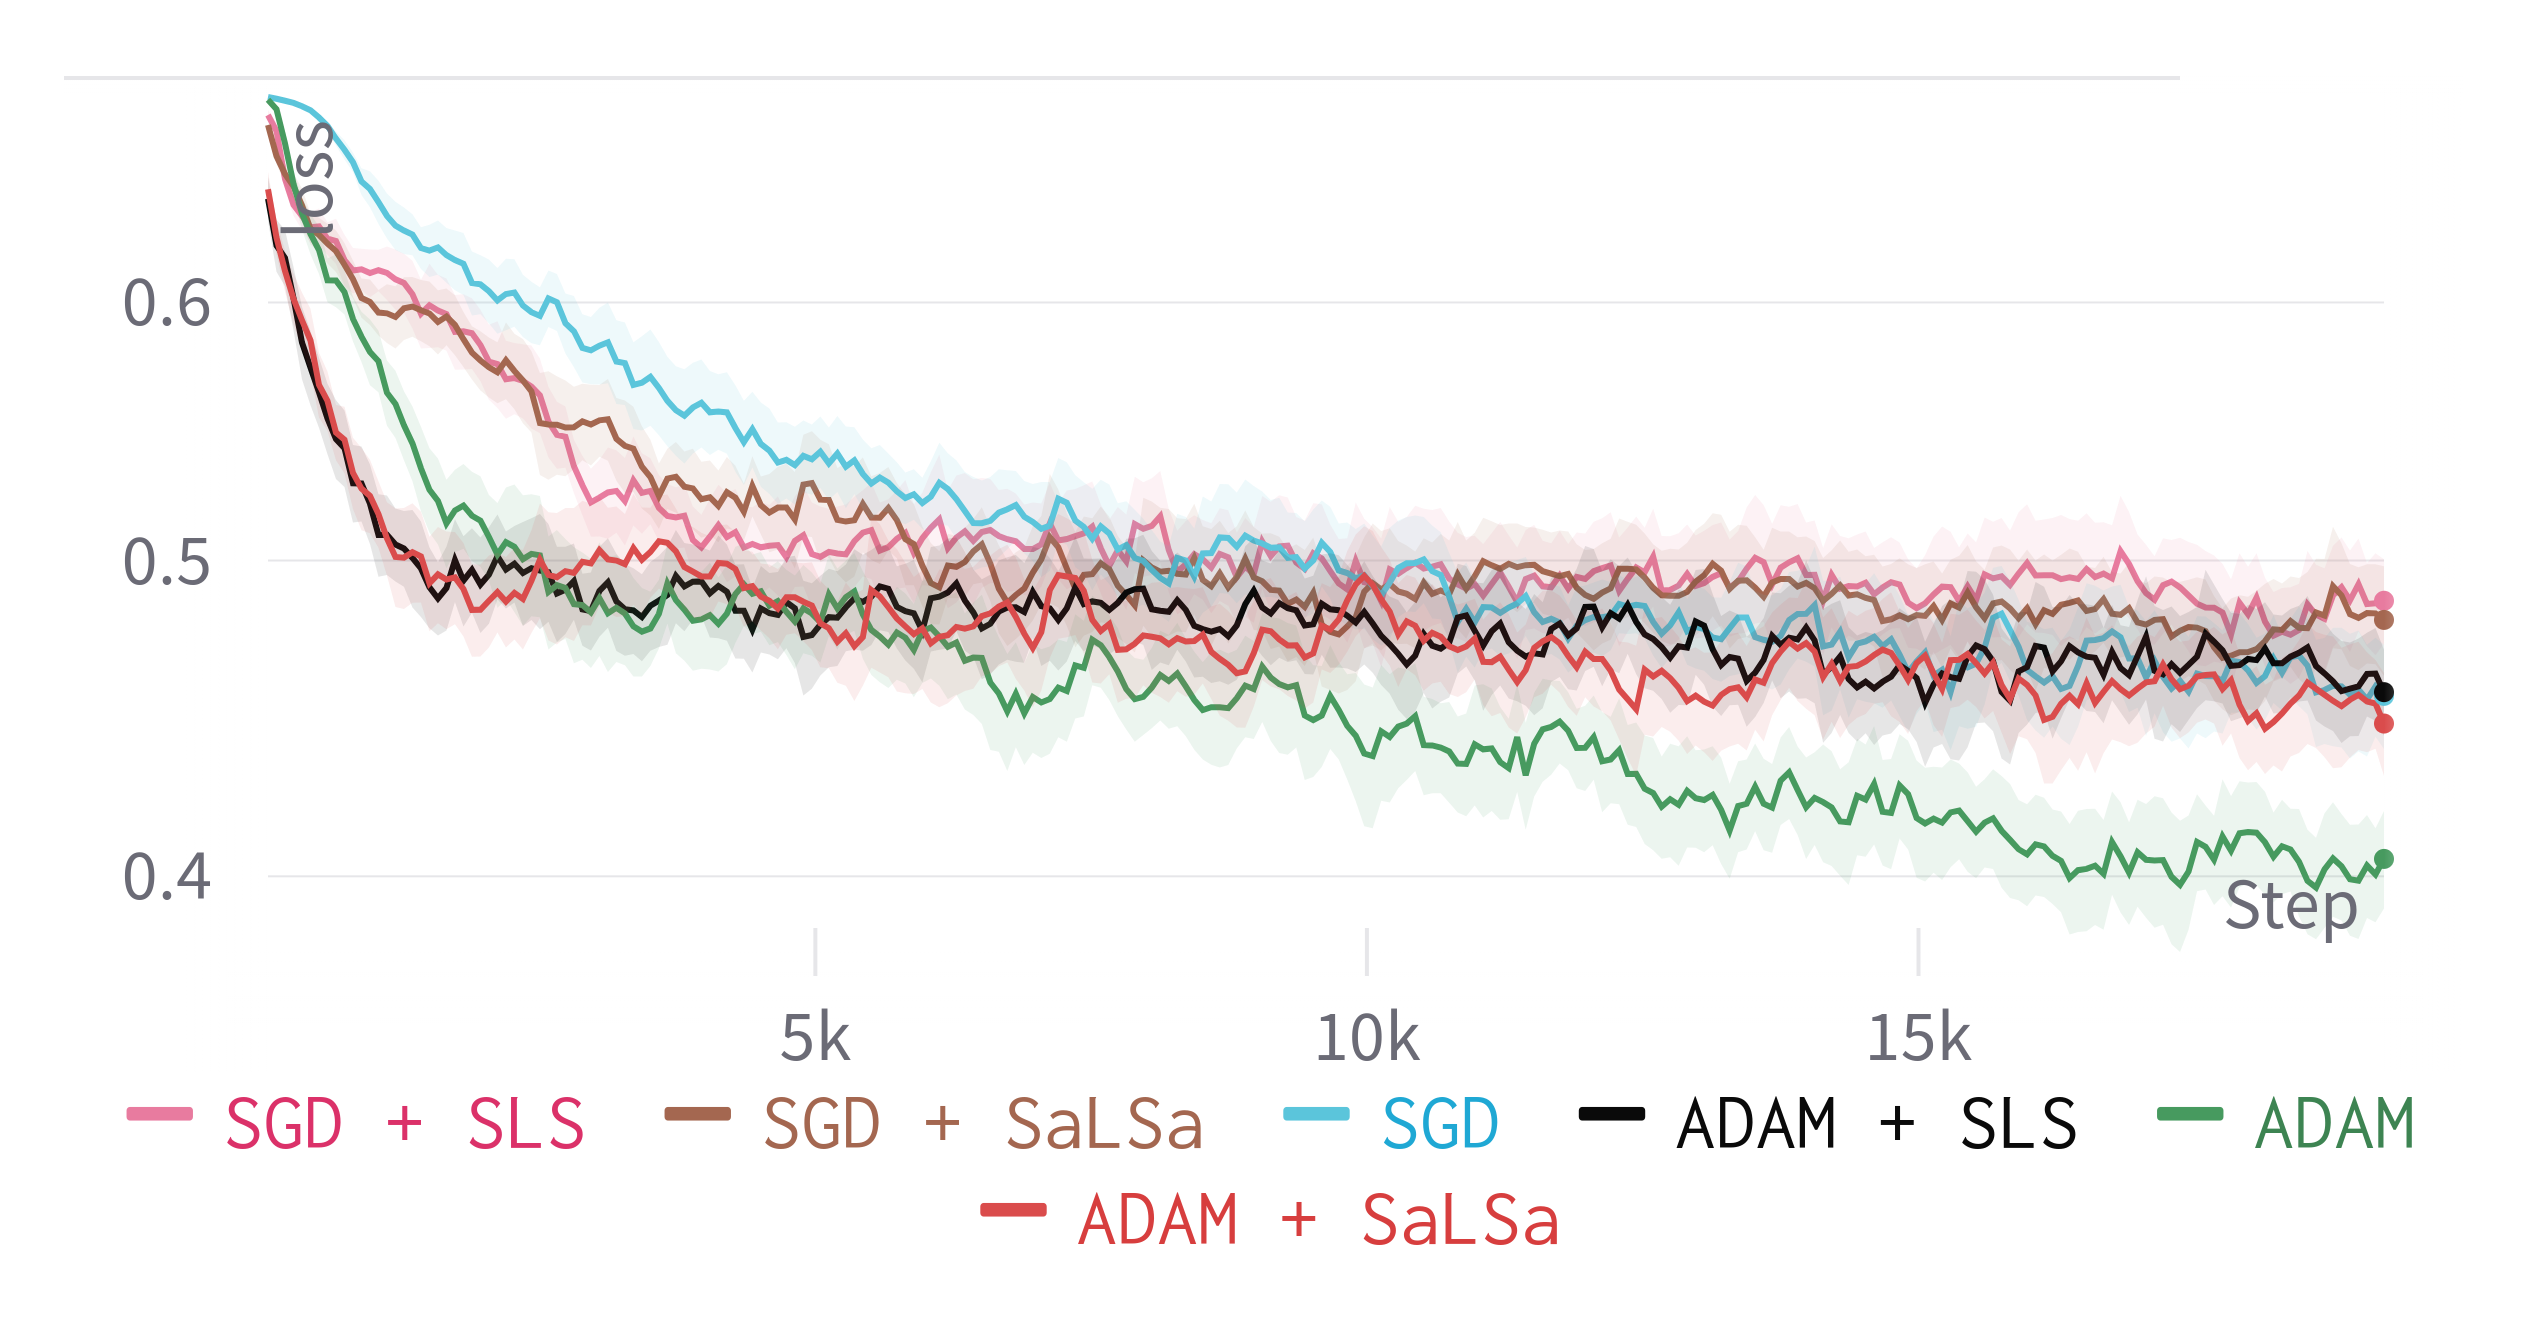}}
% \subfloat[Pol]{\includegraphics[width = 0.33\textwidth]{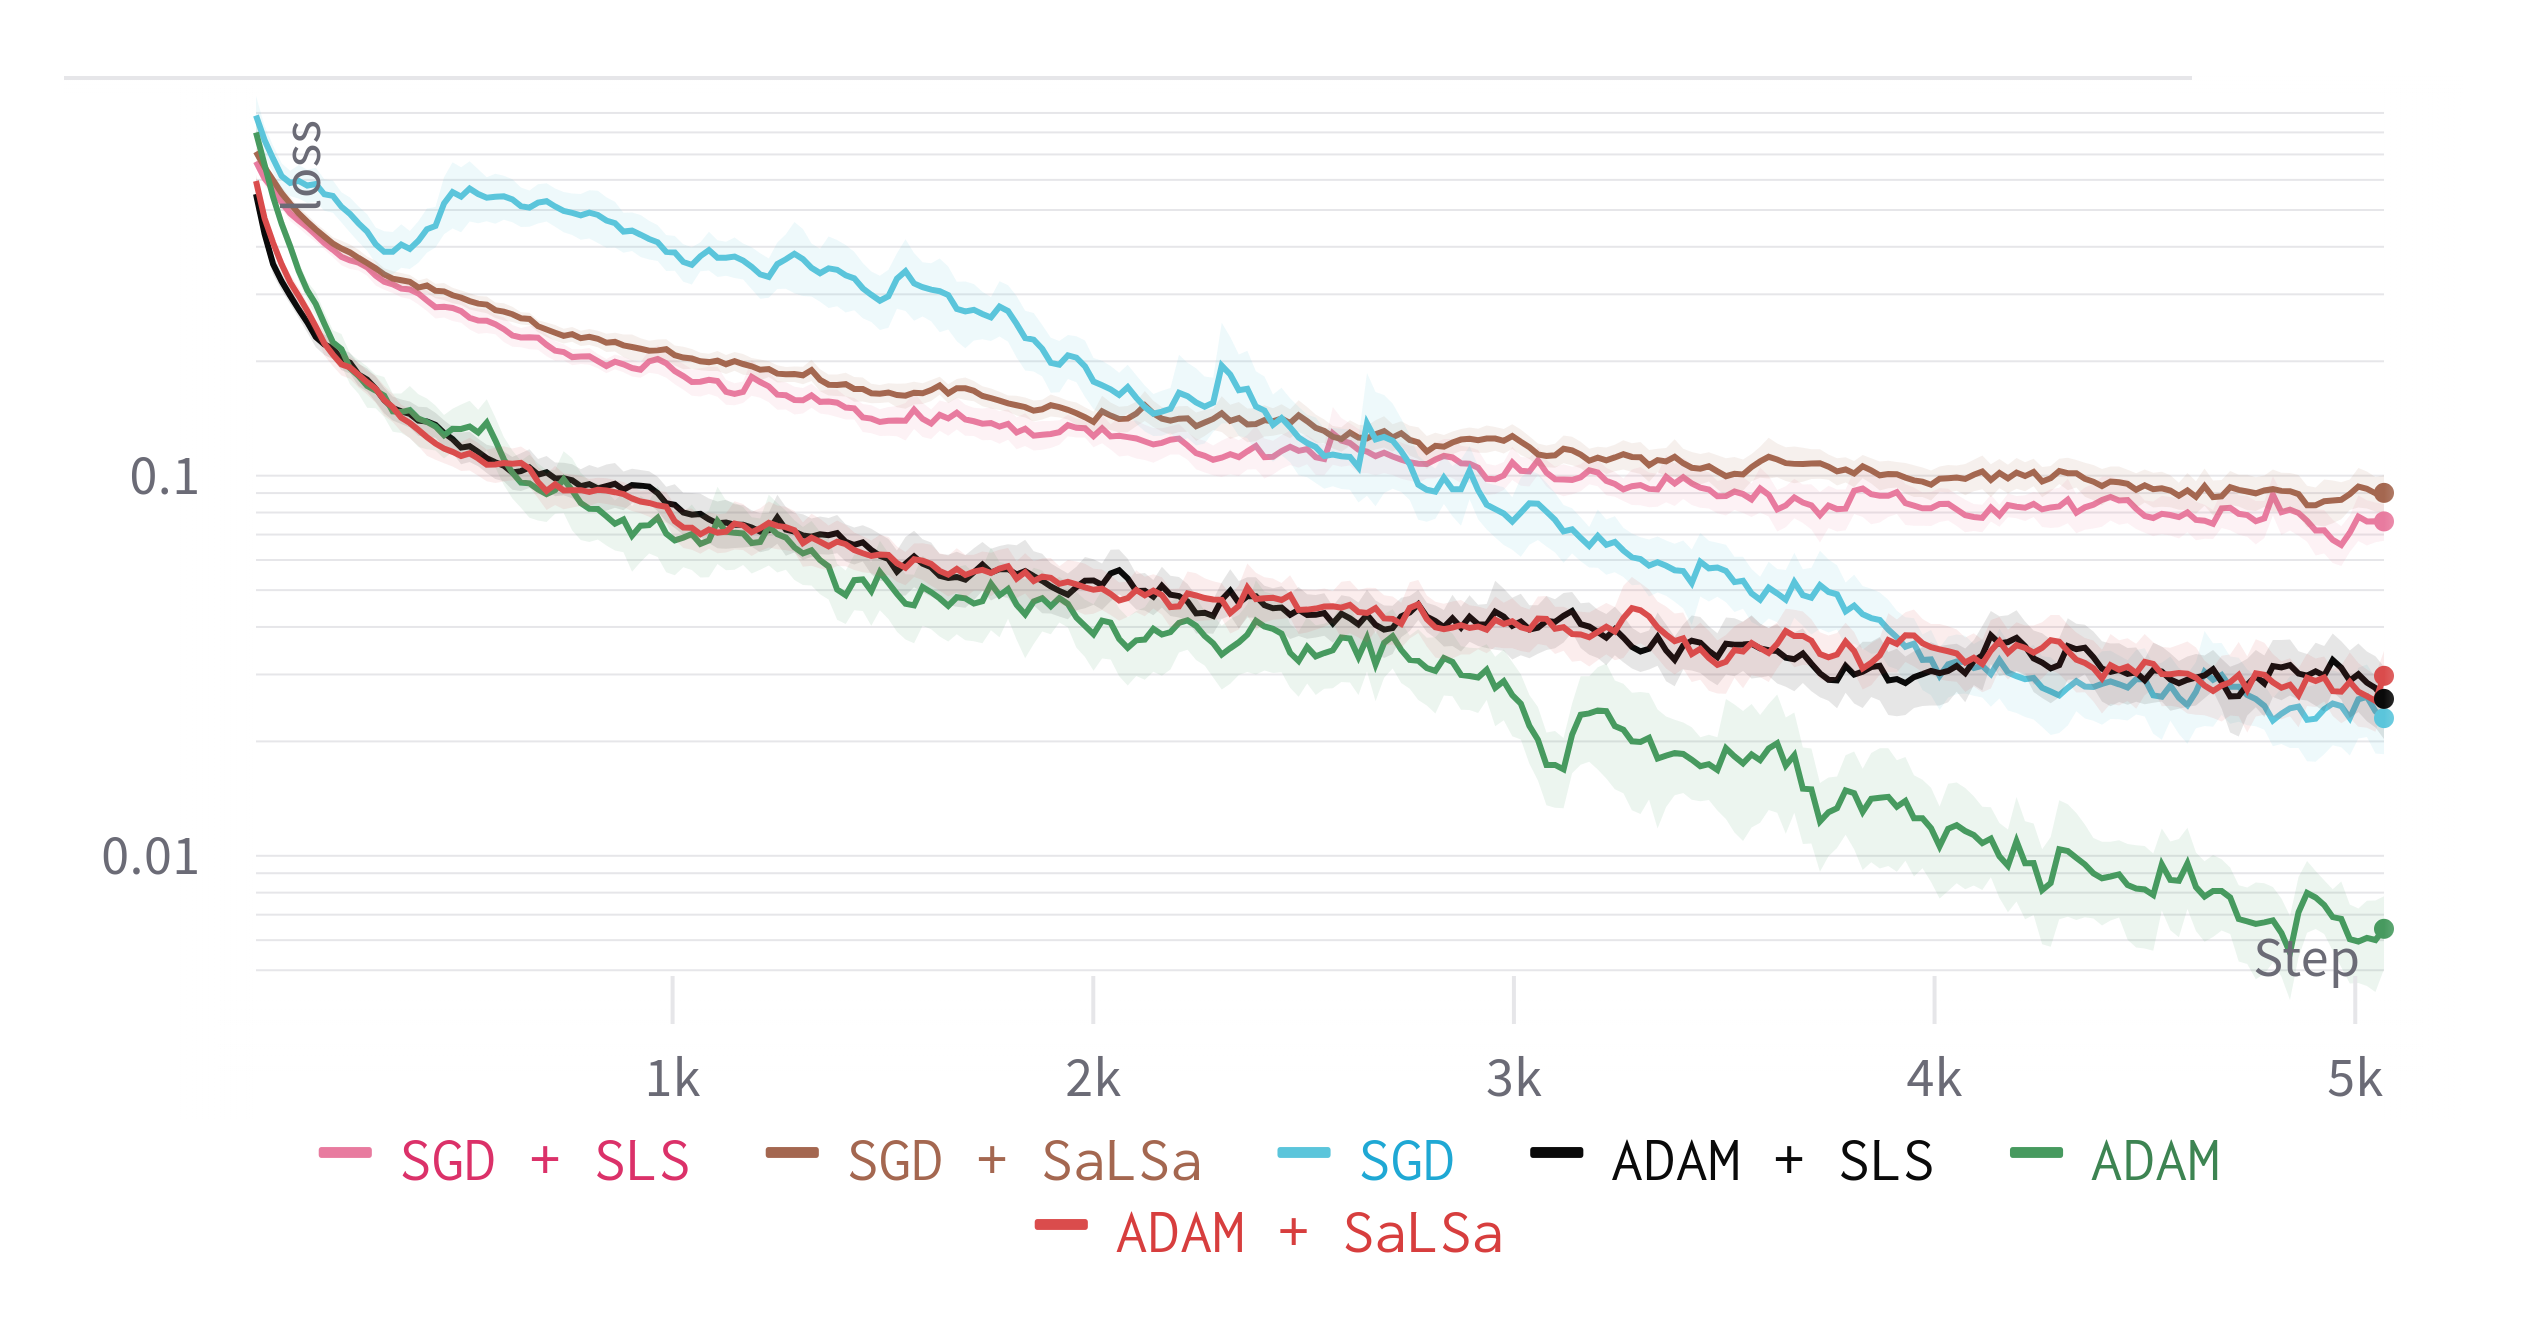}}
% \subfloat[Covertype]{\includegraphics[width = 0.33\textwidth]{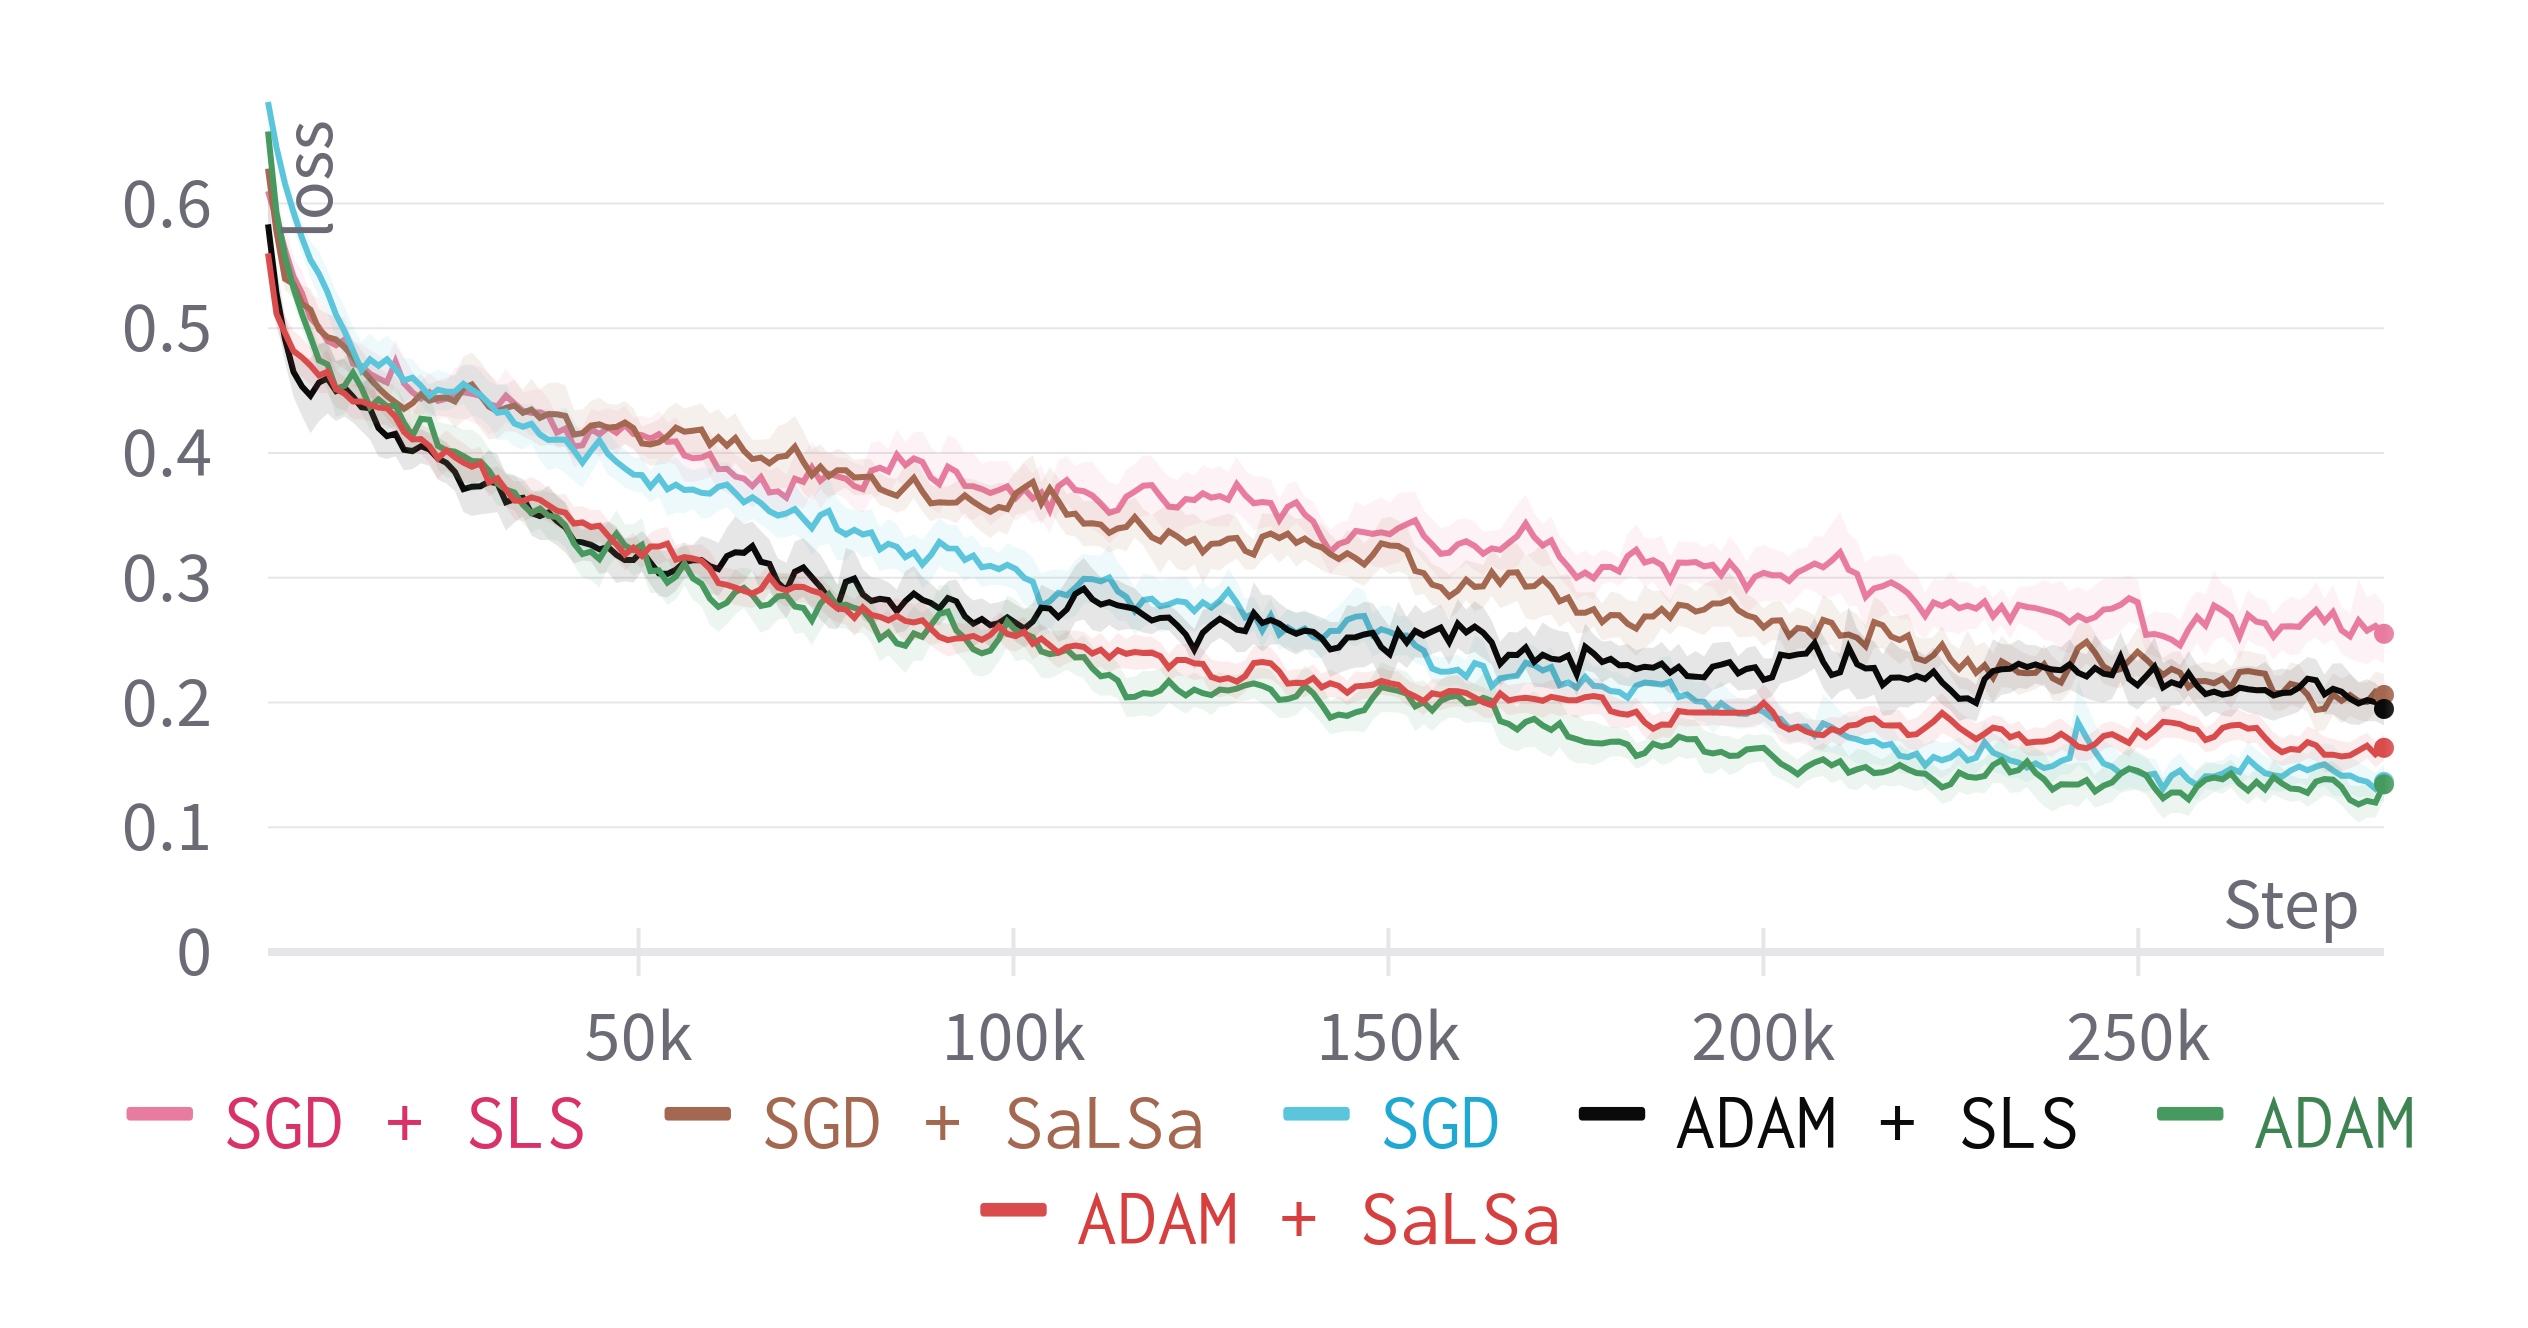}}
%  \\
% \subfloat[Electric]{\includegraphics[width = 0.33\textwidth]{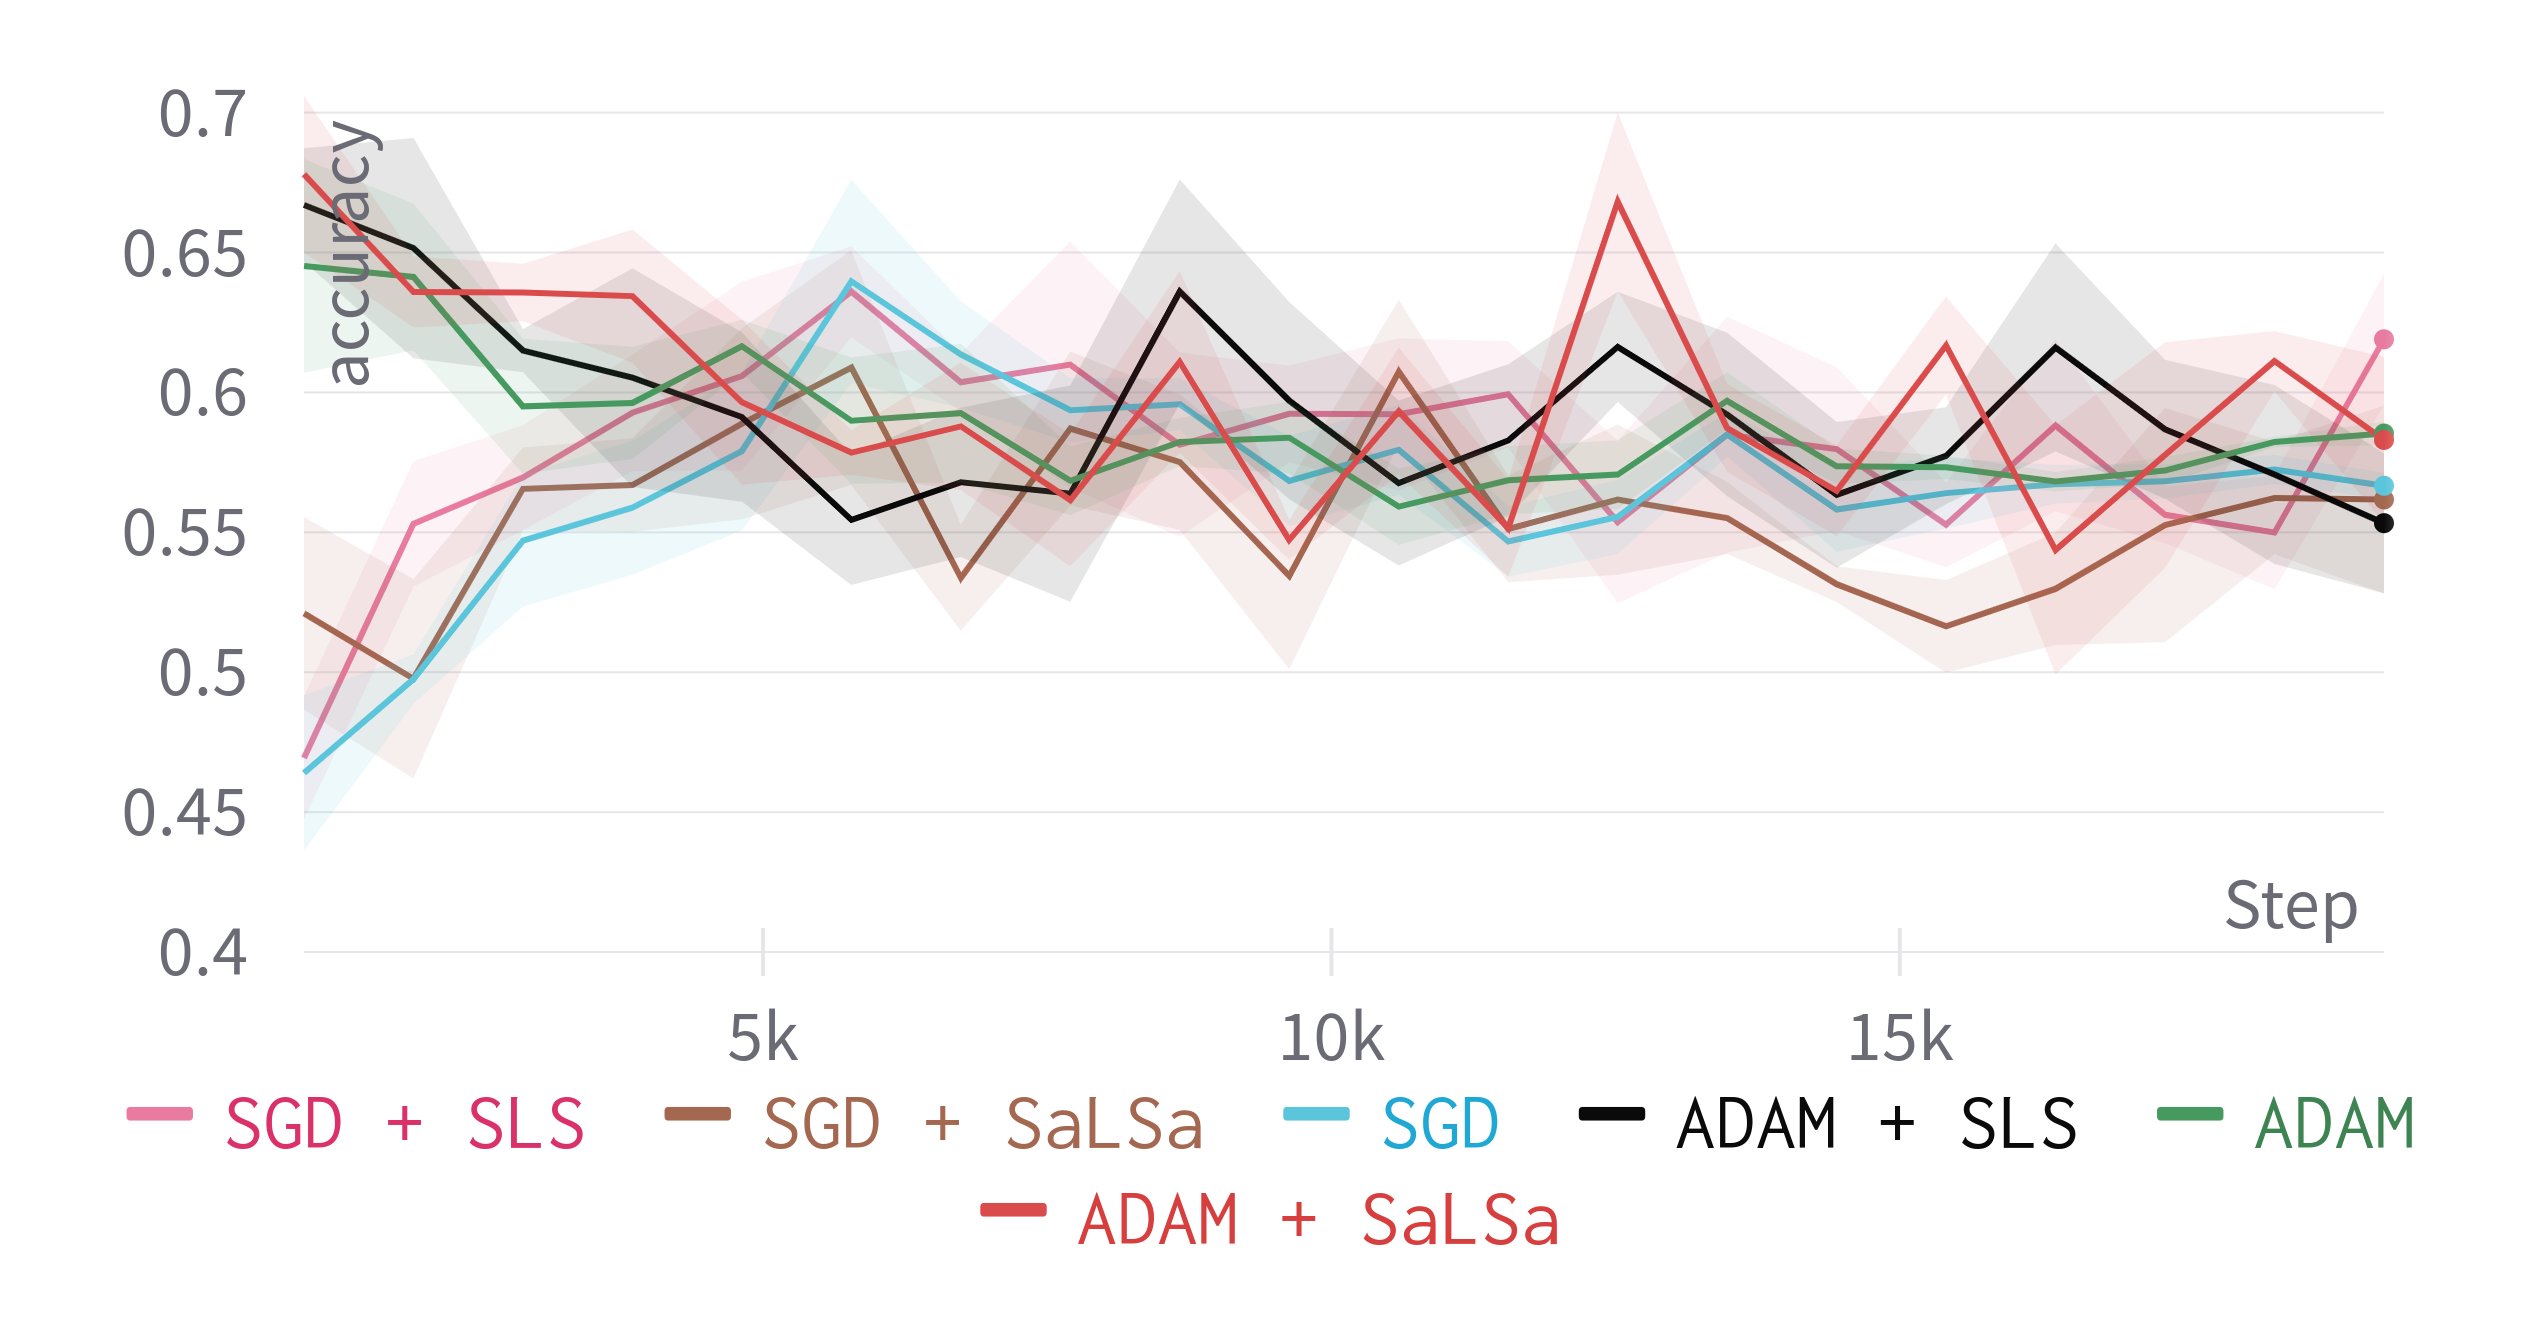}} 
% \subfloat[Pol]{\includegraphics[width = 0.33\textwidth]{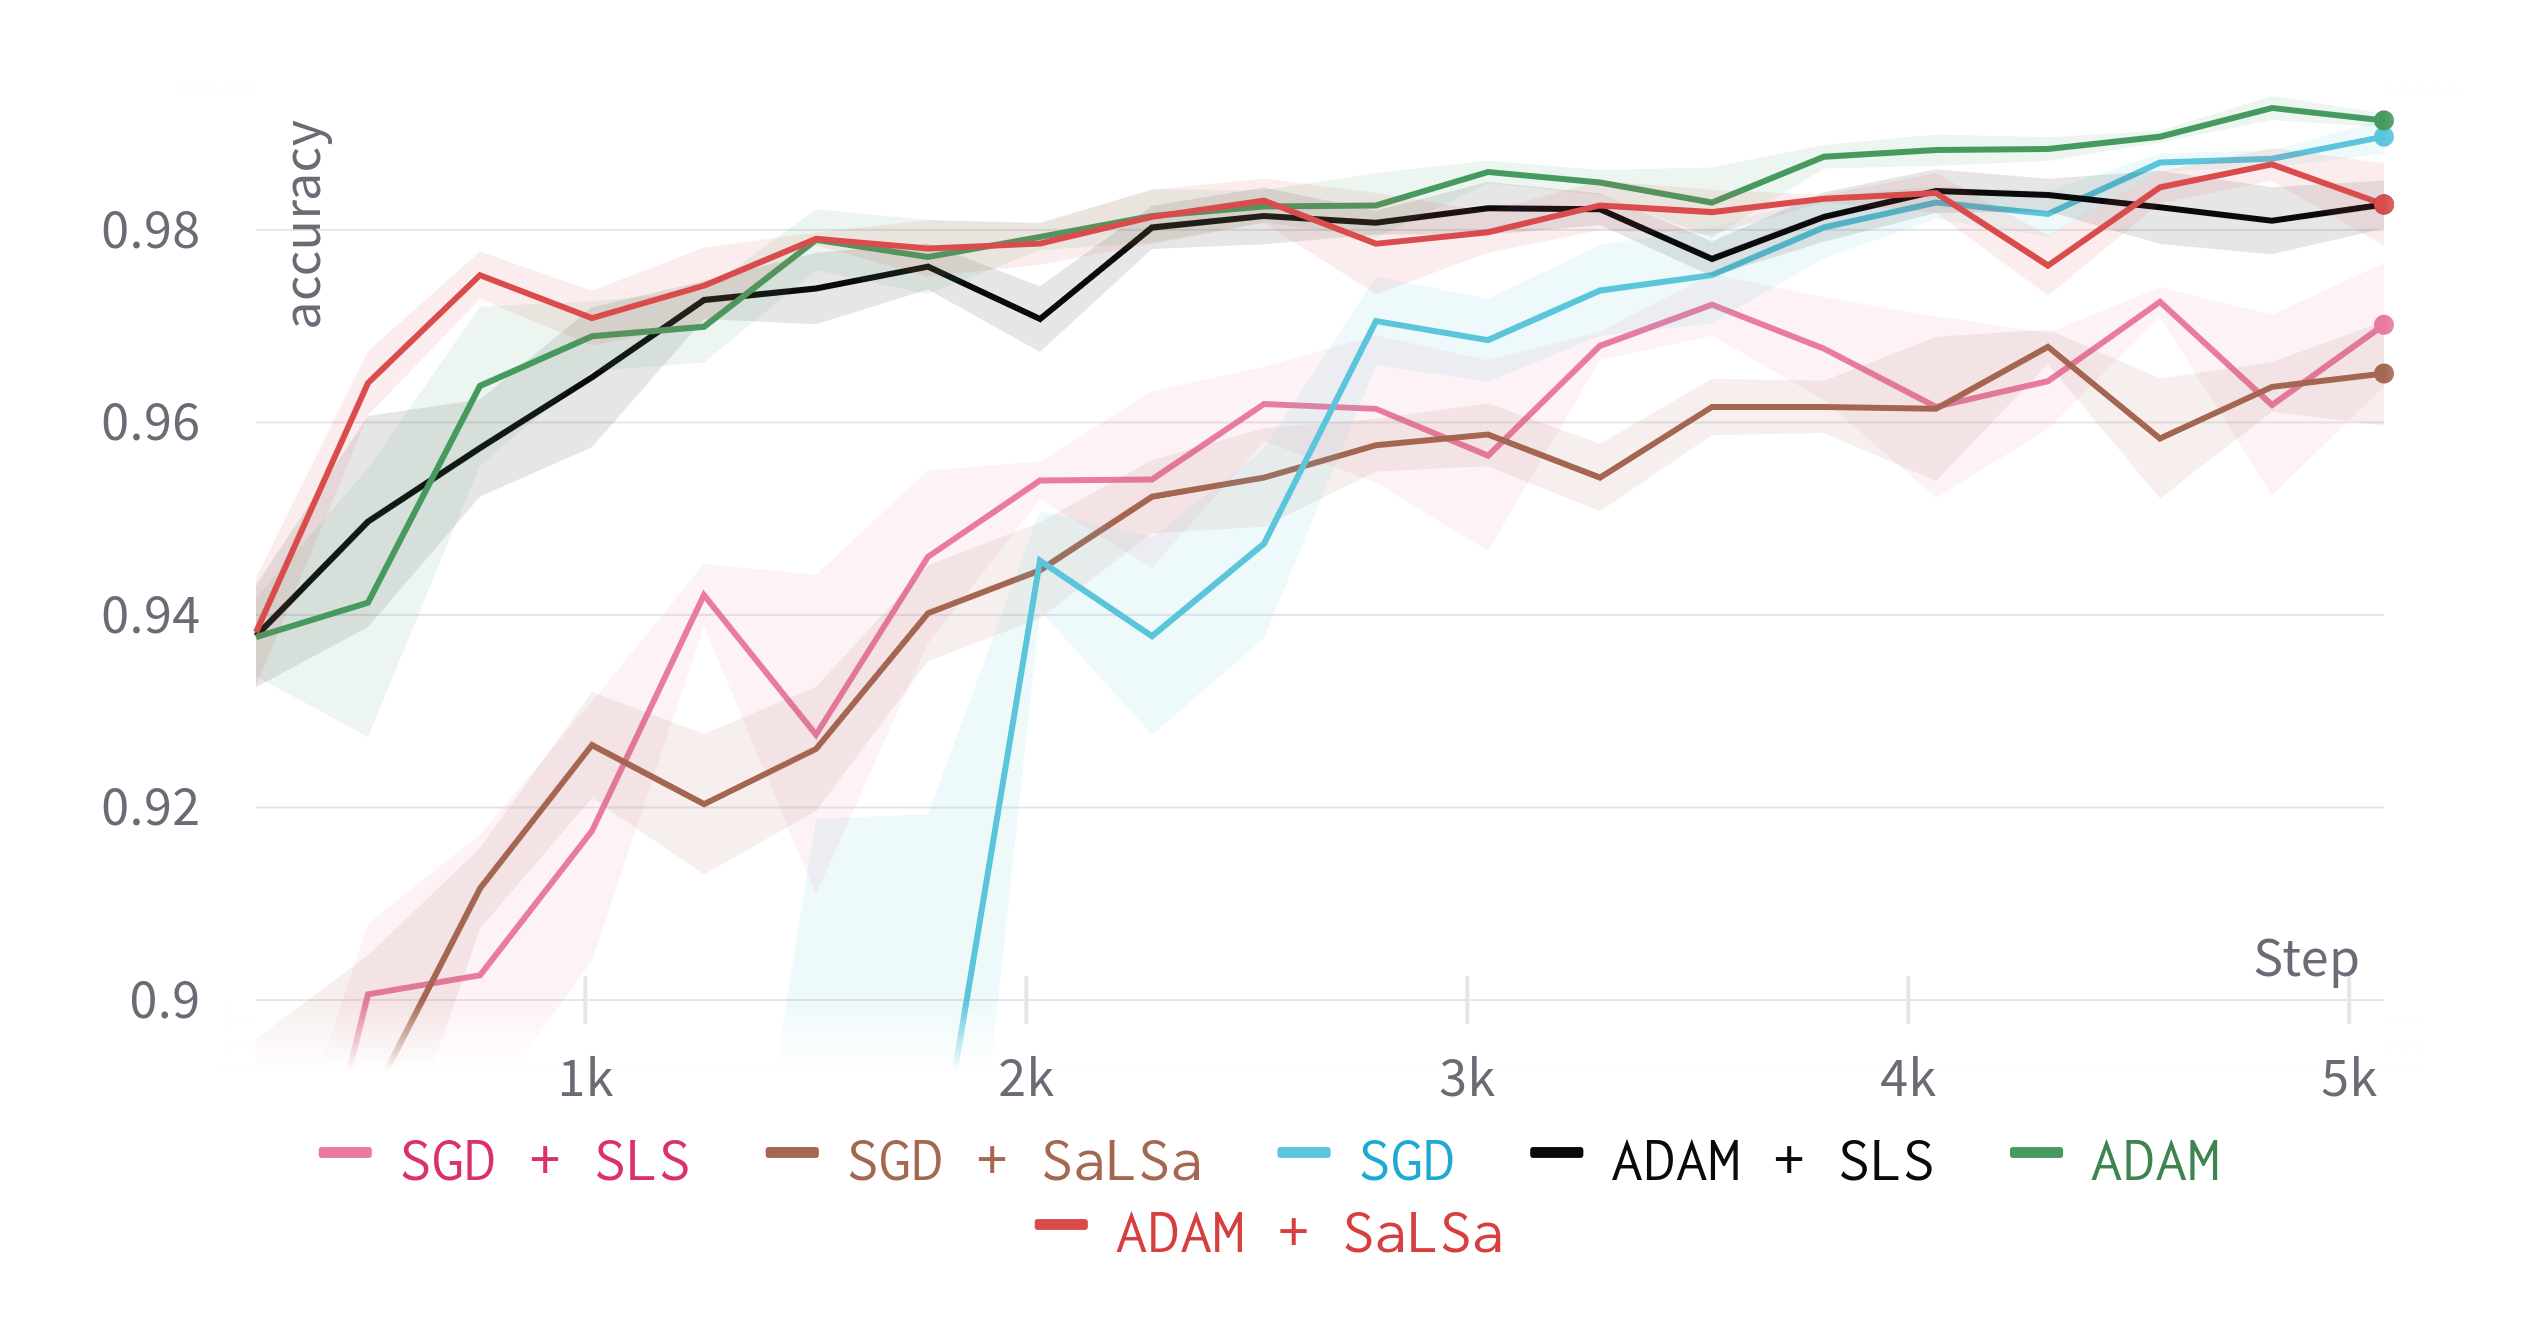}} 
% \subfloat[Covertype]{\includegraphics[width = 0.33\textwidth]{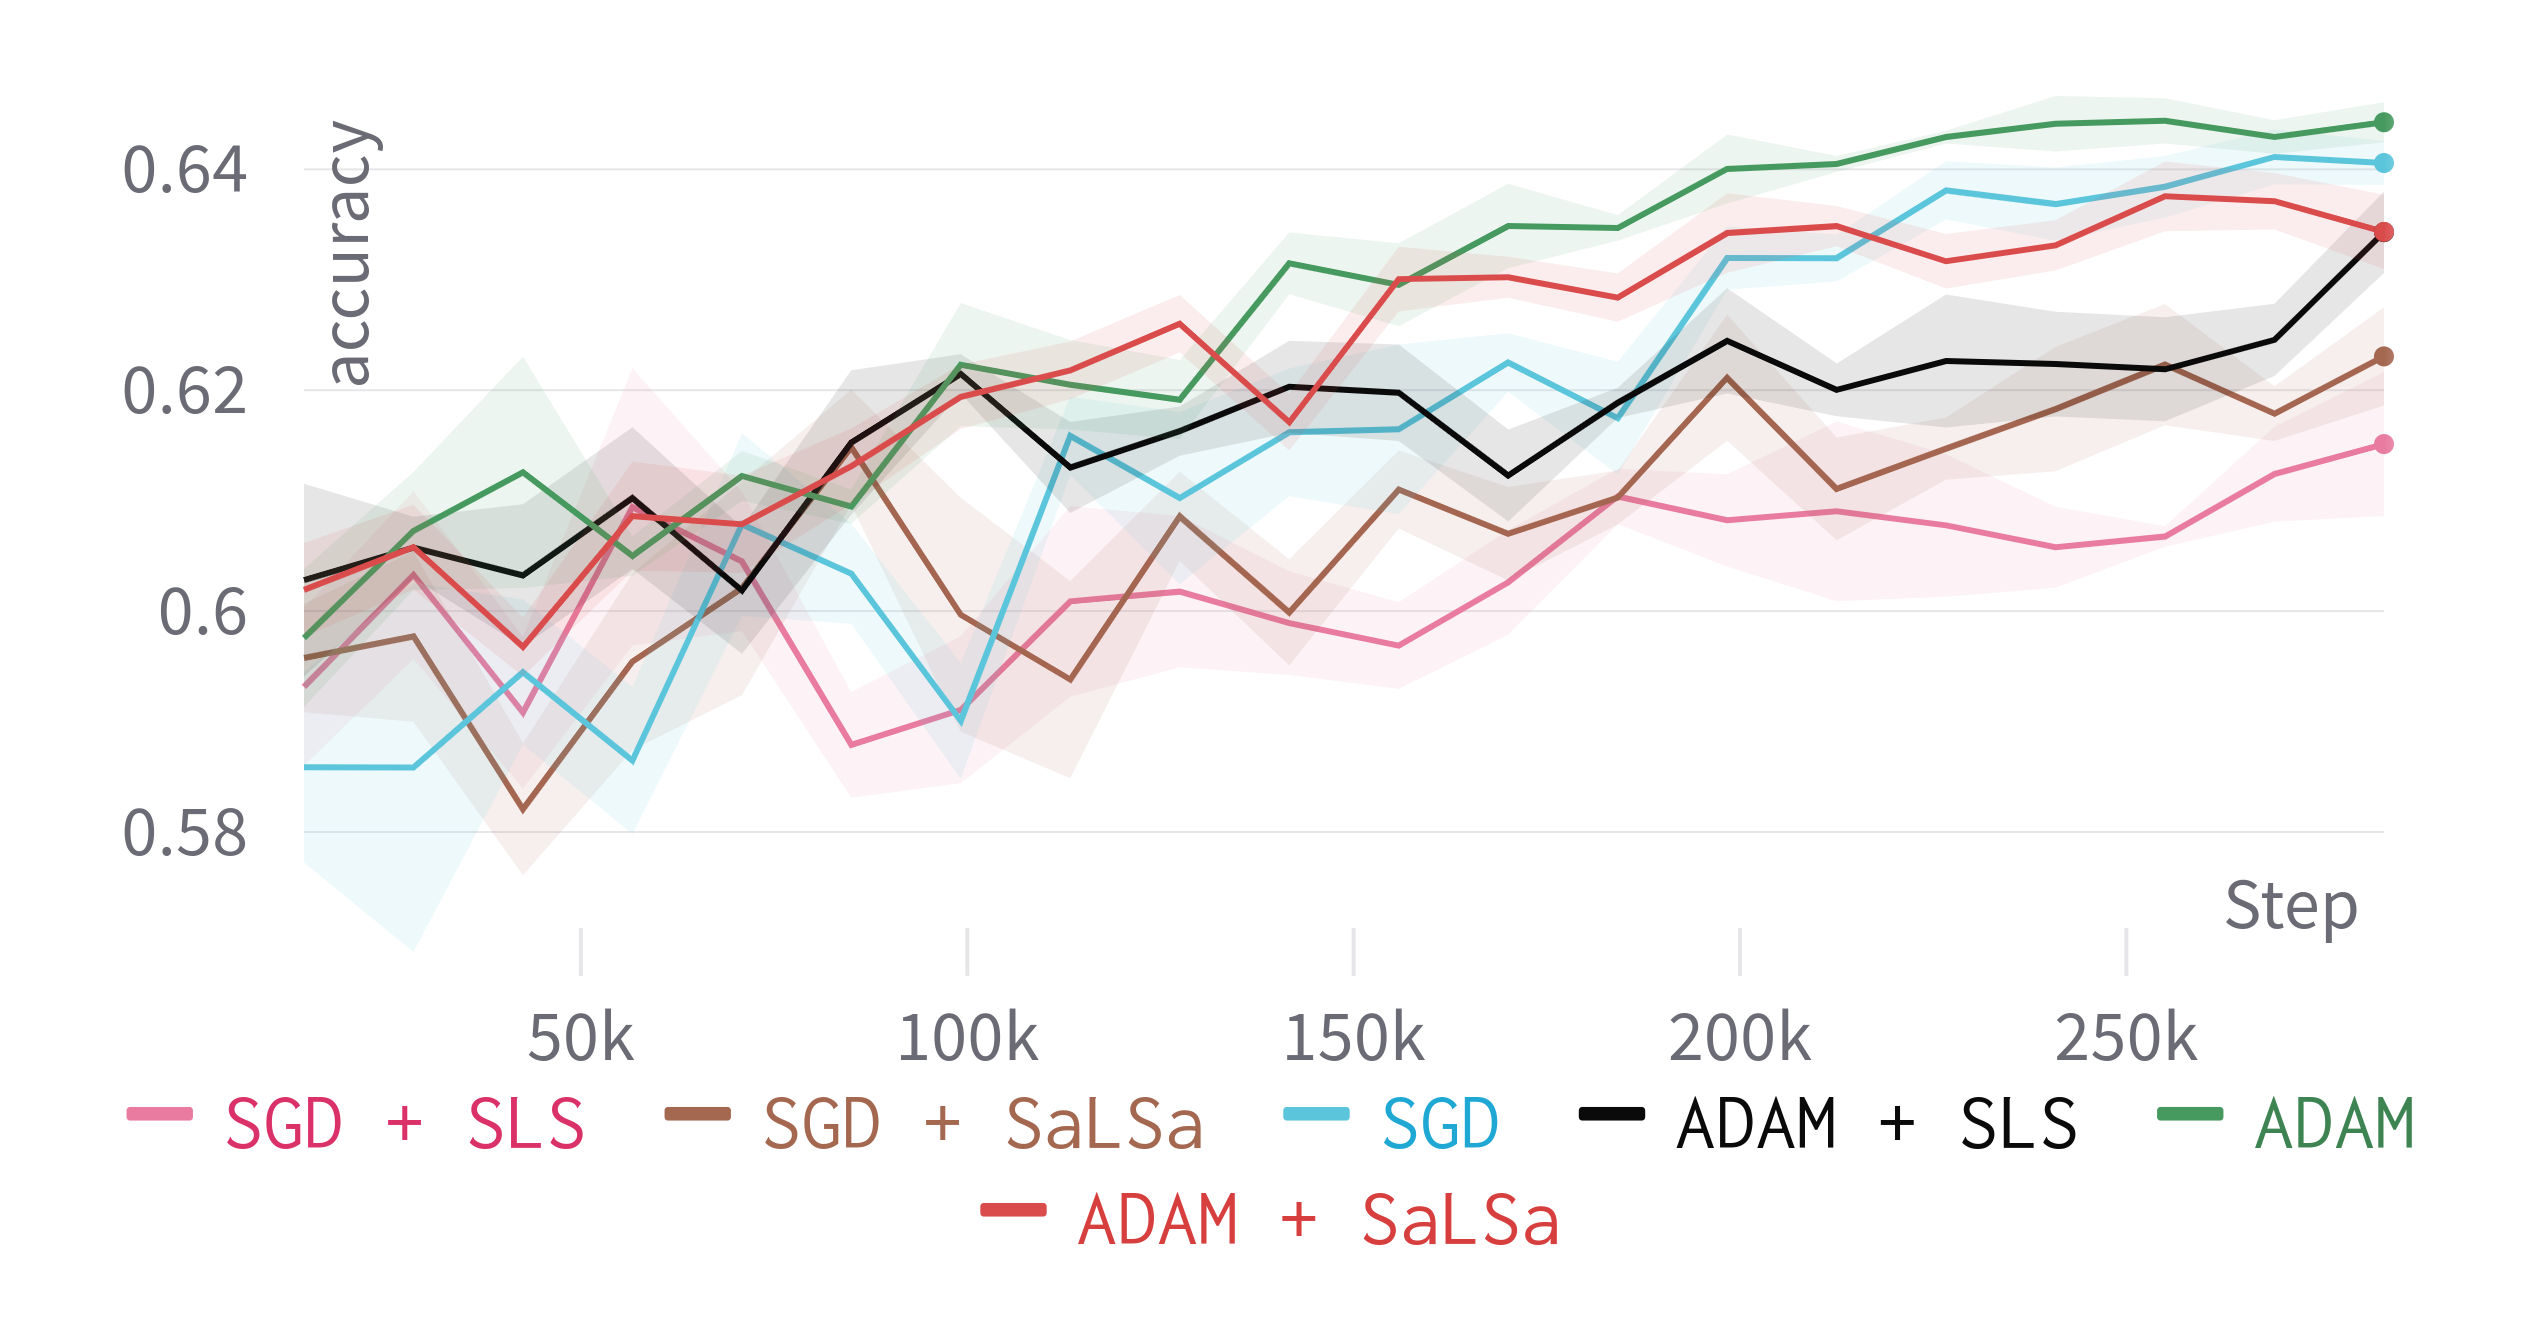}} 

% \caption{The loss (top row) and accuracy curves (bottom row) of the Tabular experiments with standard error indicated around each line, starting after the first epoch. Accuracy was calculated on the validation data, while loss was calculated on the training data.}
% \label{fig:tabular}
% \end{figure}

\begin{figure}[h!]
\subfloat[GPT-2]{\includegraphics[width = 0.33\textwidth]{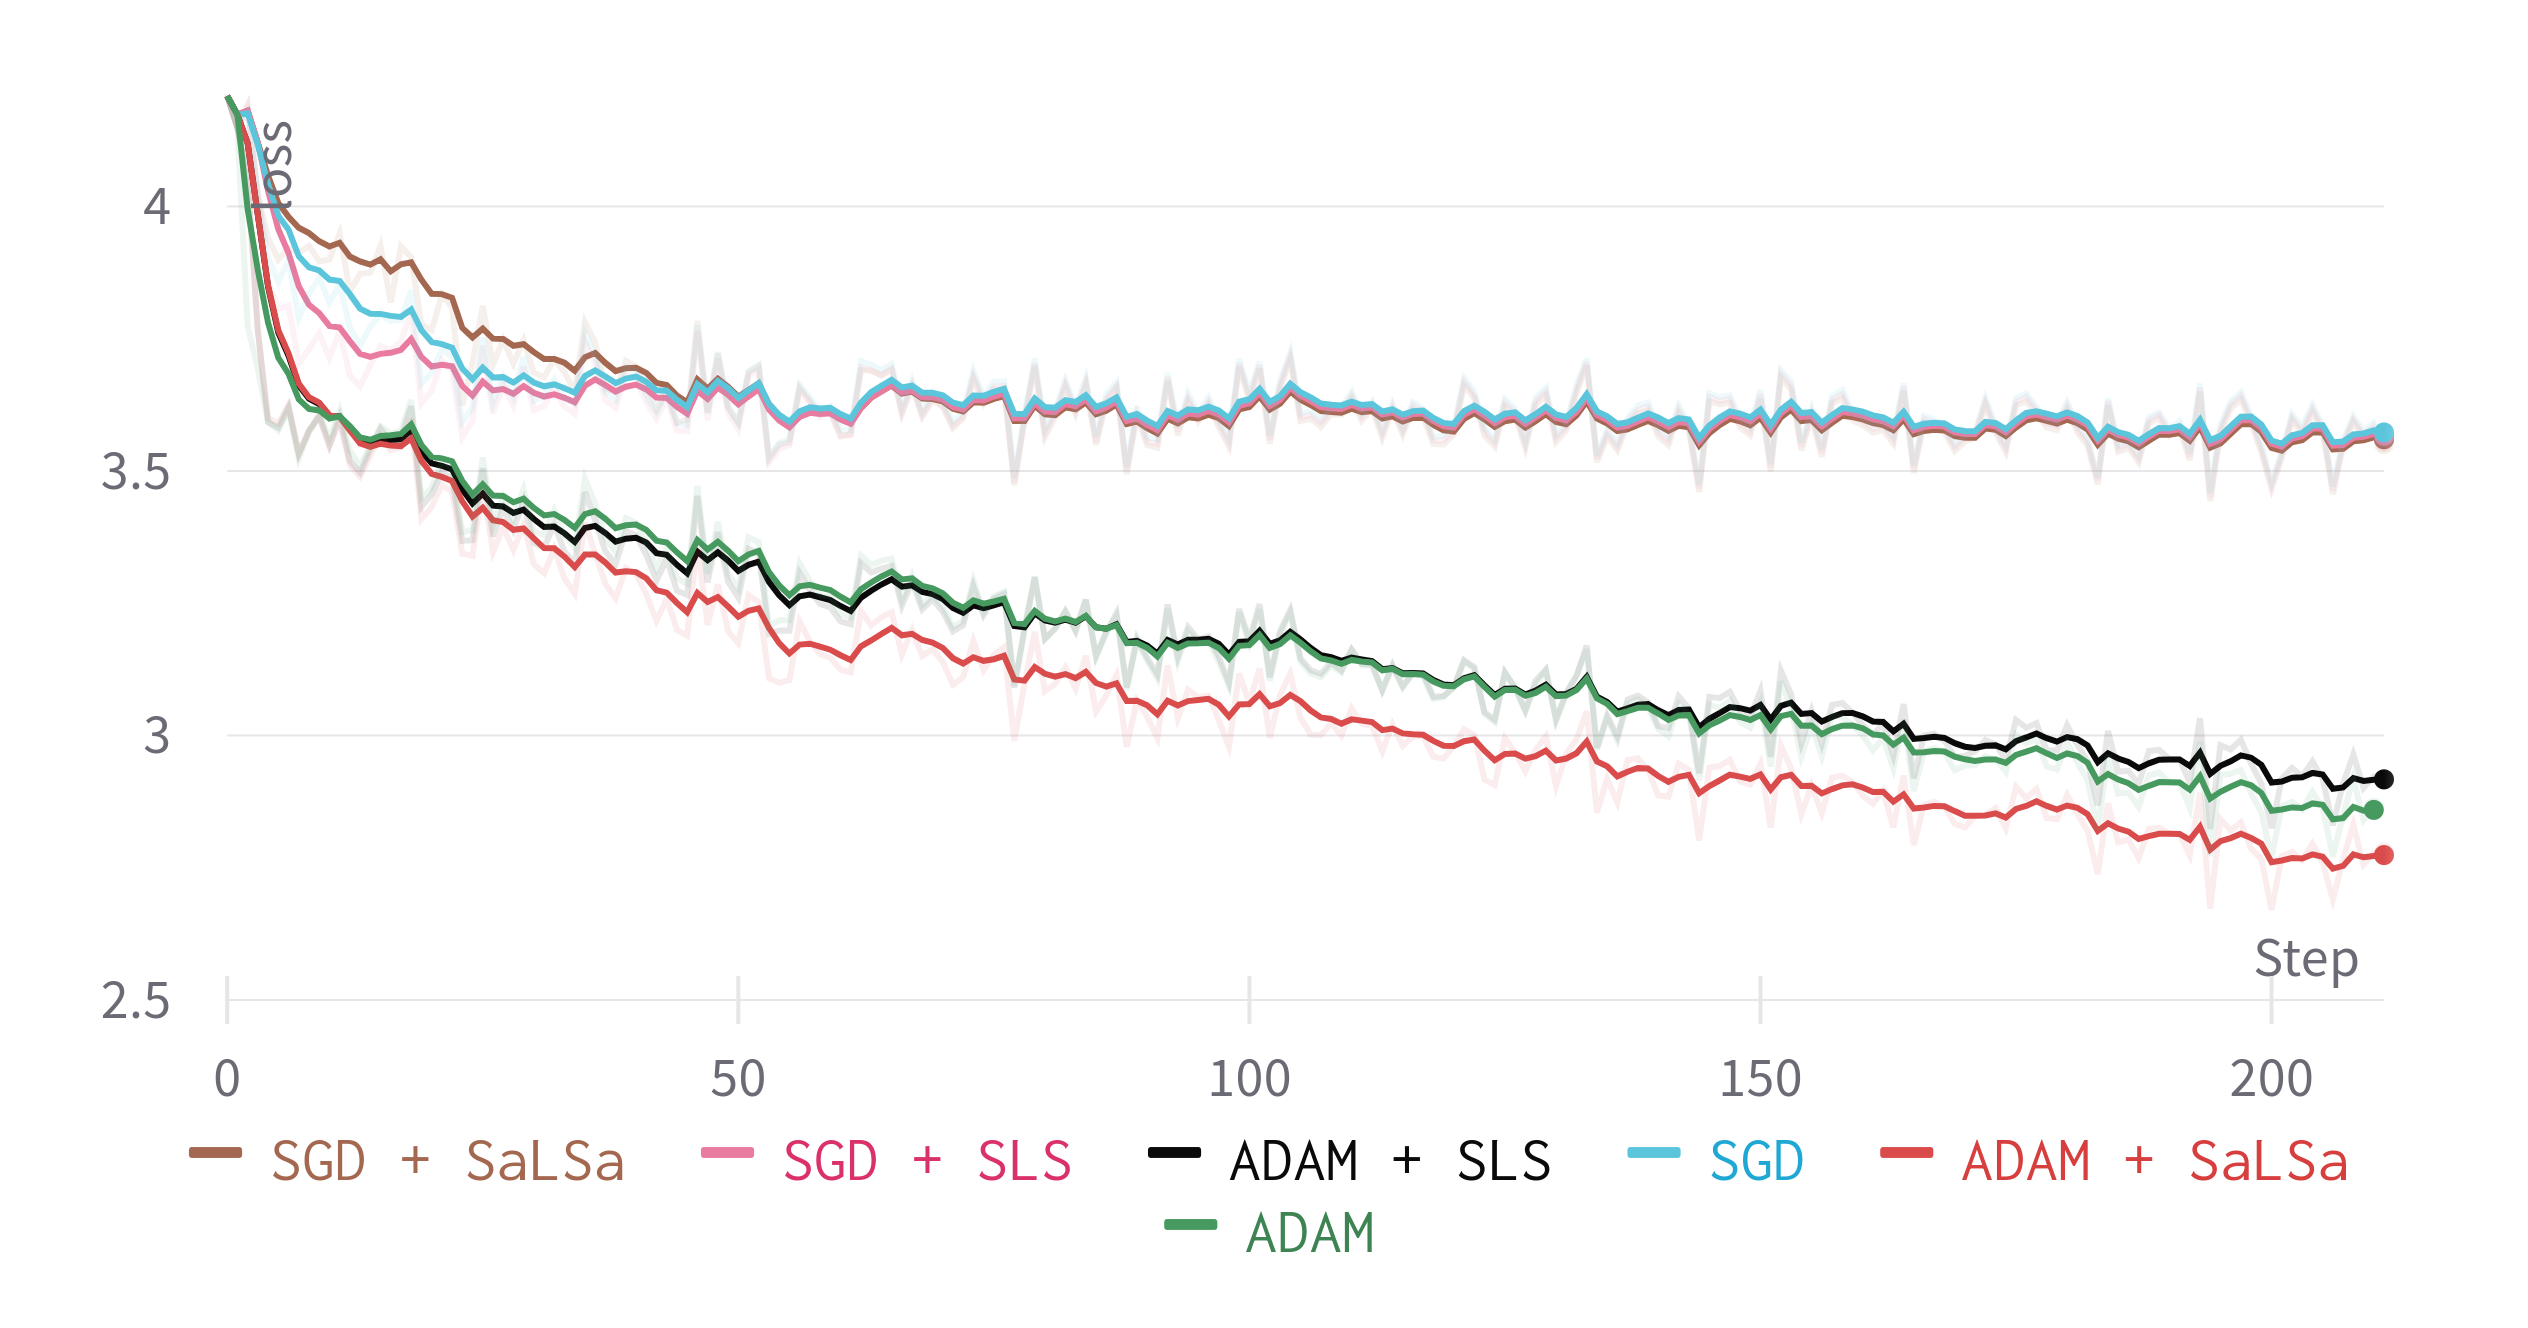}}
\subfloat[SST2 loss]{\includegraphics[width = 0.33\textwidth]{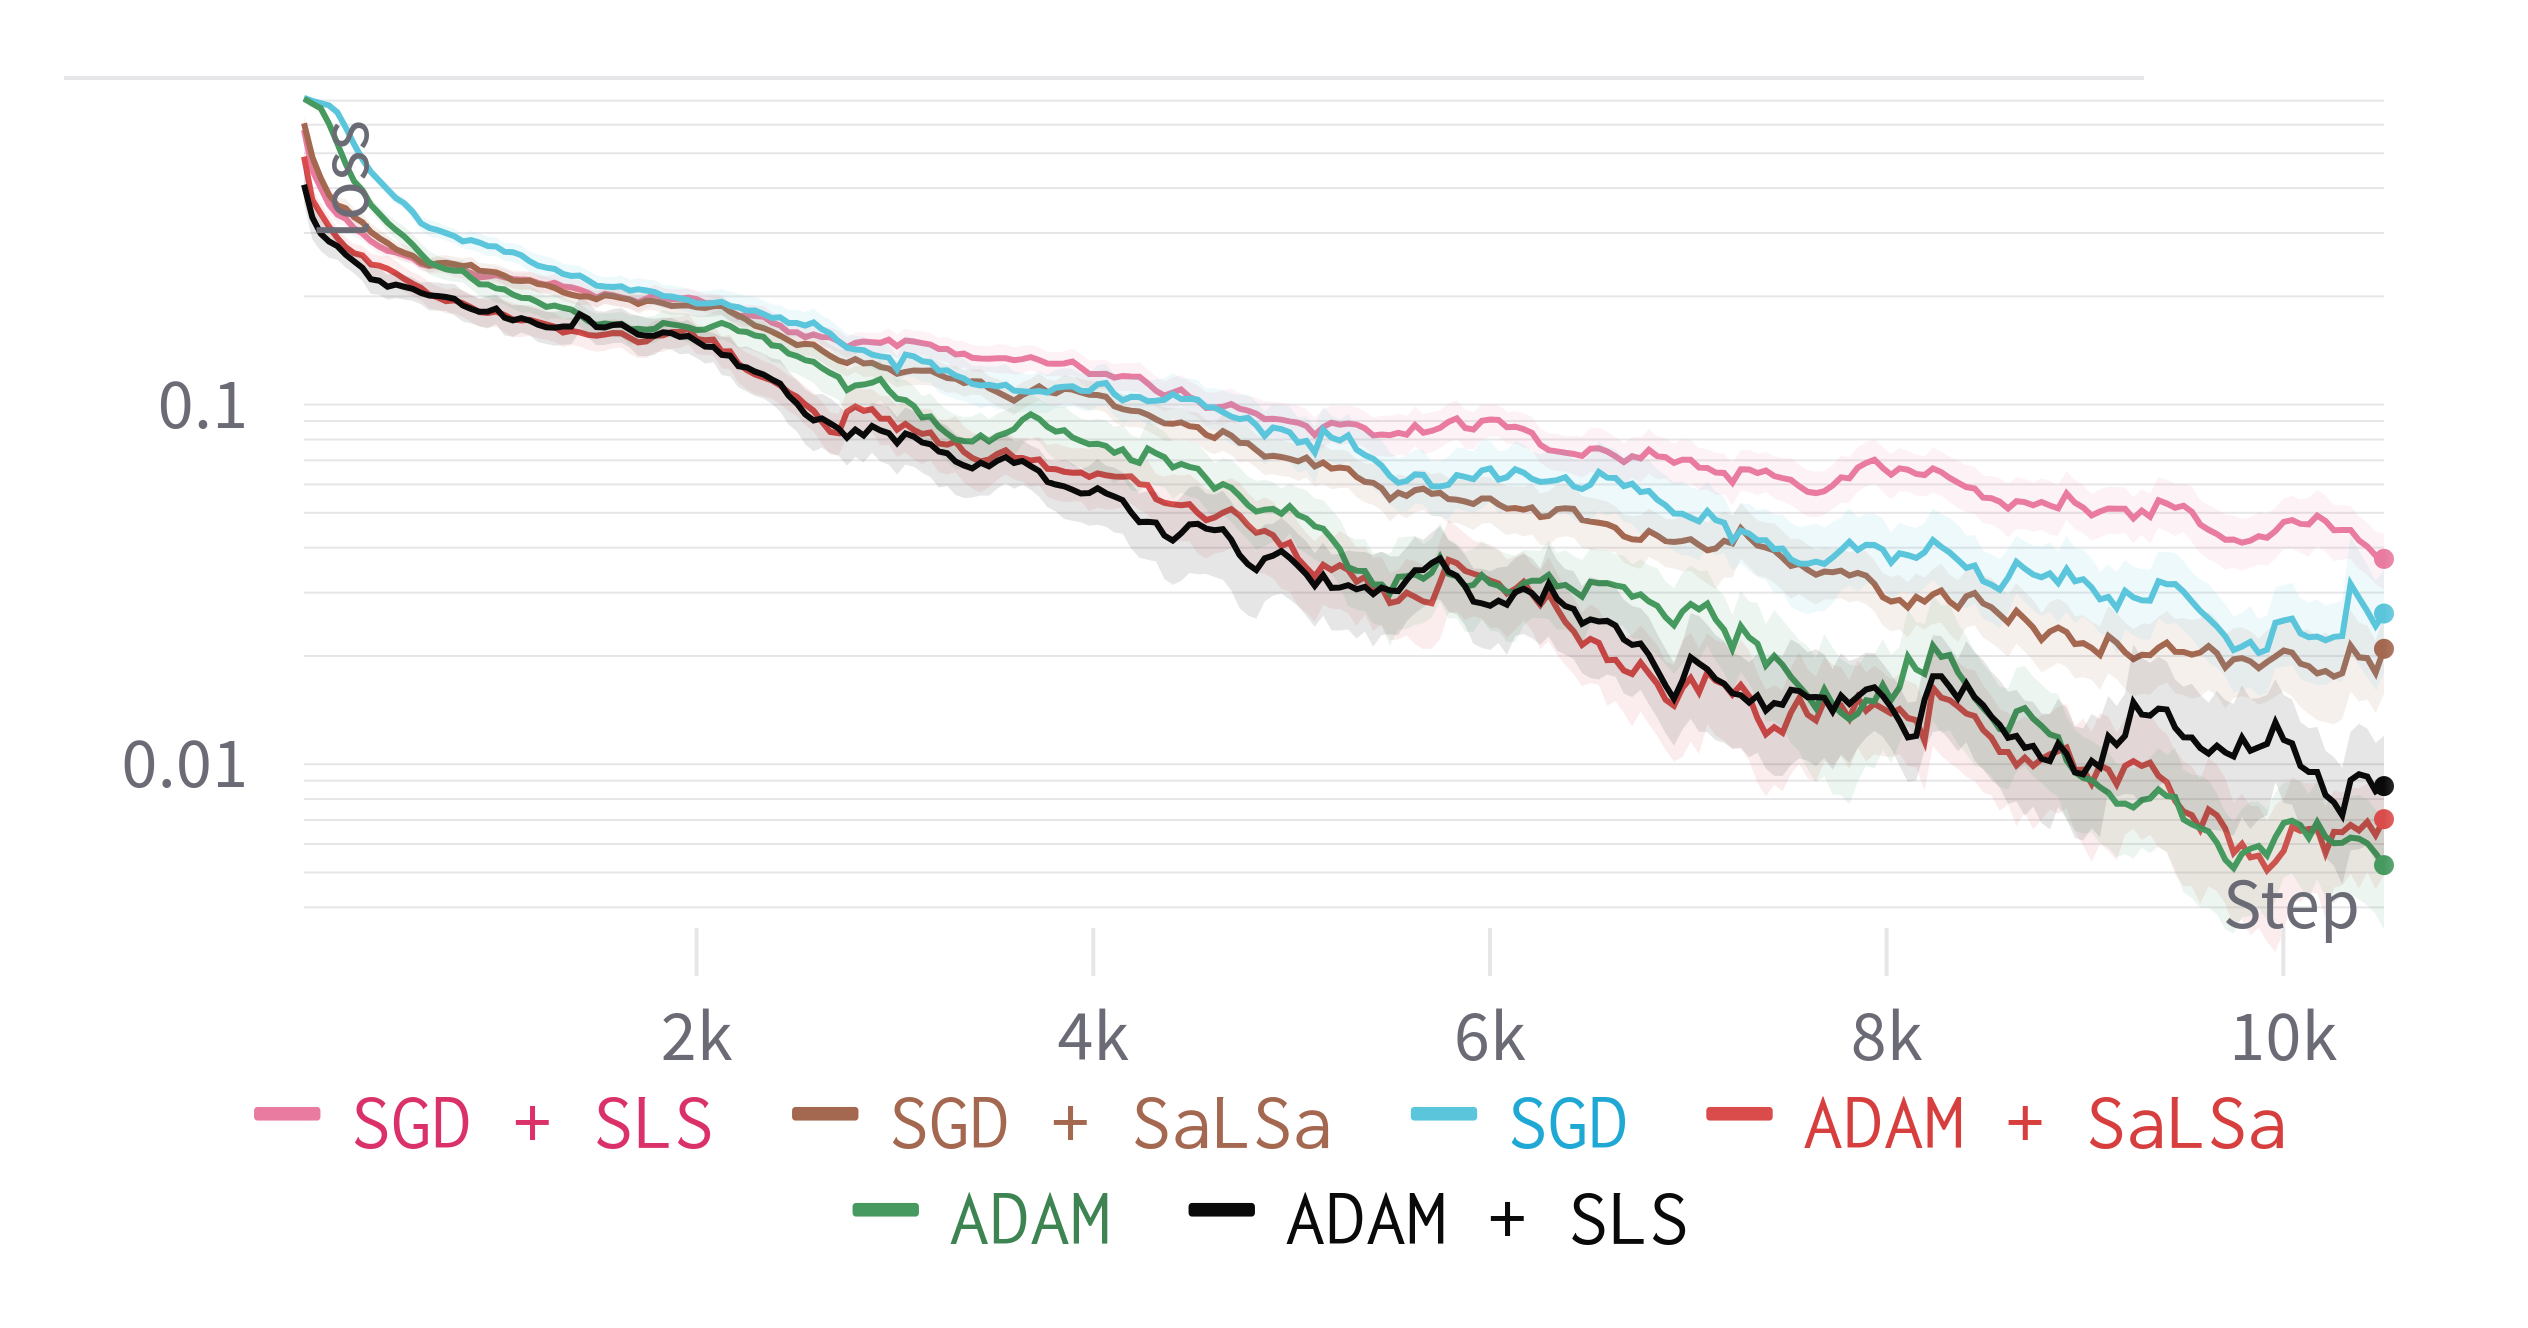}} 
\subfloat[SST2 accuracy]{\includegraphics[width = 0.33\textwidth]{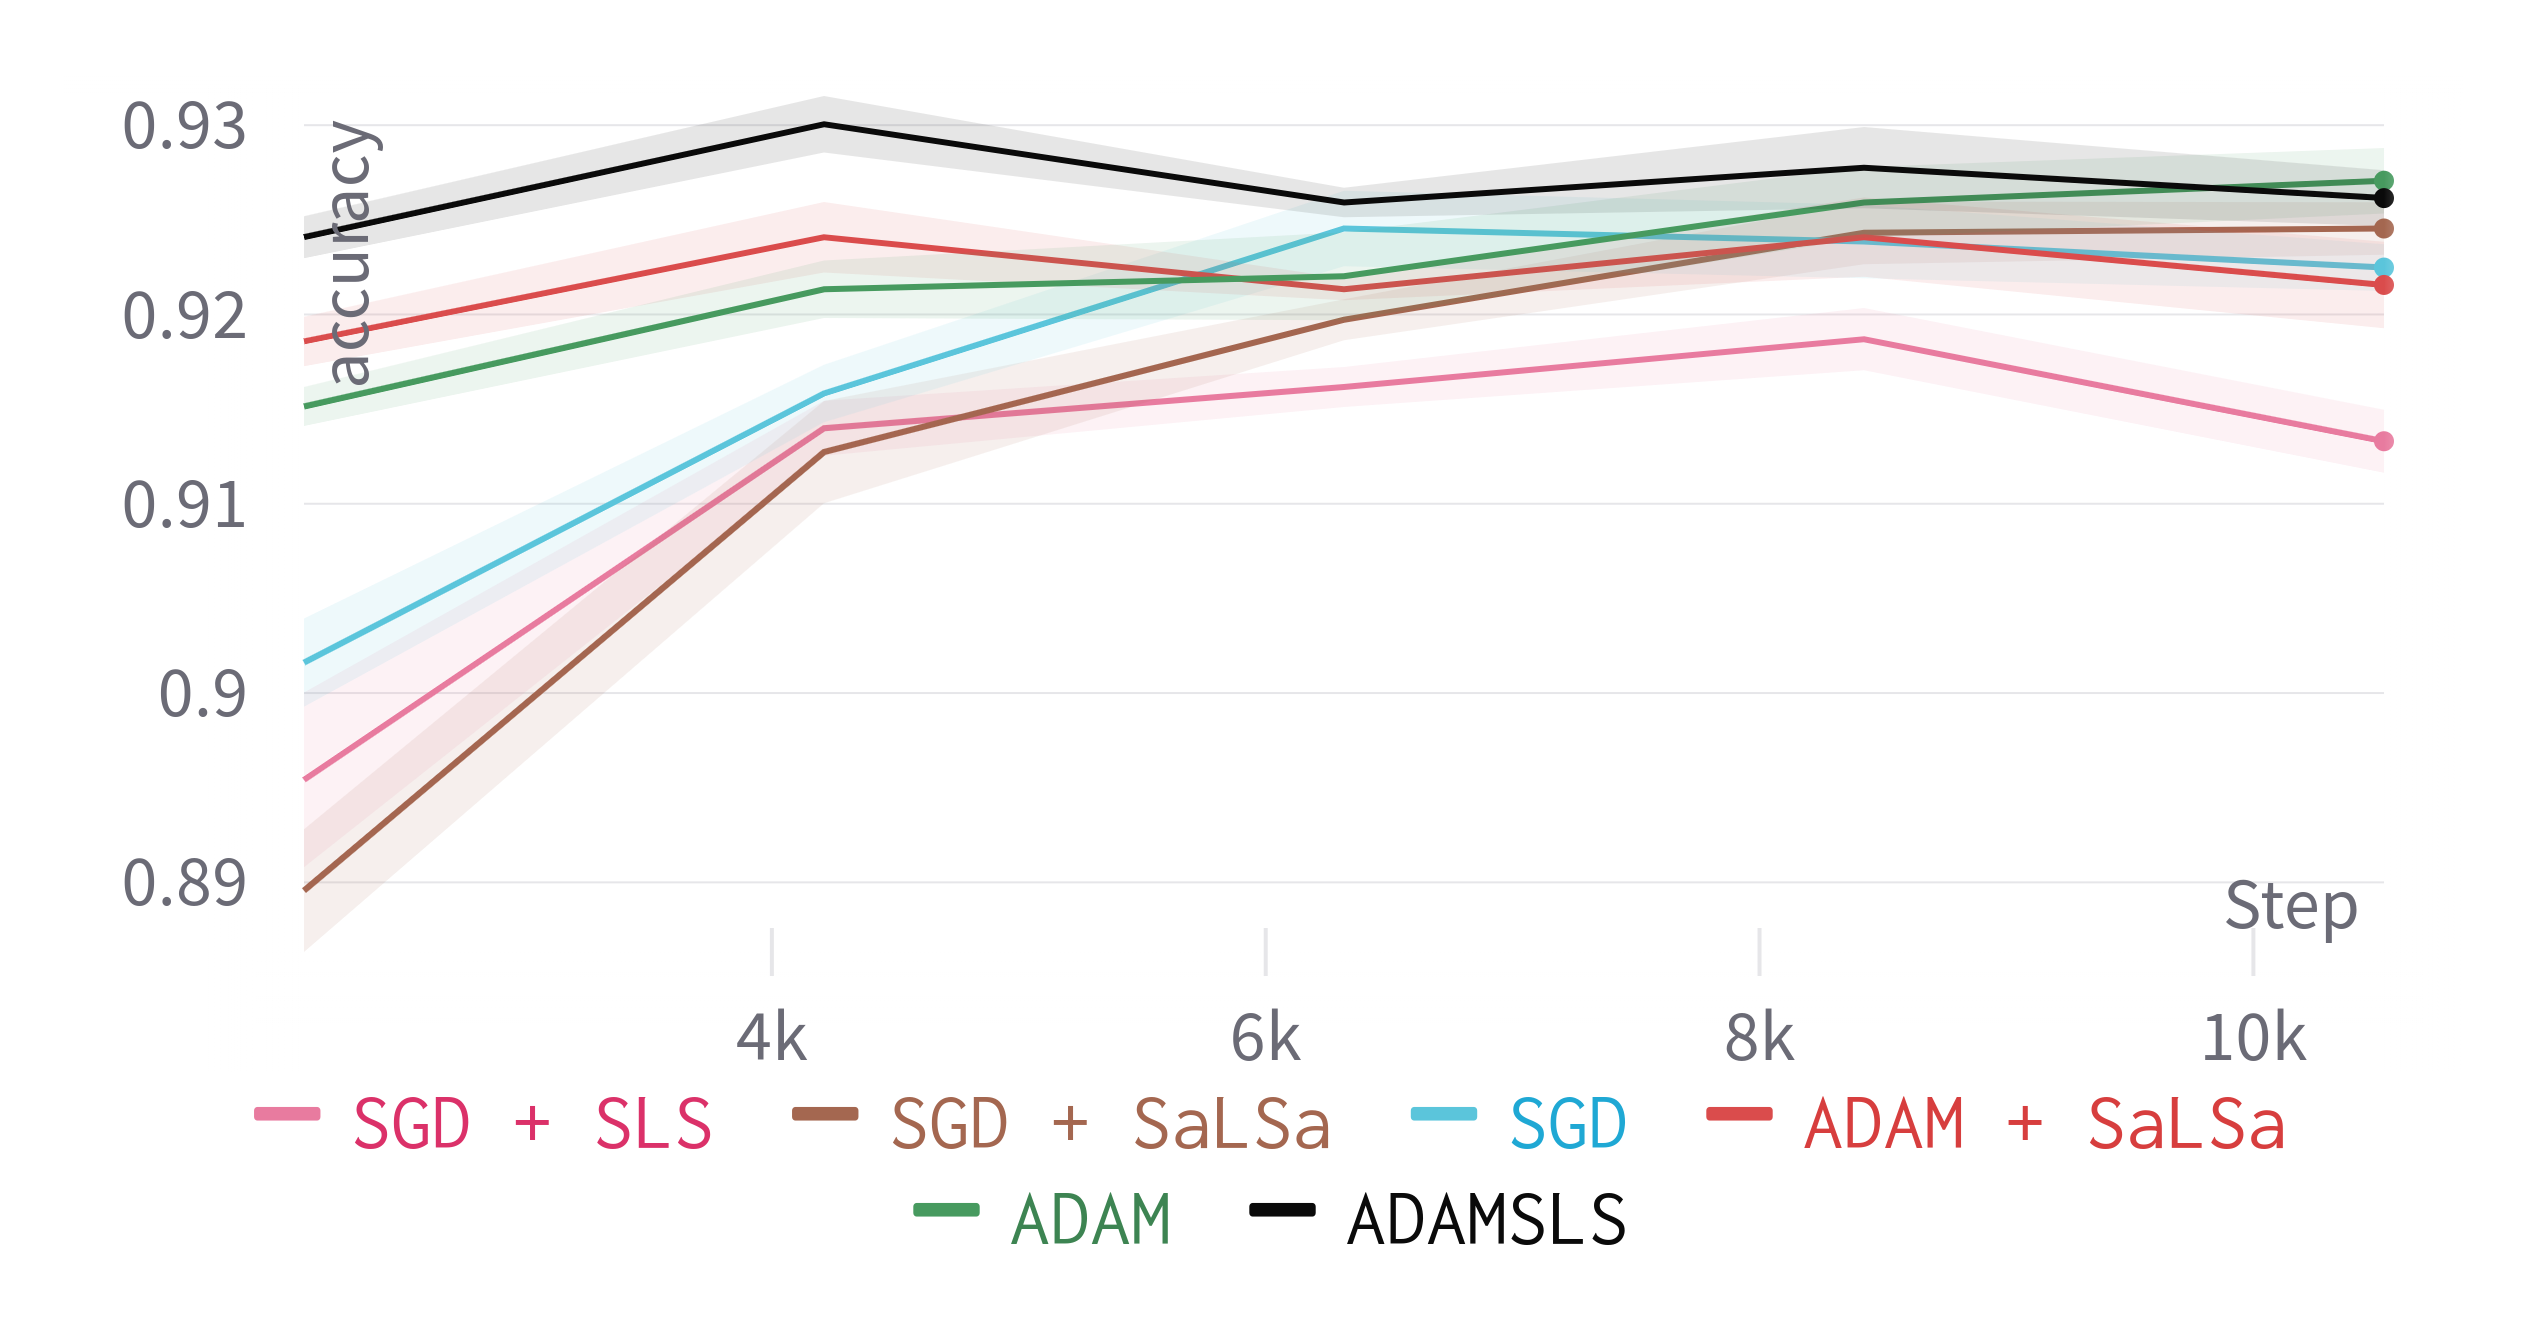}}

\caption{The loss (top row) and accuracy curves of the EfficientNet experiment and the SST2 experiment and the GPT-2 experiment with standard error indicated around each line, starting after the first epoch. Accuracy was calculated on the validation data, while loss was calculated on the training data. No Accuracy is displayed for GPT-2, since it is not trained on a classification task.}
\label{fig:extra}
\end{figure}

\newpage
\subsection{Proof for Theorem 1}
\label{sec:proofappendix}
Below we show a theoretical proof for Theorem 1 and display training runs where we applied the non decrease condition $f(w_k) - f(w_k + \eta_k d_k) \geq 0$, by lowering the step size until it is fulfilled for each step, see Figure \ref{fig:lossdec}. The effect of this additional constraint does not affect the optimization process significantly.

\begin{figure}[h!]

\subfloat[MNLI]{\includegraphics[width = 0.48\textwidth]{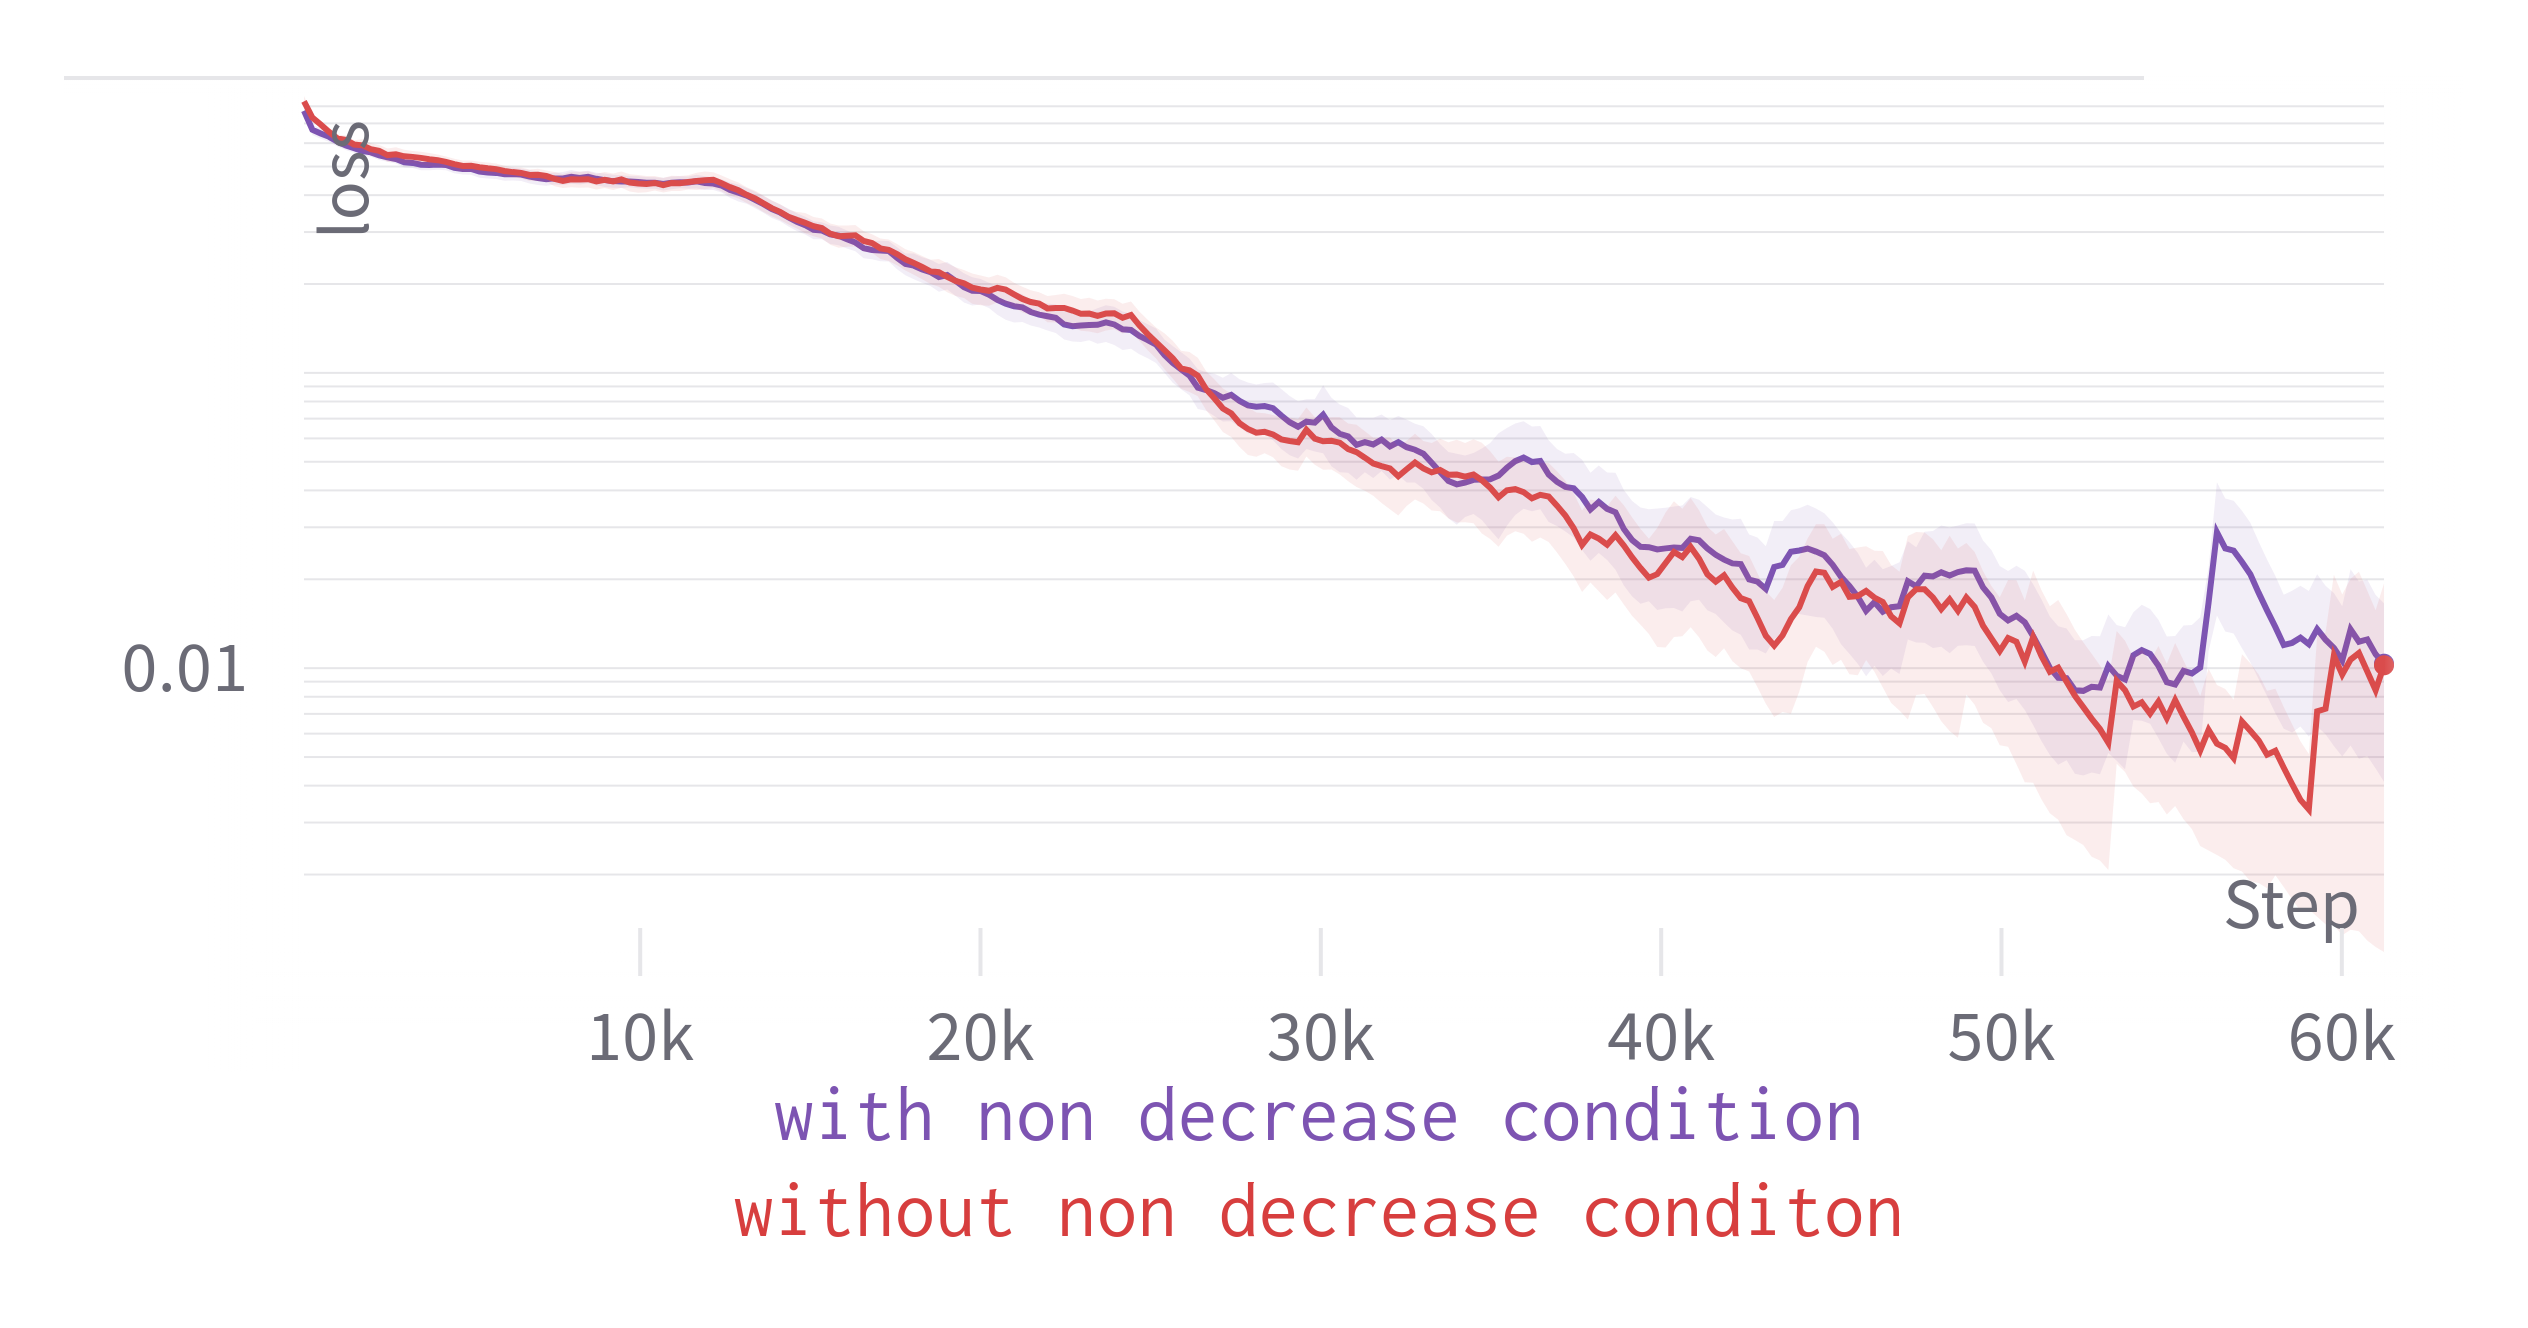}}
\subfloat[SST2]{\includegraphics[width = 0.48\textwidth]{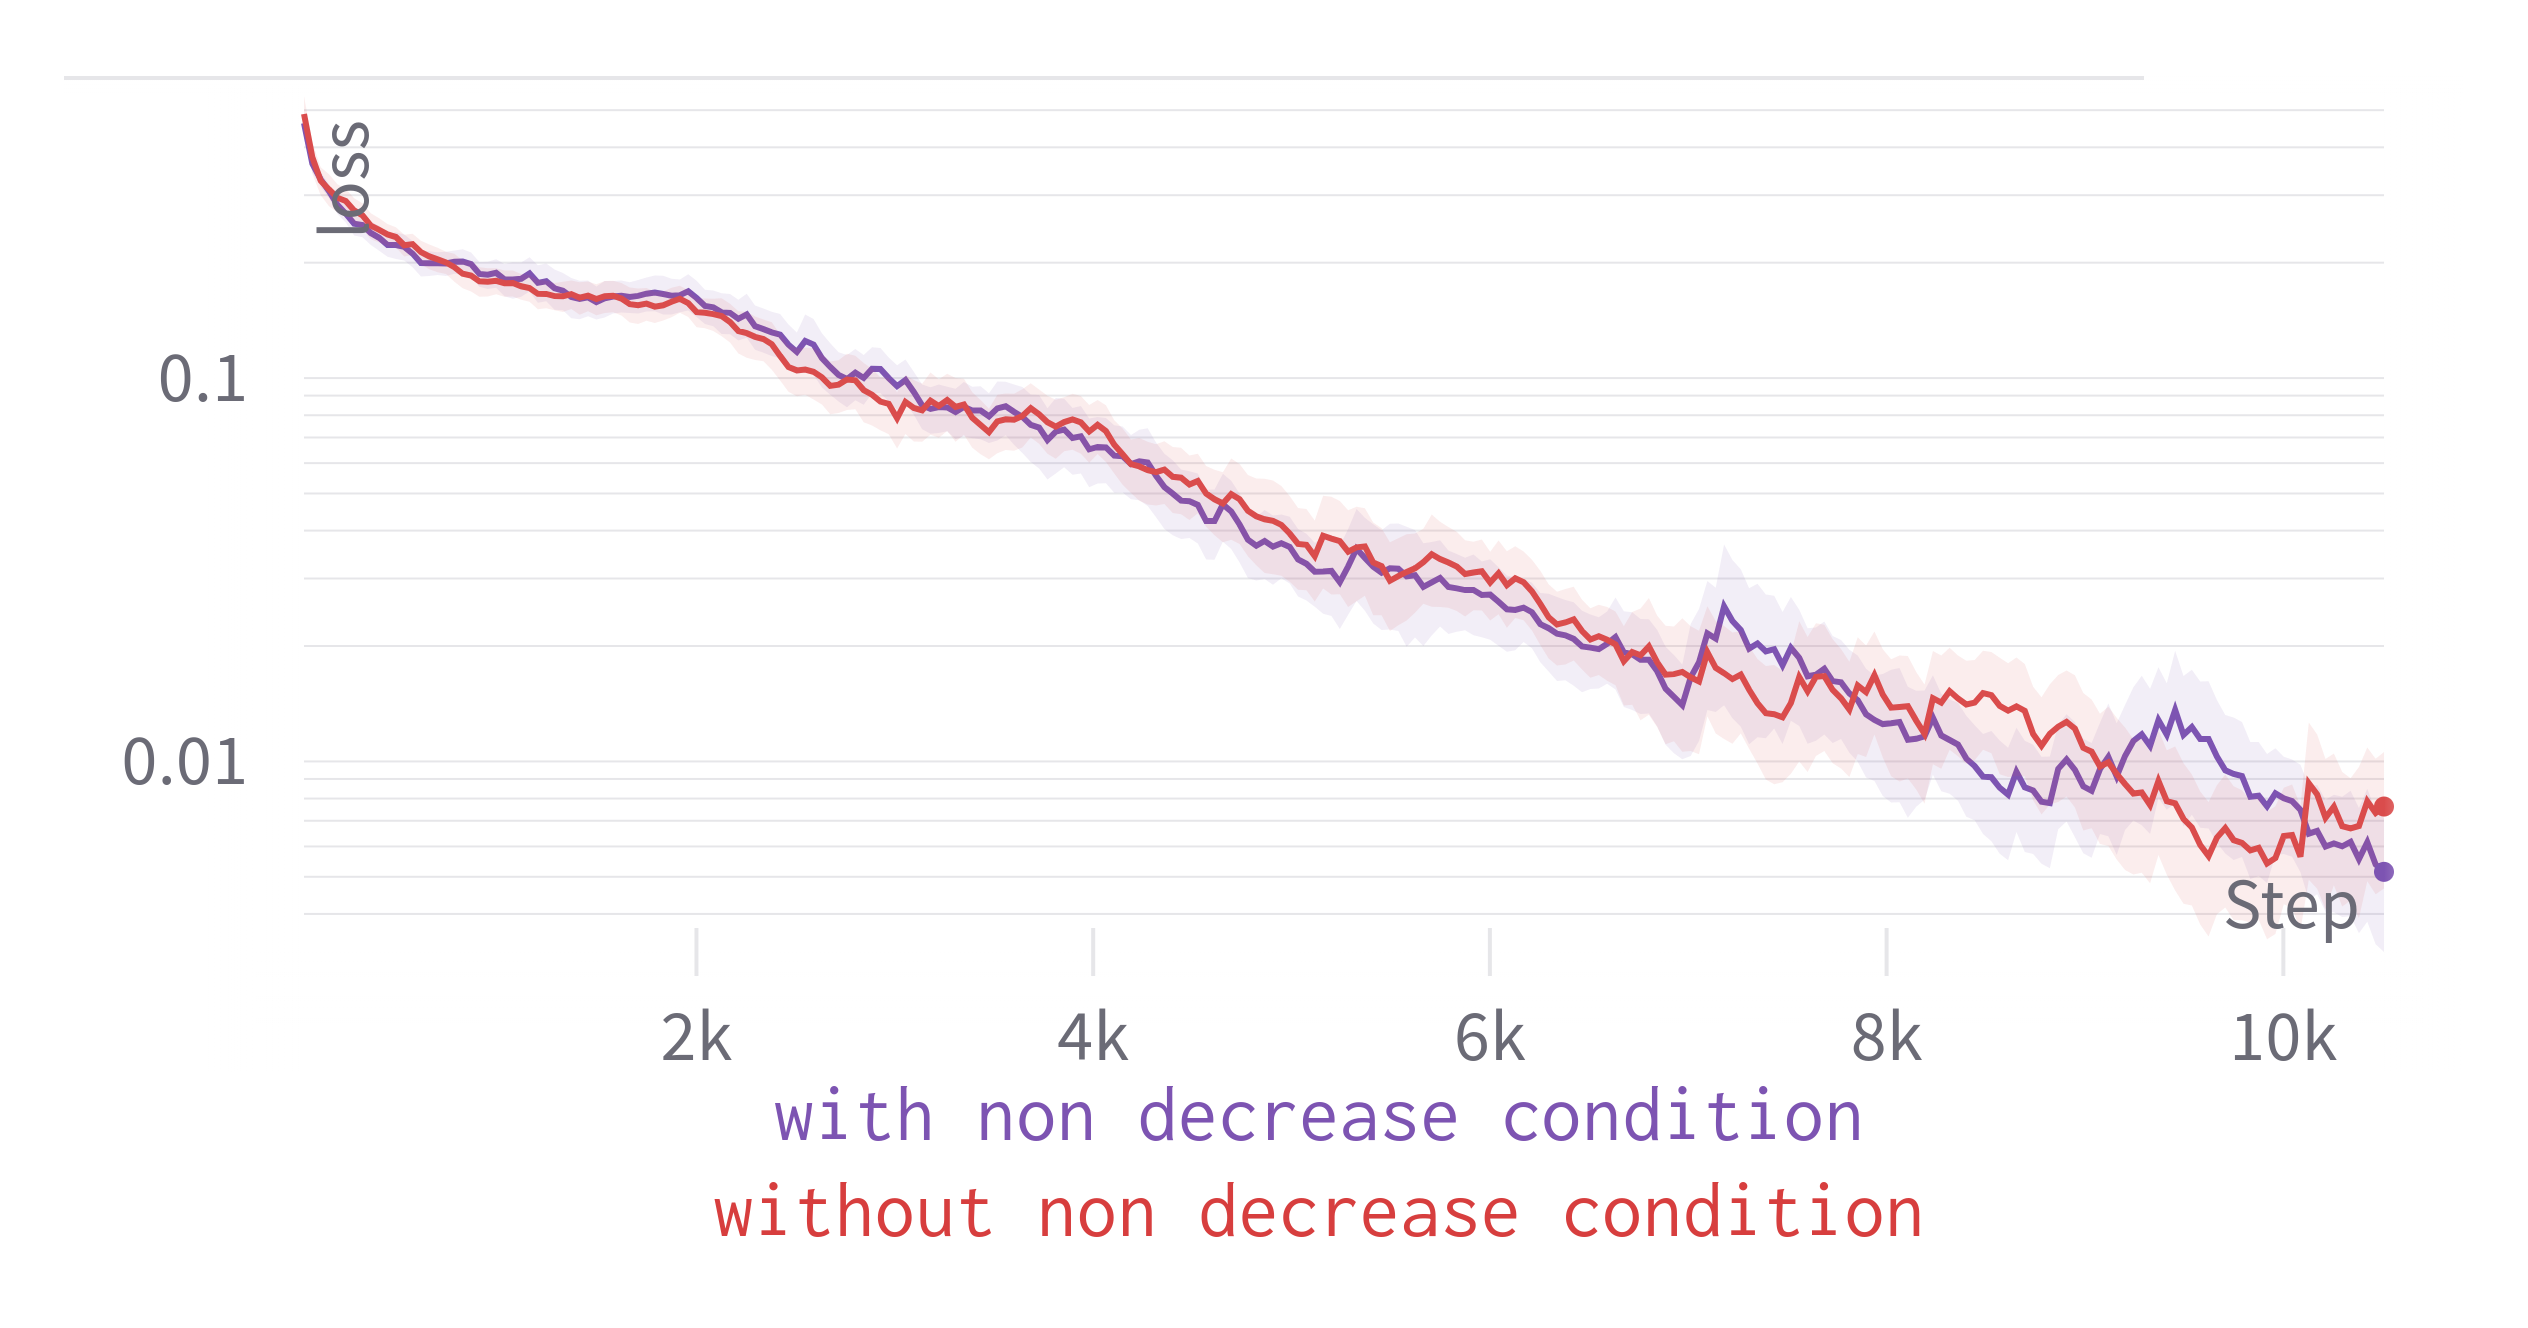}}

\caption{Average Loss curves of training on the MNLI and SST2 dataset over 5 runs with and without the additional condition required in the proof.}
\label{fig:lossdec}
\end{figure}

\begin{proof}
    The condition $f(w_k) - f(w_k + \eta_k d_k) \geq 0$ ensures that $\{f(w_k)\}_{k=1}^K$ is non-increasing and thus any infinite sequence will converge to $f(w^*)$, given the assumptions.
    It thus remains to show, that in every step such a step size $\eta_k$ can be found.
    By definition, we have that
    \begin{align*}
        h_k &= \beta_3 h_{k-1} + (1-\beta_3) \left[f(w_k) - f(w_k + \eta_k d_k)\right]
        \\
        &\geq \beta_3 c \eta_{k-1} s_{k-1} + (1-\beta_3) \left[f(w_k) - f(w_k + \eta_k d_k)\right].
    \end{align*}
        If we assume, that there exists a learning rate $\eta_k\leq\eta_{k-1}$, such that $f(w_k) - f(w_k + \eta_k d_k) \geq c \eta_k \Vert \nabla f(w_k)\Vert^2$ (see proof of existence below), we can show that
    \begin{align*}
        \beta_3 c \eta_{k-1} s_{k-1} + (1-\beta_3) \left[f(w_k) - f(w_k + \eta_k d_k)\right] &\geq c \eta_{k}\left[\beta_3 s_{k-1} + (1-\beta_3) \Vert \nabla f(w_k)\Vert^2\right]
        \\
        &= c \eta_{k} s_{k},
    \end{align*}
    which finishes the proof, as we have found a learning rate $\eta_k$ that fulfills the SaLSa criterion.
    
    We now prove the existence of $\eta_k\leq\eta_{k-1}$ with $f(w_k) - f(w_k + \eta_k d_k) \geq c \eta_k \Vert \nabla f(w_k)\Vert^2$ by contradiction, i.e. we assume that such a $\eta_k$ does not exist and thus $f(w_k) - f(w_k + \eta_k d_k) < c \eta_k \Vert \nabla f(w_k)\Vert^2$ for $\eta_k \leq \eta_{k-1}$. 
    Using the Taylor expansion for $f$ around $f(w_k)$ yields 
    \begin{align*}
         f(w_k) - f(w_k + \eta_k d_k) = -\eta_k d_k \nabla f (w_k) - o(\eta_k).
    \end{align*}
    For $\eta_k \leq \eta_{k-1}$ it follows then
    \begin{align*}
        c \eta_k \Vert \nabla f(w_k)\Vert^2 > -\eta_k d_k \nabla f (w_k) - o(\eta_k).
    \end{align*}
    Dividing both sides by $\eta_k$ and taking the limit for $\eta_k \to 0$ yields
    \begin{align*}
         c \Vert \nabla f(w_k)\Vert^2 > -d_k \nabla f (w_k),
    \end{align*}
    and thus with $d_k = - \nabla f(w_k)$ it follows $c > 1$, which is a contradiction.
\end{proof}

\newpage
\subsection{Hyperparameter studies for $\beta_3$ and $c$}
\label{sec:hypercandb}
\begin{figure}[h!]

\subfloat[MRPC]{\includegraphics[width = 0.48\textwidth]{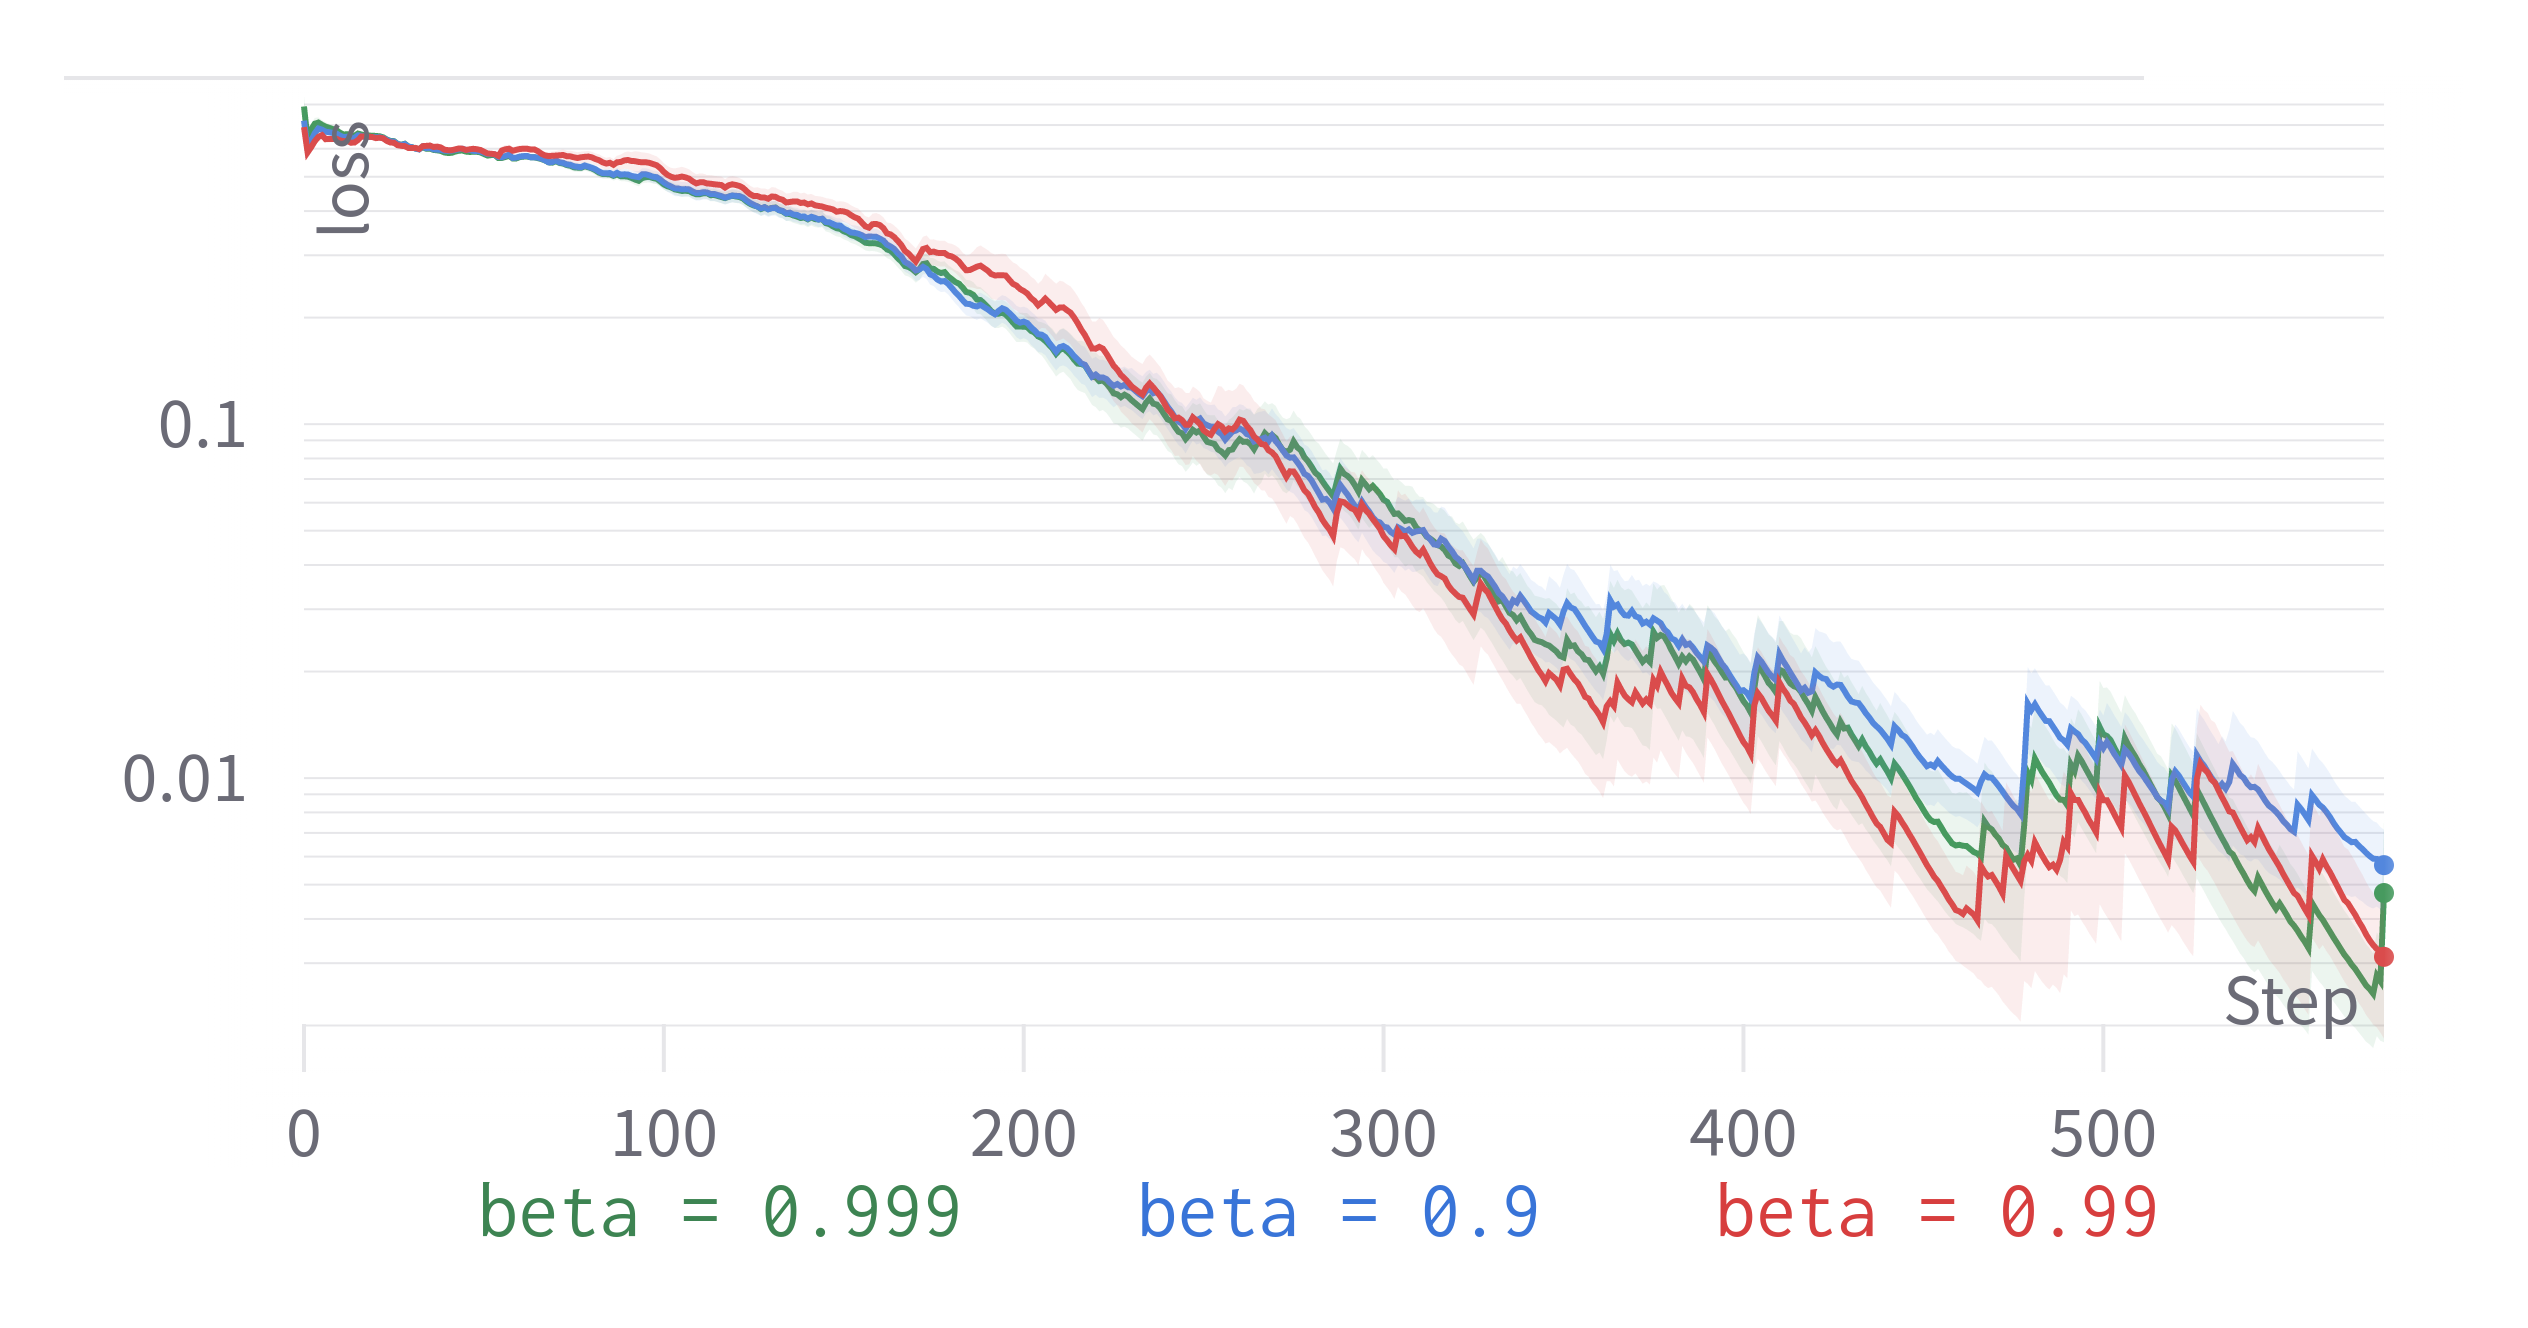}}
\subfloat[MNLI]{\includegraphics[width = 0.48\textwidth]{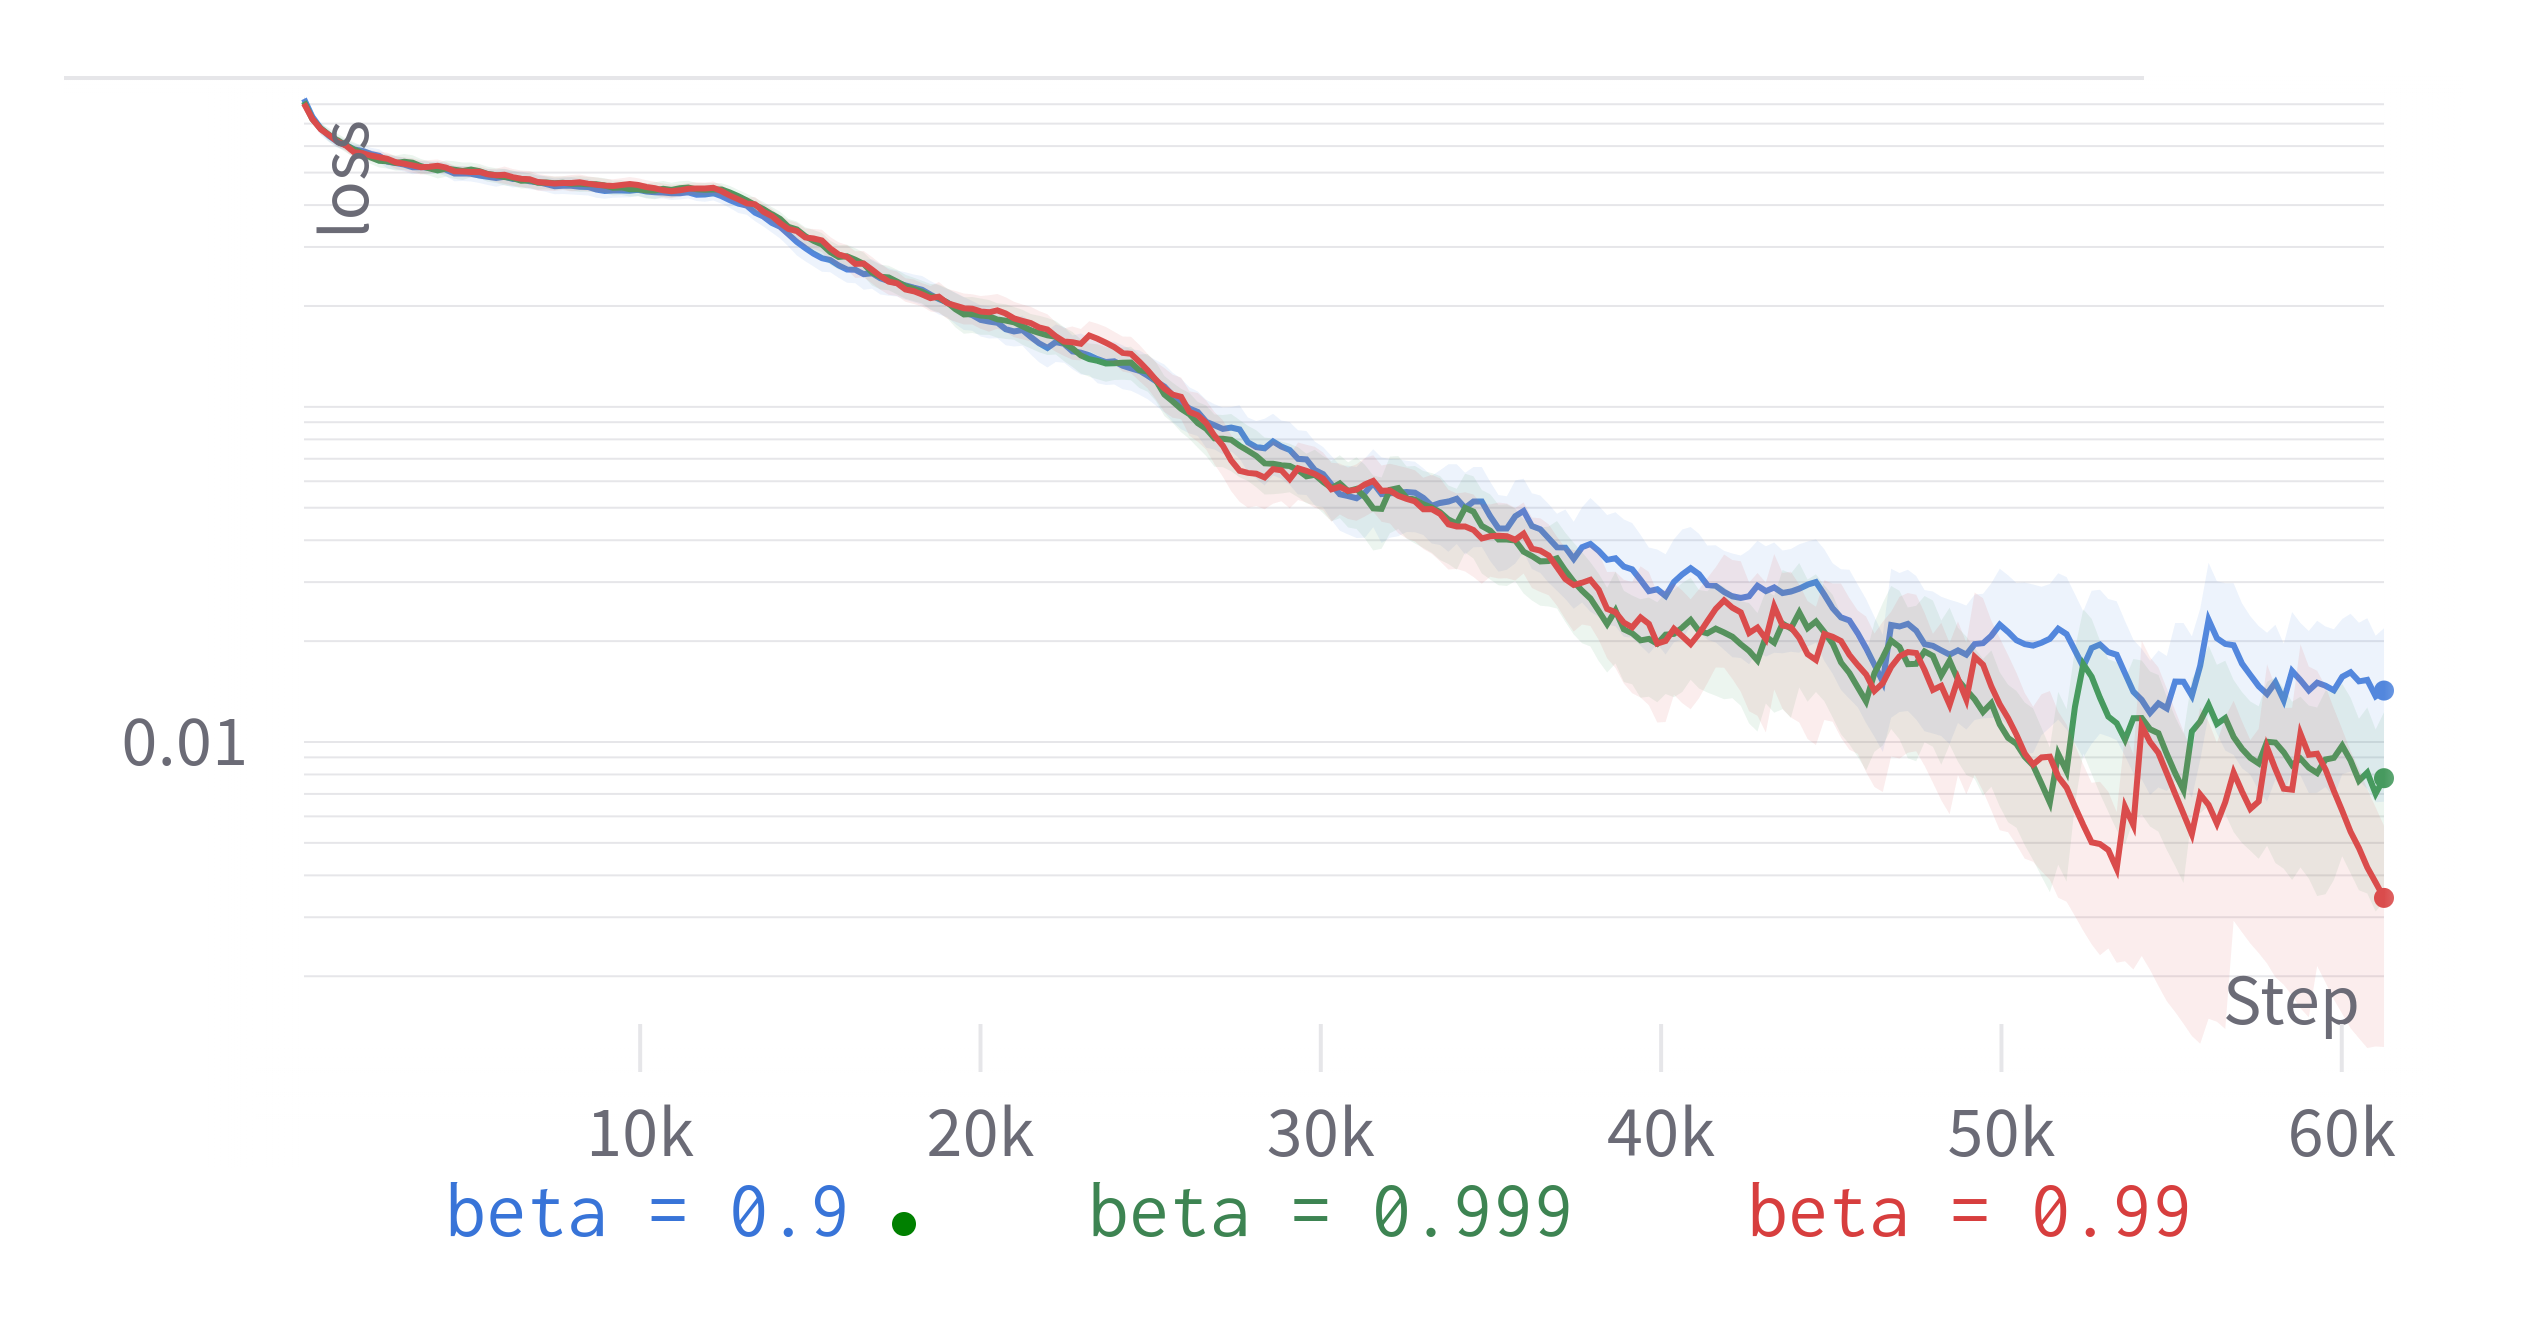}}

\caption{Average loss curves of training on the MRPC and SST2 dataset over 5 runs with different values for $\beta_3$ for the SaLSa + ADAM optimizer}
\label{fig:lossdec}
\end{figure}

\begin{figure}[h!]

\subfloat[MRPC]{\includegraphics[width = 0.48\textwidth]{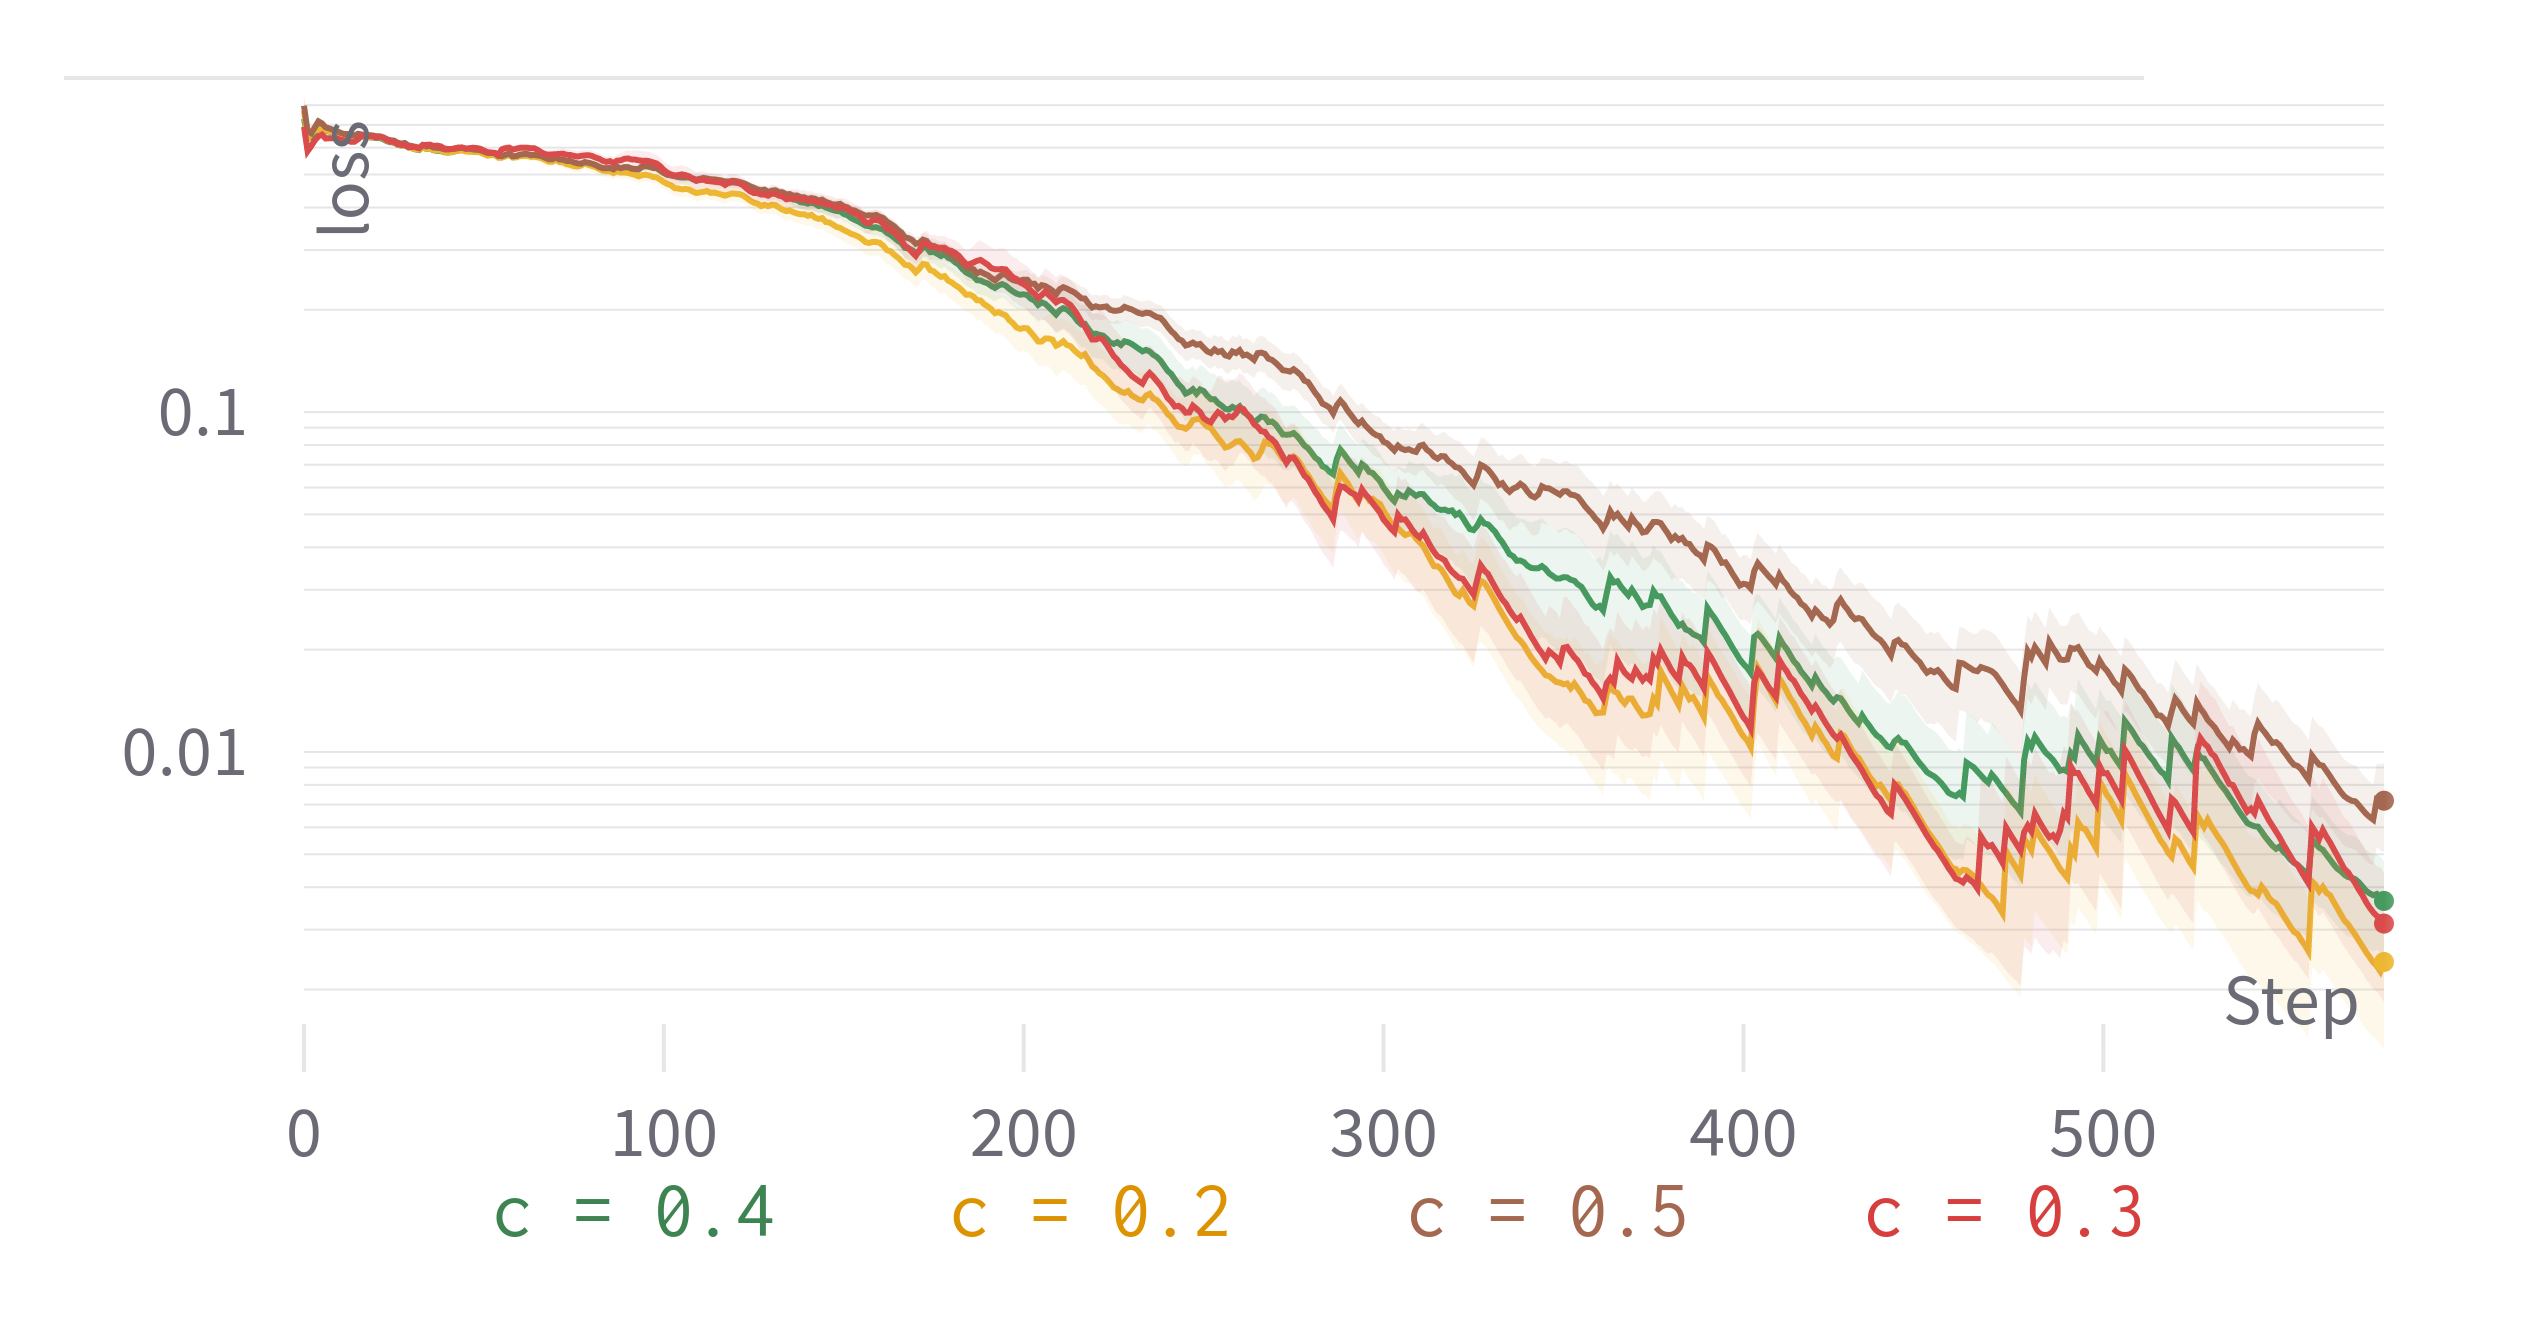}}
\subfloat[SST2]{\includegraphics[width = 0.48\textwidth]{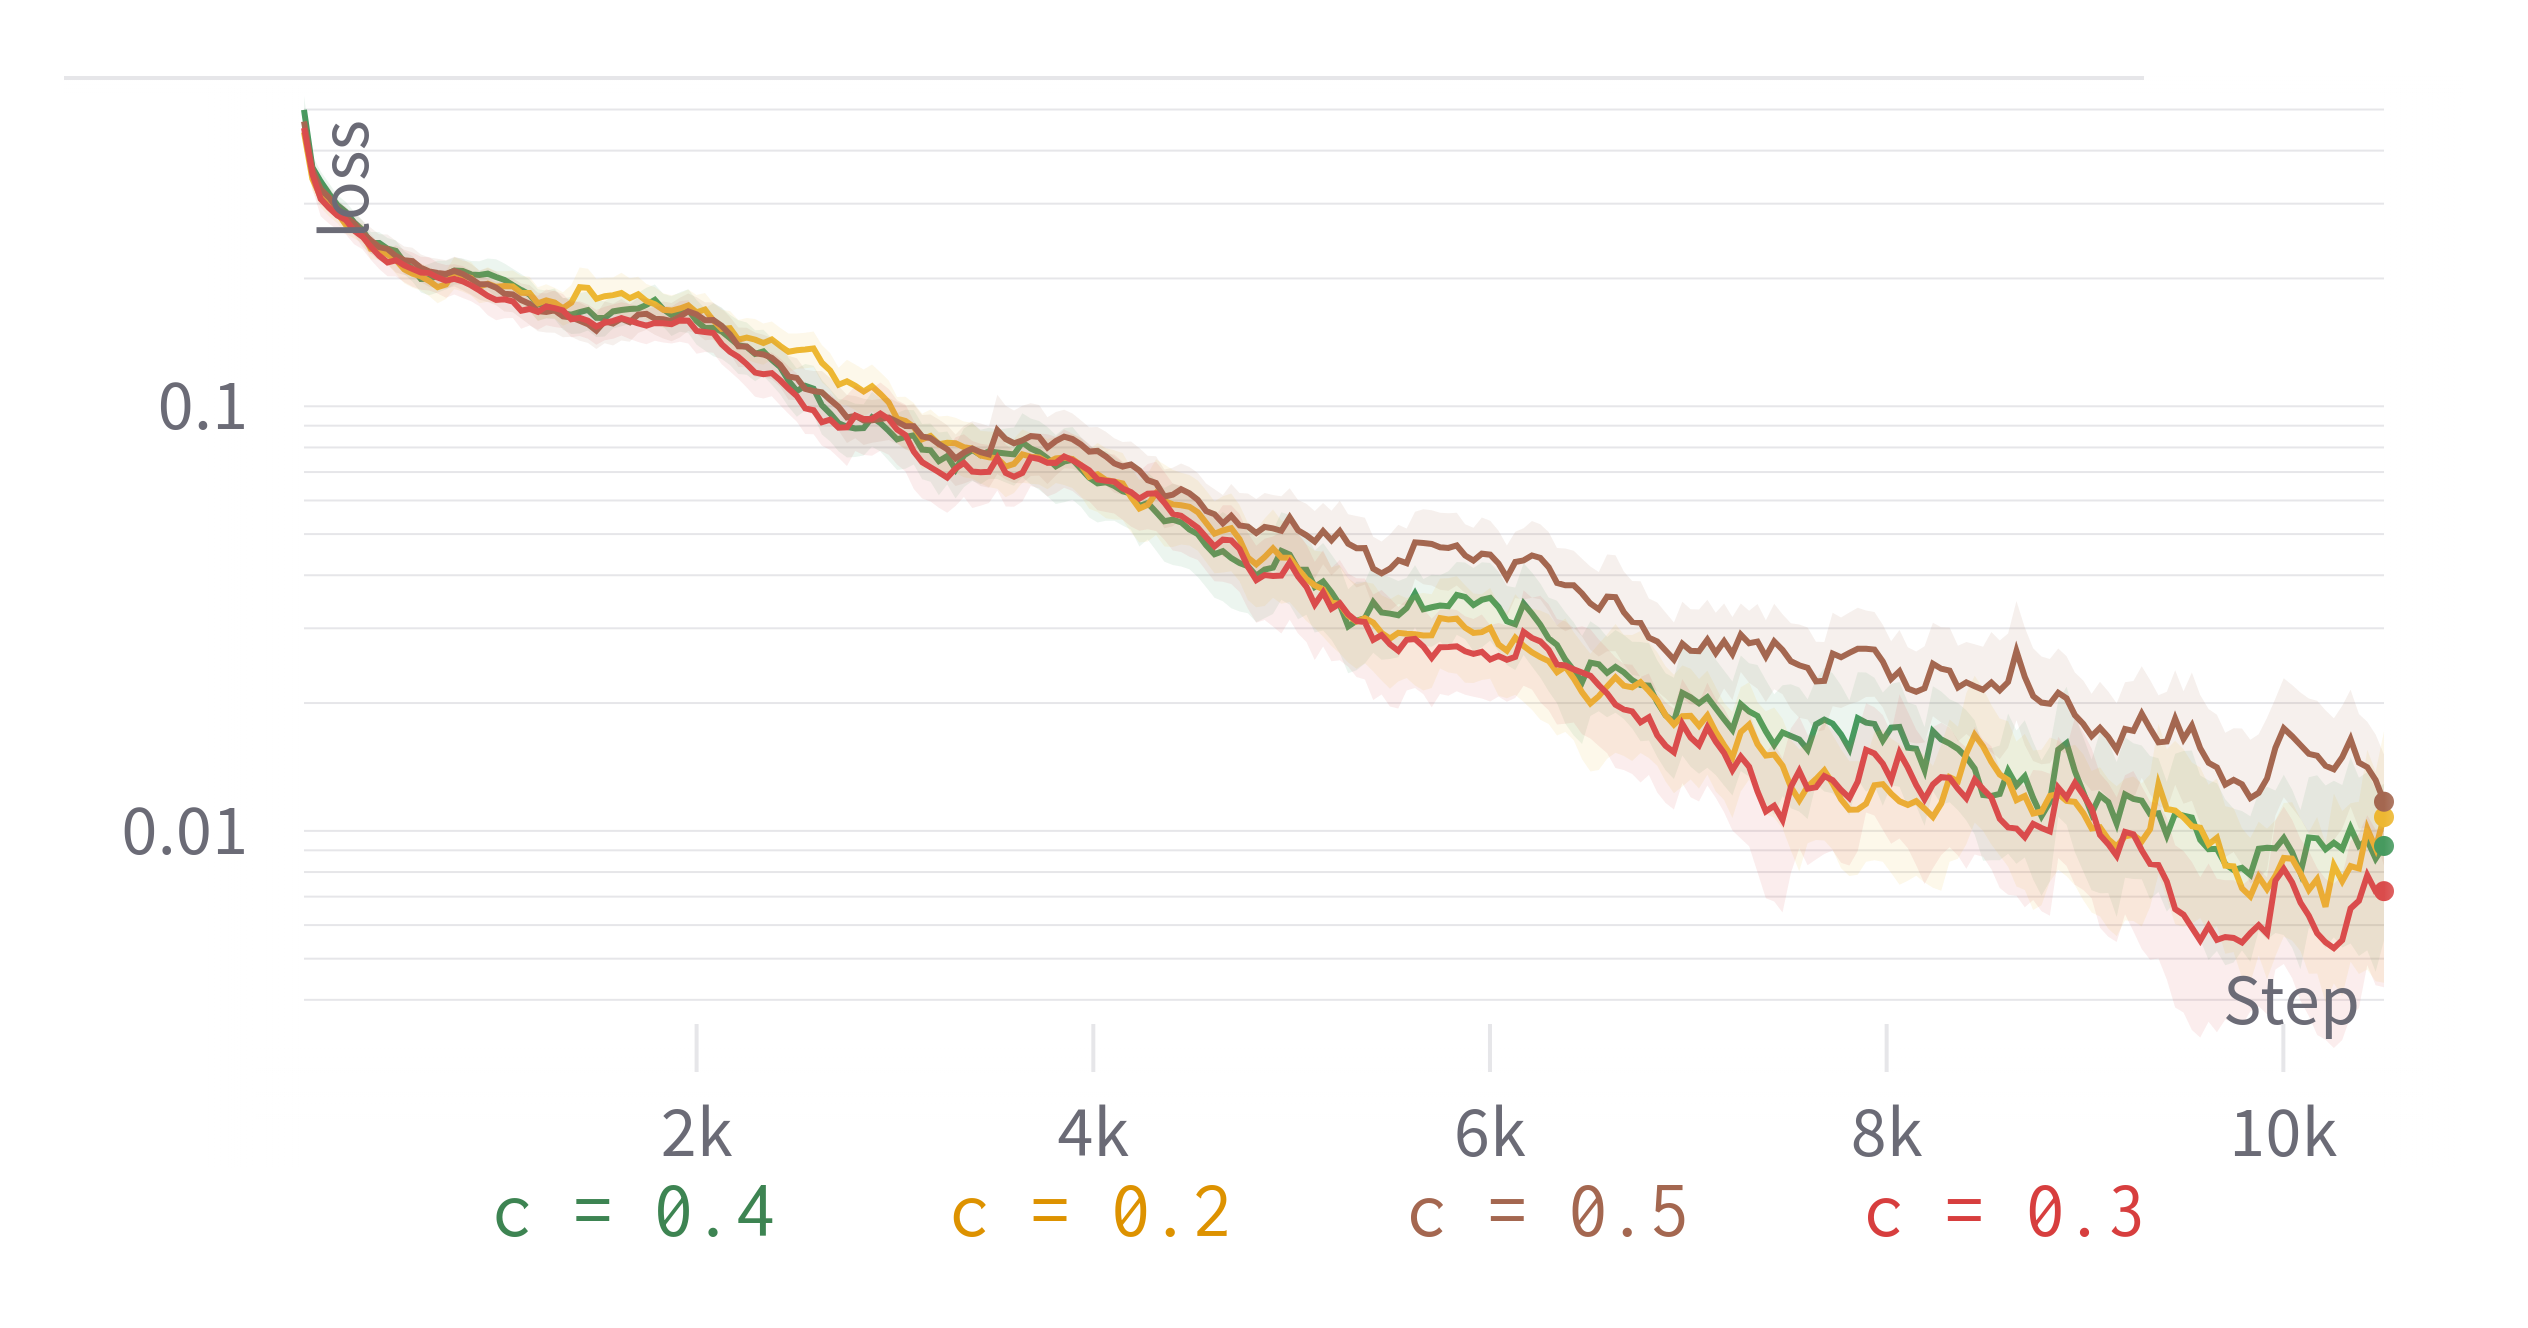}} \\
\subfloat[MNLI]{\includegraphics[width = 0.48\textwidth]{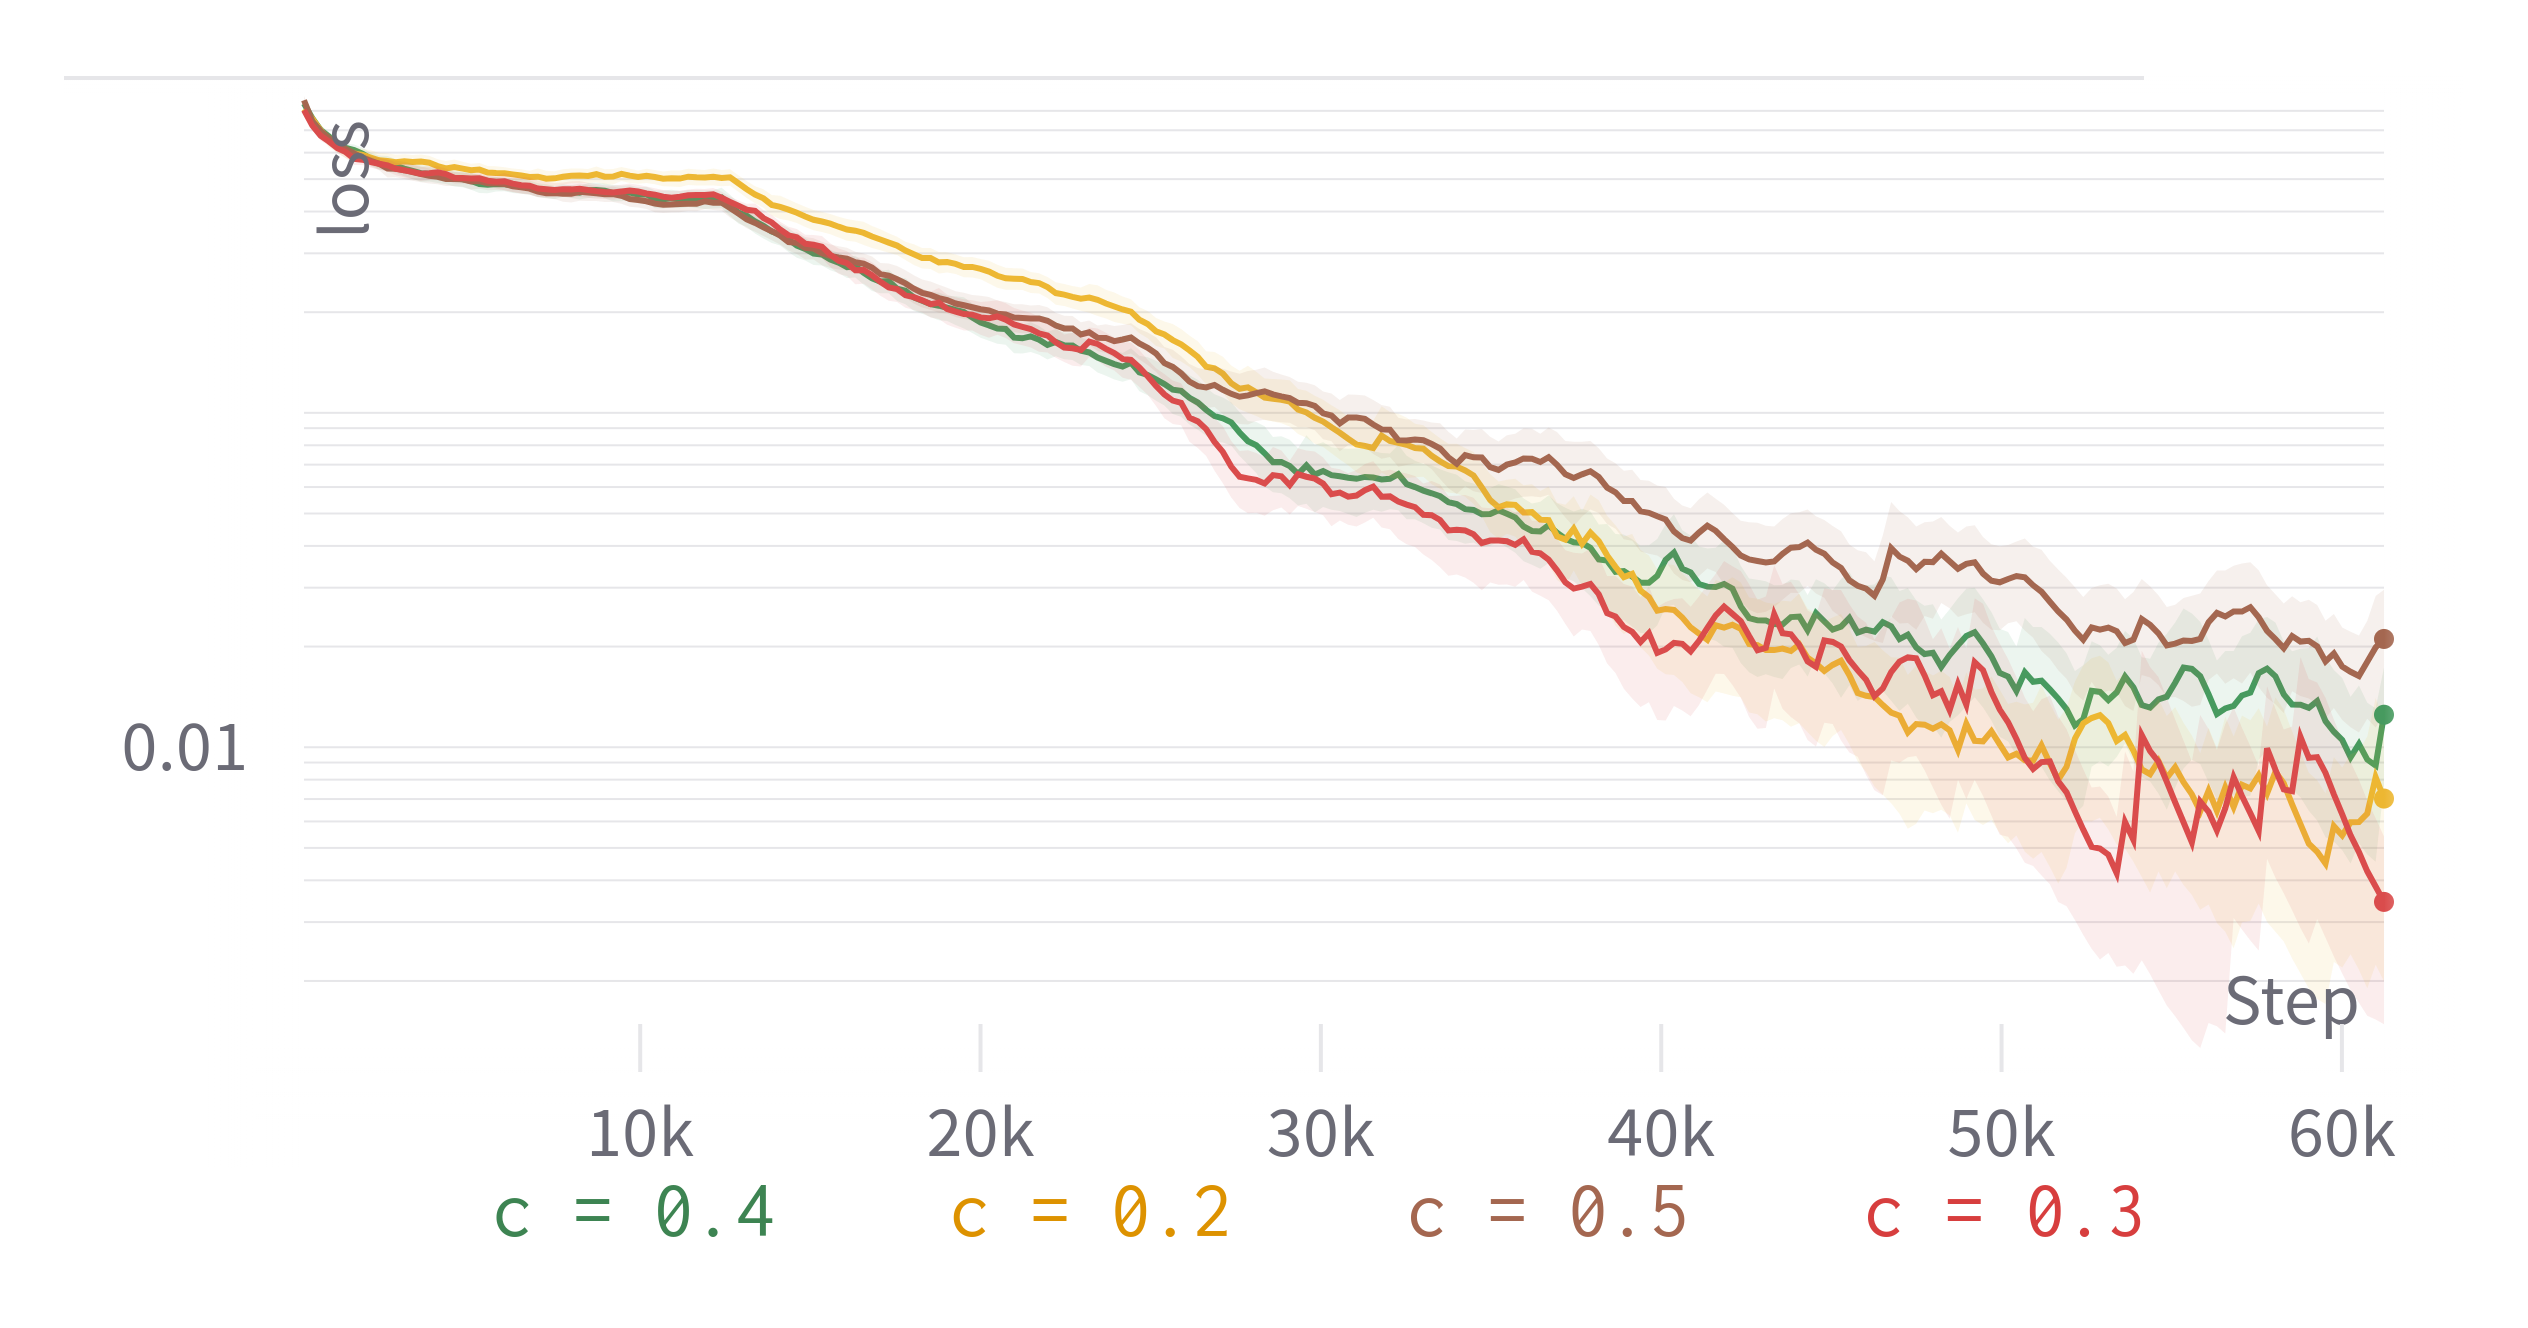}}
\subfloat[QNLI]{\includegraphics[width = 0.48\textwidth]{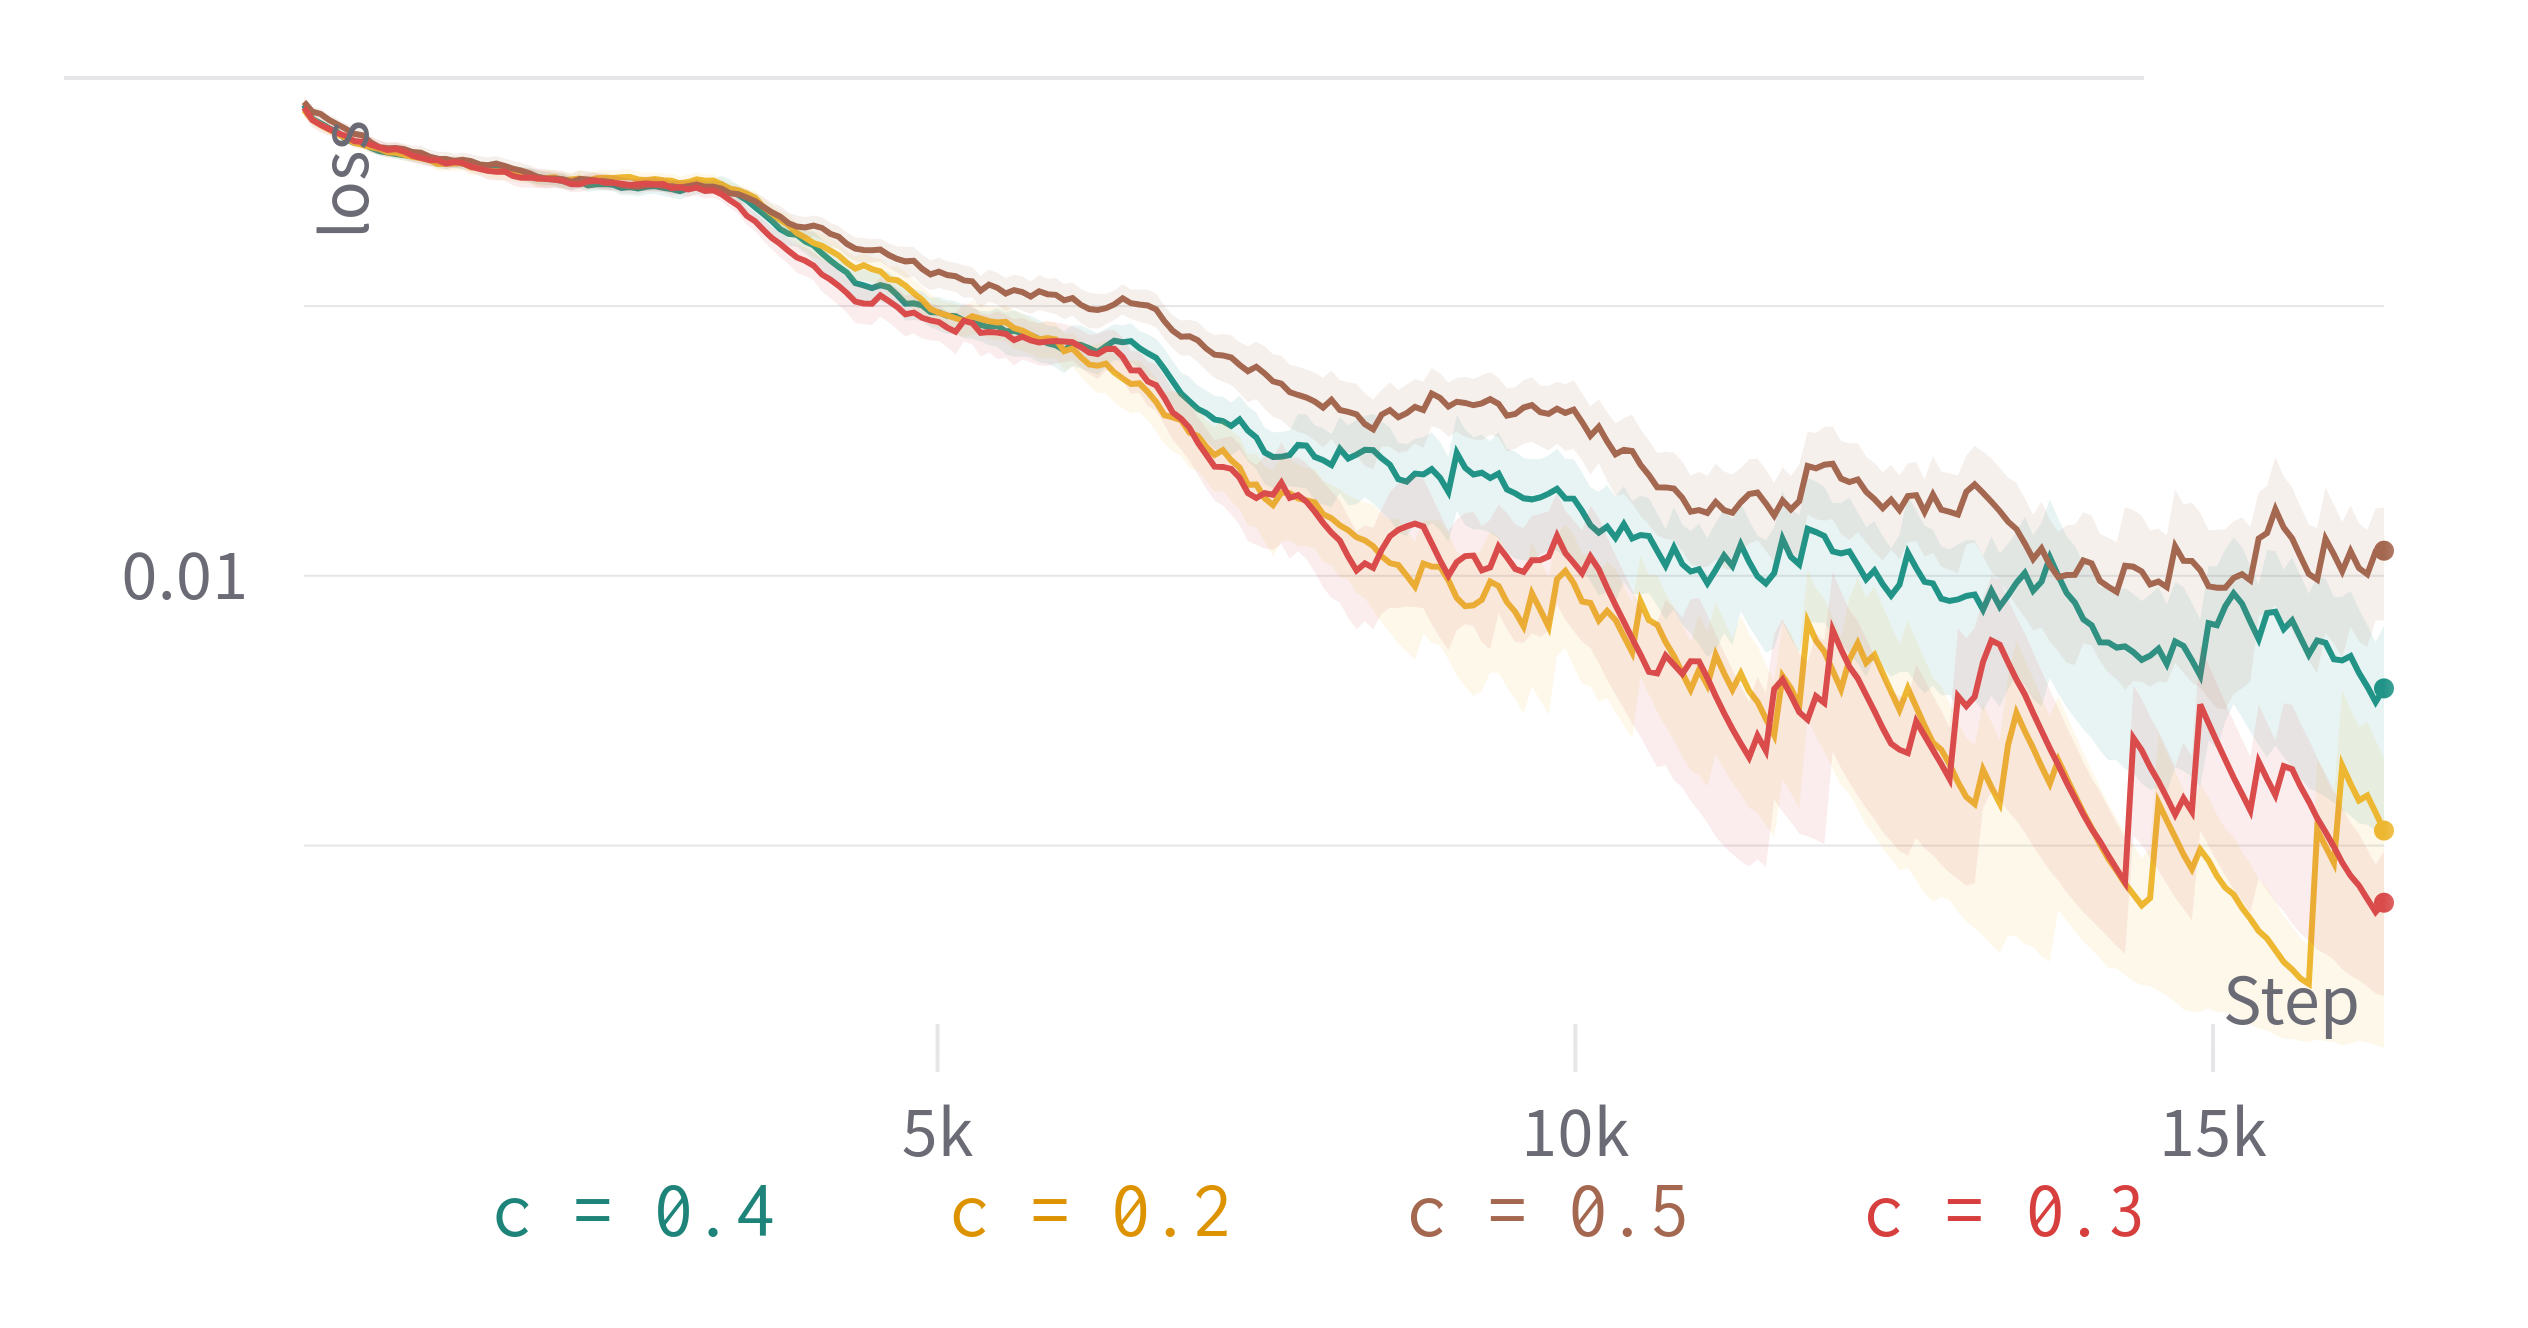}}

\caption{Average loss curves with standard error indicated of training on the GLUE dataset over 5 runs with different values for $c$ for the SaLSa + ADAM optimizer}
\label{fig:lossdec}
\end{figure}

In our Hyperparameter studies, we notice that the $\beta_3$ parameter minimally affects performance, with all training runs falling within the range of estimation error. 
The hyperarameter $c$ however does have a more substantial impact on the performance. All runs converge regardless of tested value, yet higher $c$ values exhibit a tendency to converge at a slower pace overall.

\newpage
\subsection{Limiting the Line search frequency}
\label{sec:lsappendix}
Here we show experimental results evaluating the impact of the proposed speed-up in Section \ref{sec:speedup}.

The observed difference in performance in Figure \ref{fig:speeduploss} is minor and within the margin of error.
\begin{figure}[h!]

\subfloat[QNLI]{\includegraphics[width = 0.33\textwidth]{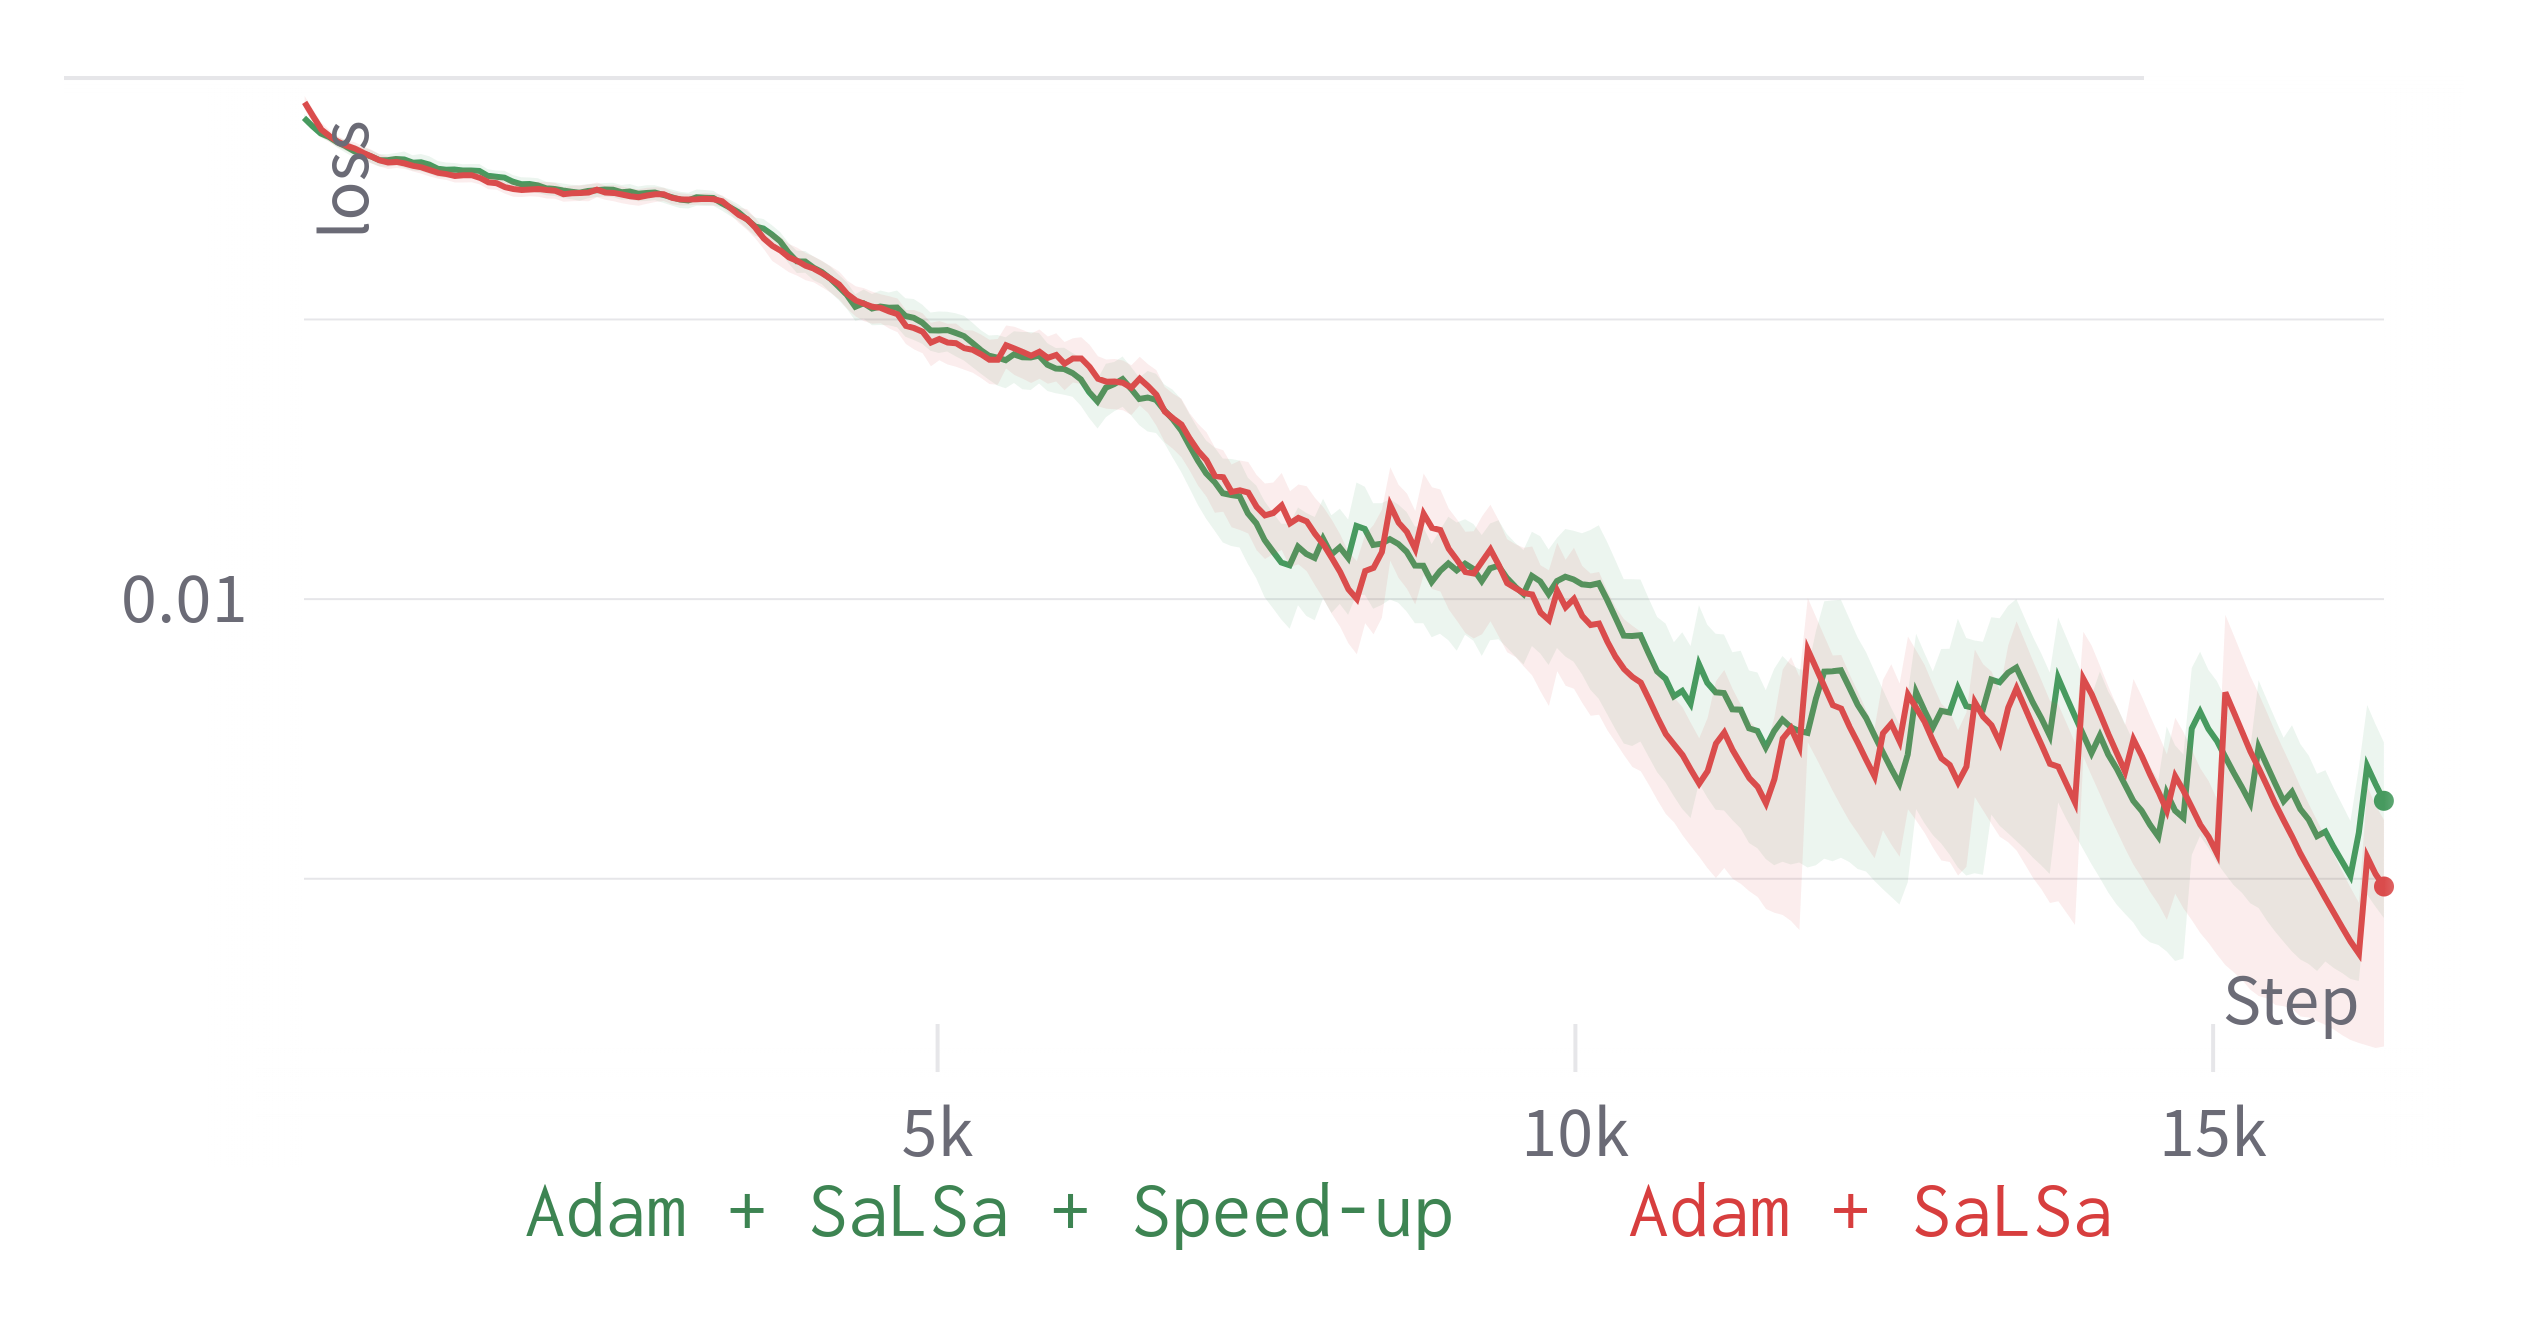}}
\subfloat[MNLI]{\includegraphics[width = 0.33\textwidth]{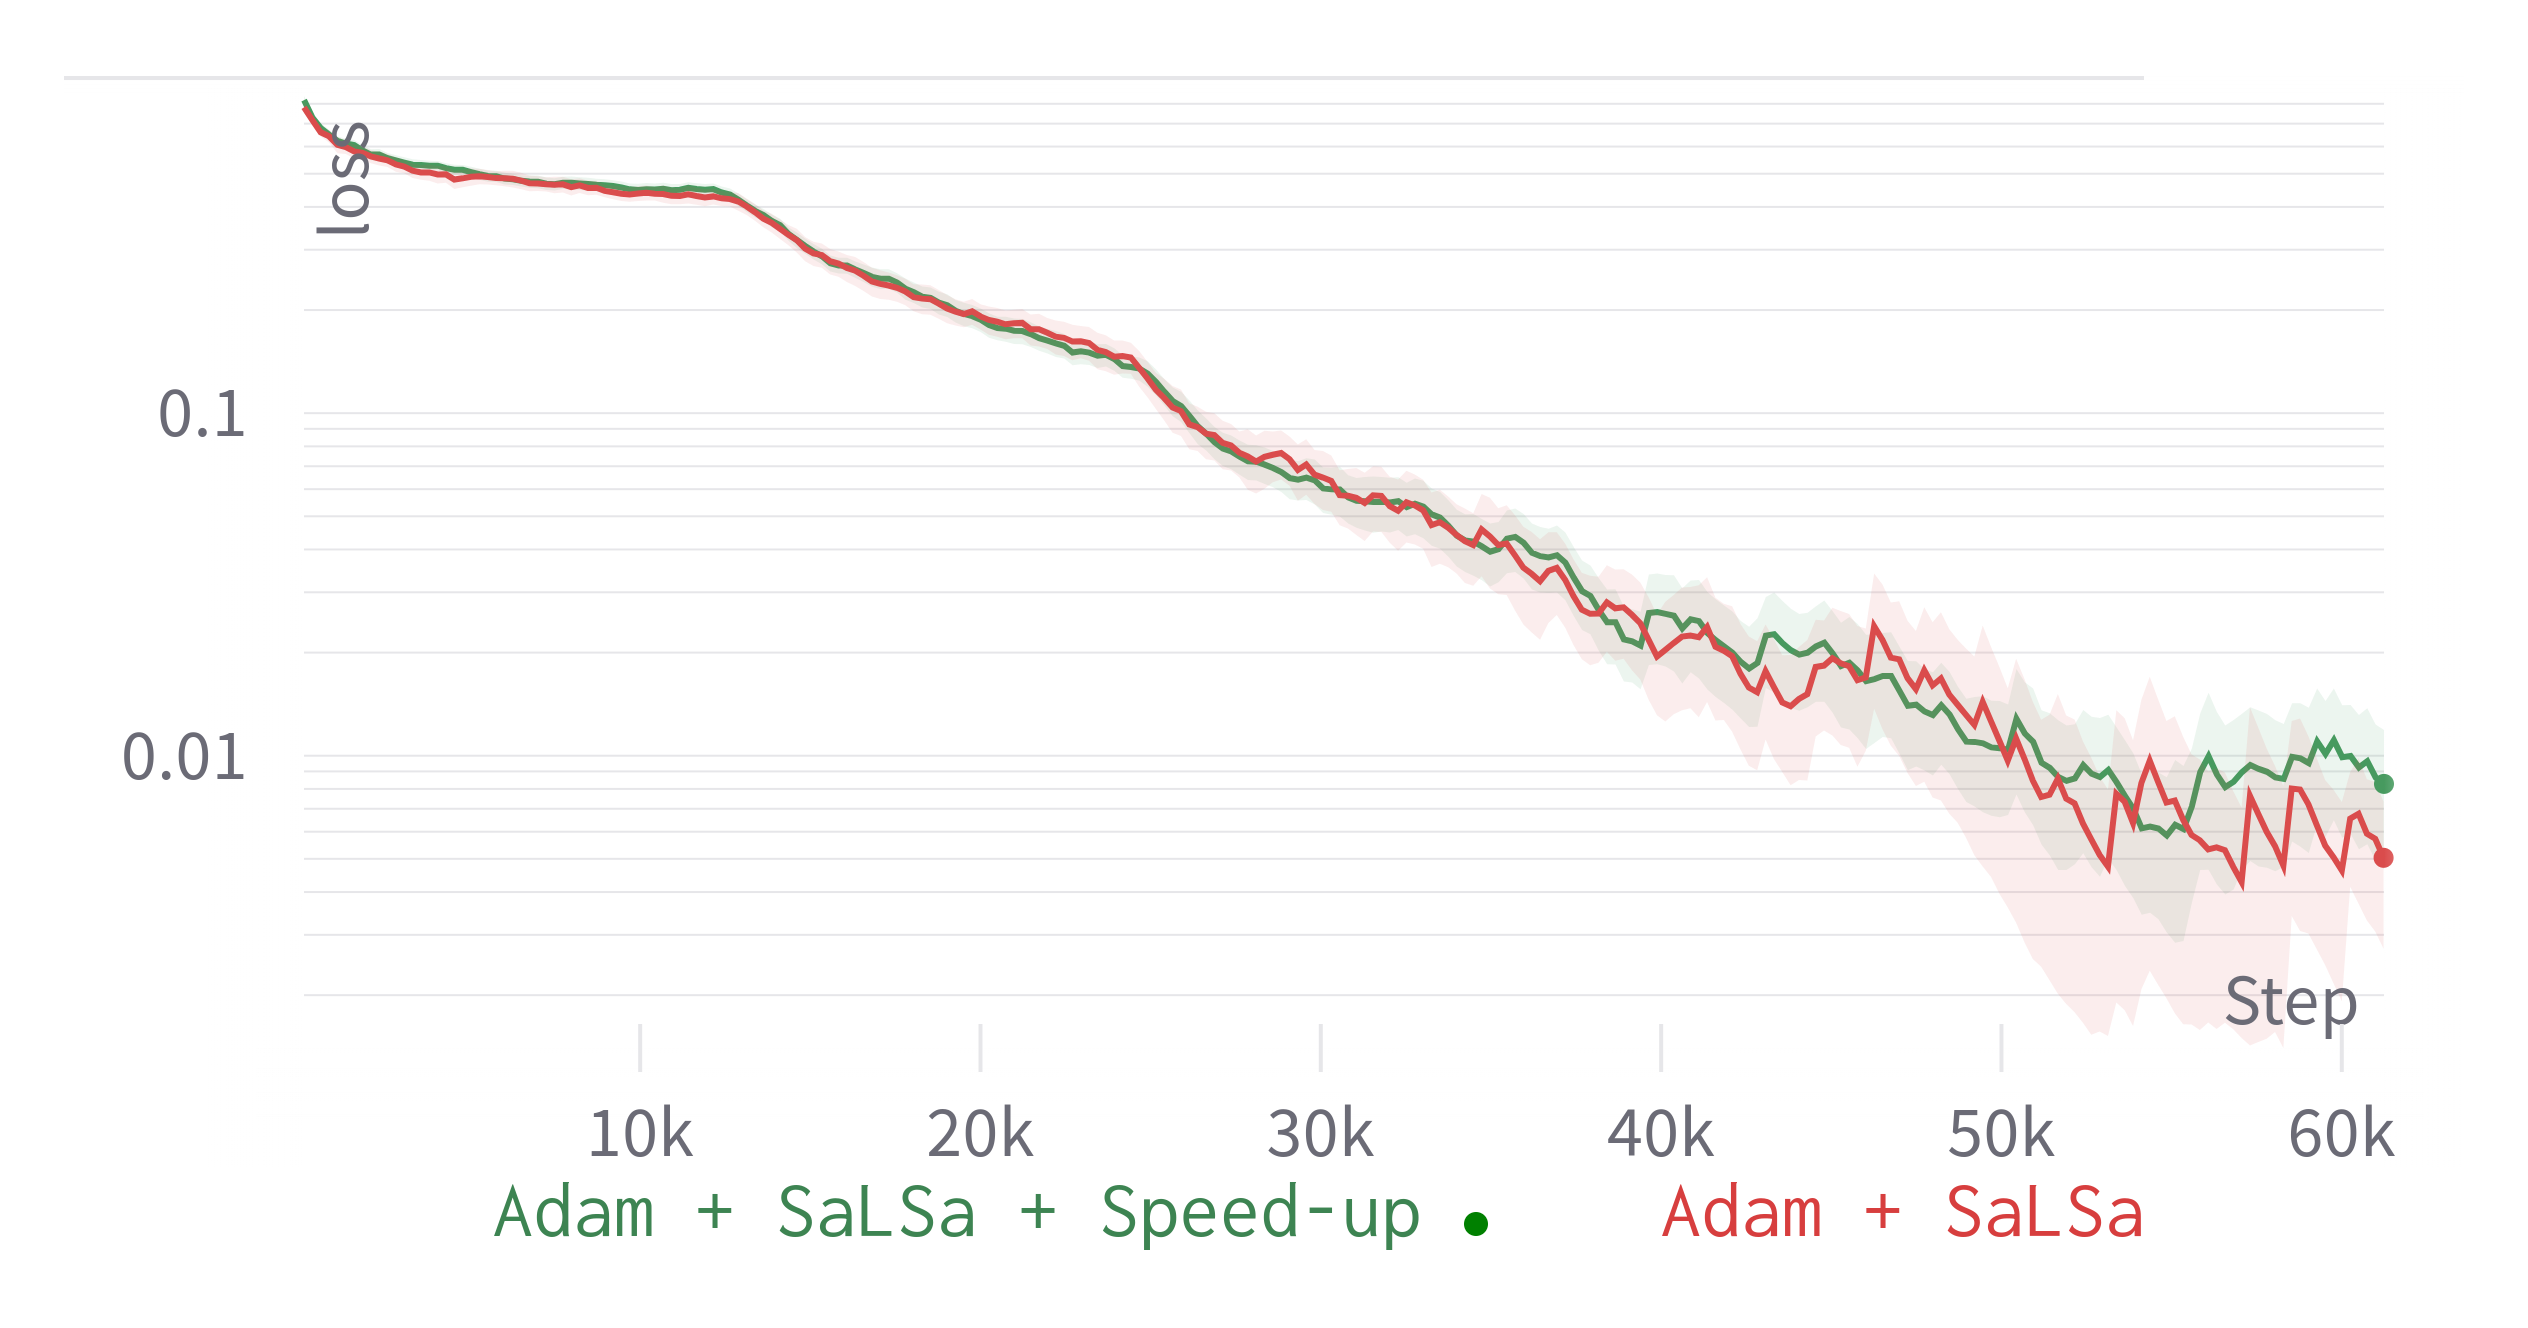}} 
\subfloat[SST2]{\includegraphics[width = 0.33\textwidth]{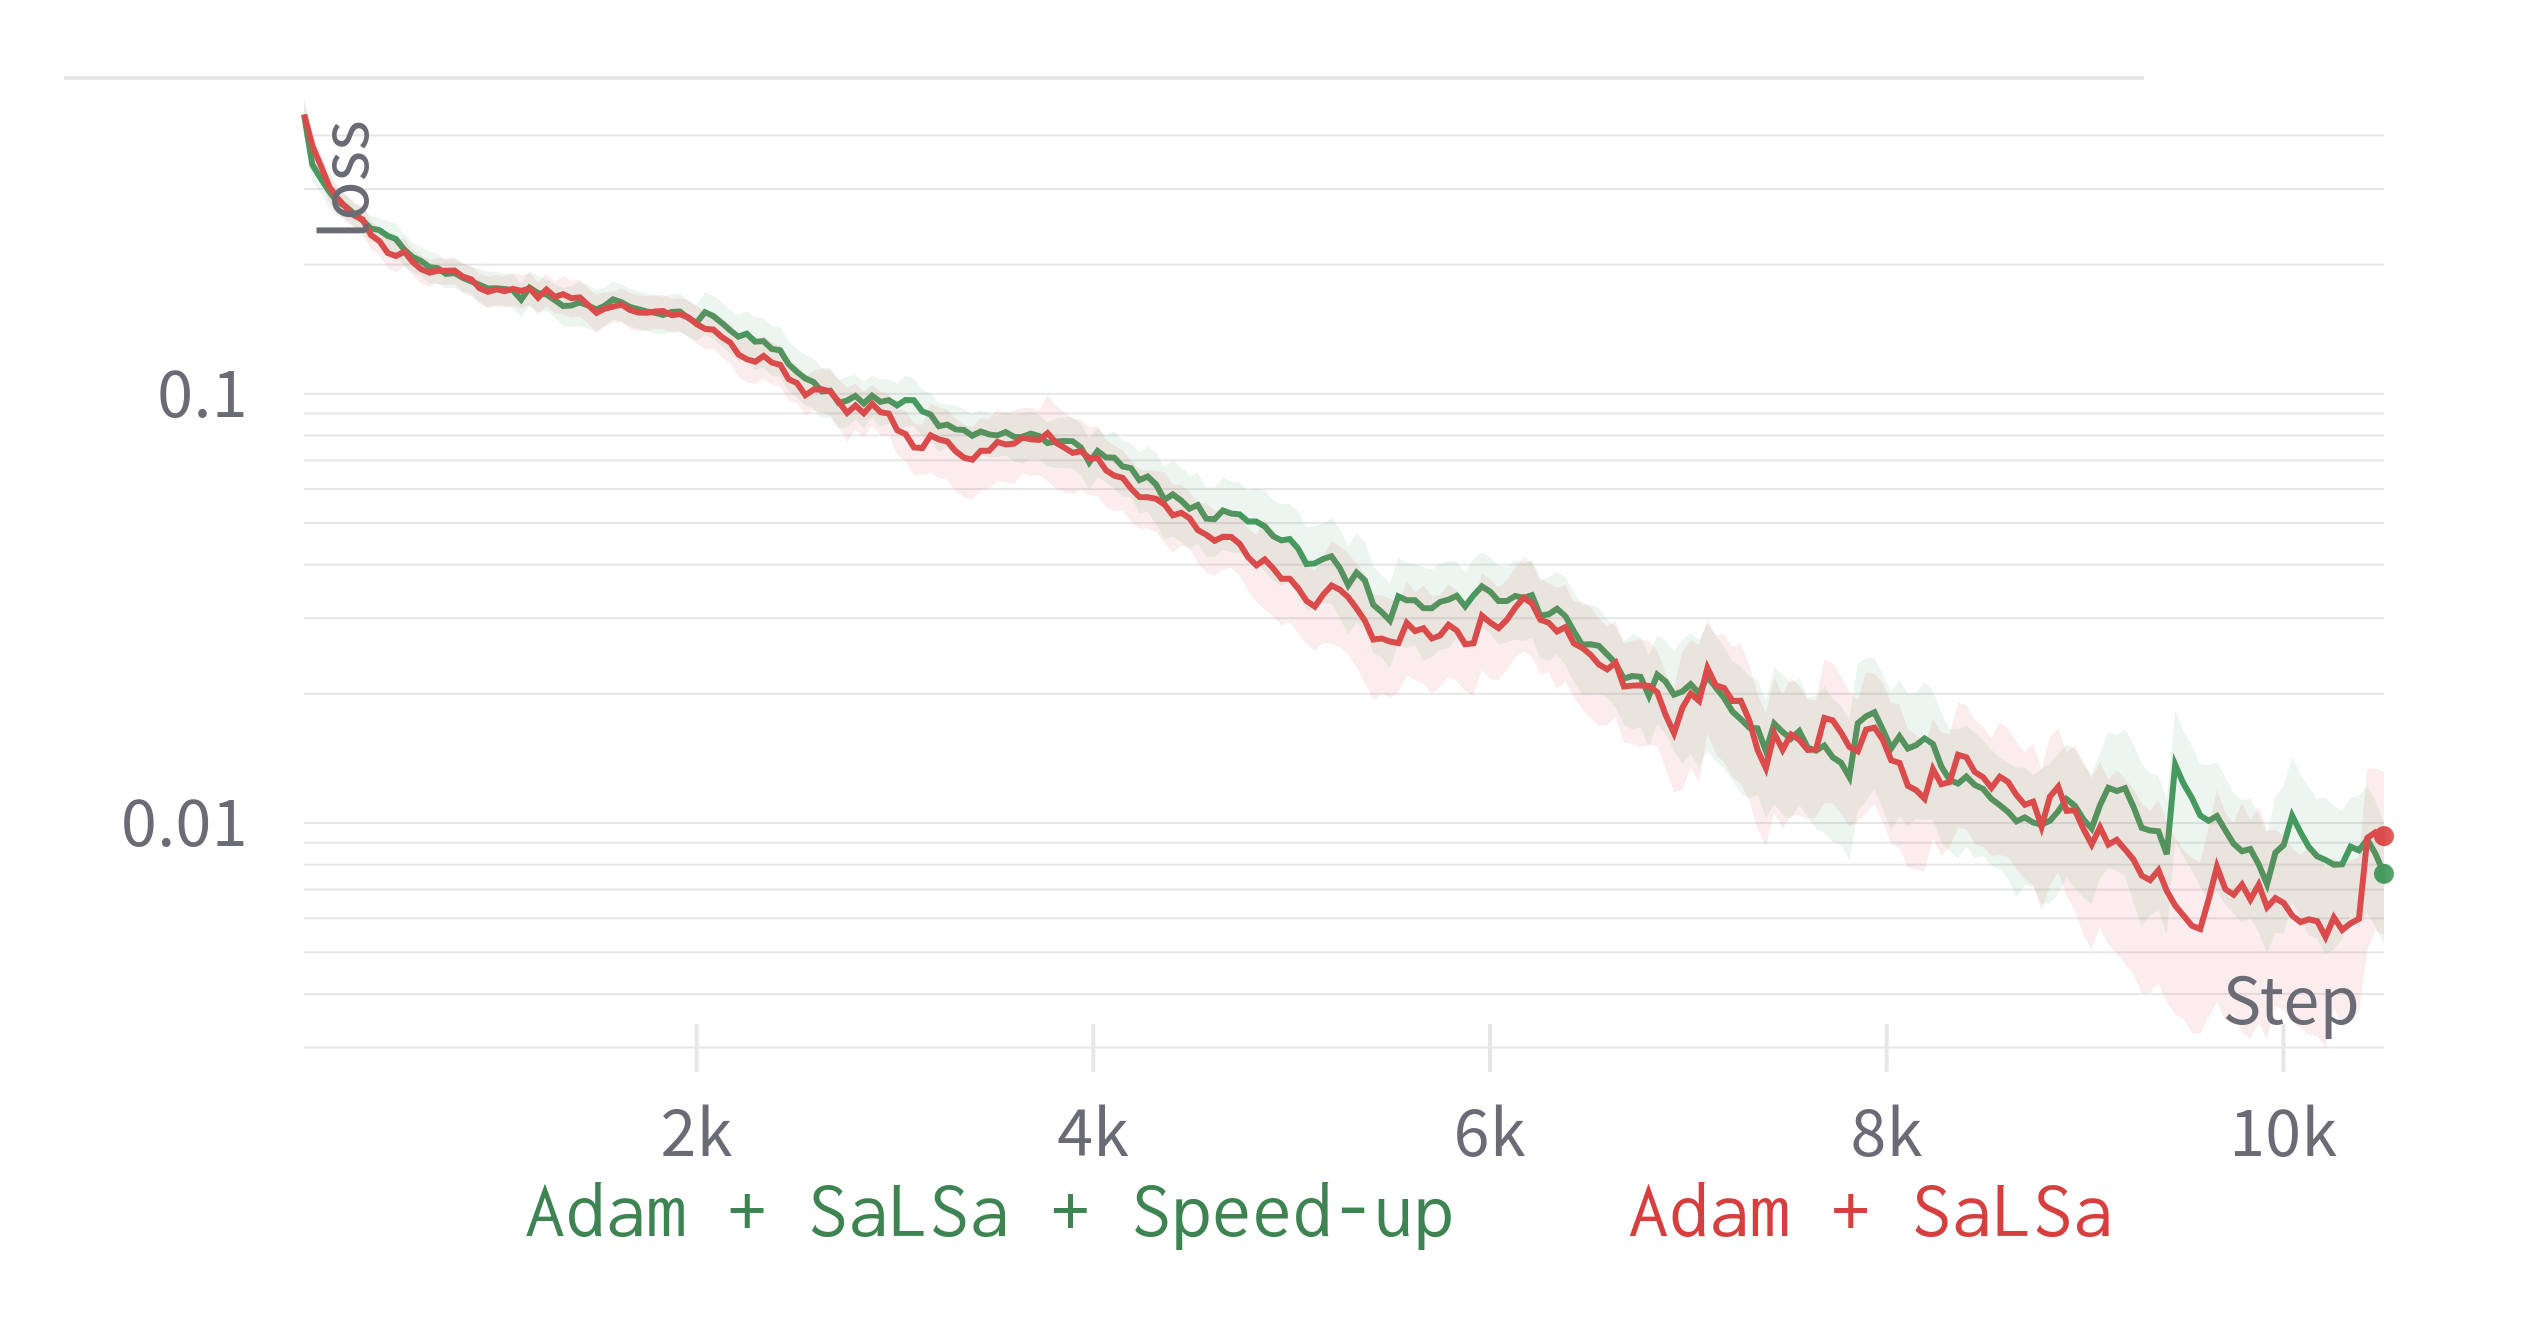}} 

\caption{Average loss curves with standard error indicated of training on the SST2, MNLI and QNLI dataset over 5 runs with and without the speed-up for the SaLSa + ADAM optimizer}
\label{fig:speeduploss}
\end{figure}

In \ref{fig:speedup} we can observe that $L_k$ is maximal $L_k=10$ during long plateaus of the step size, but decreases for faster changes in the step size.

\begin{figure}[h!]

\subfloat[$L_k$]{\includegraphics[width = 0.48\textwidth]{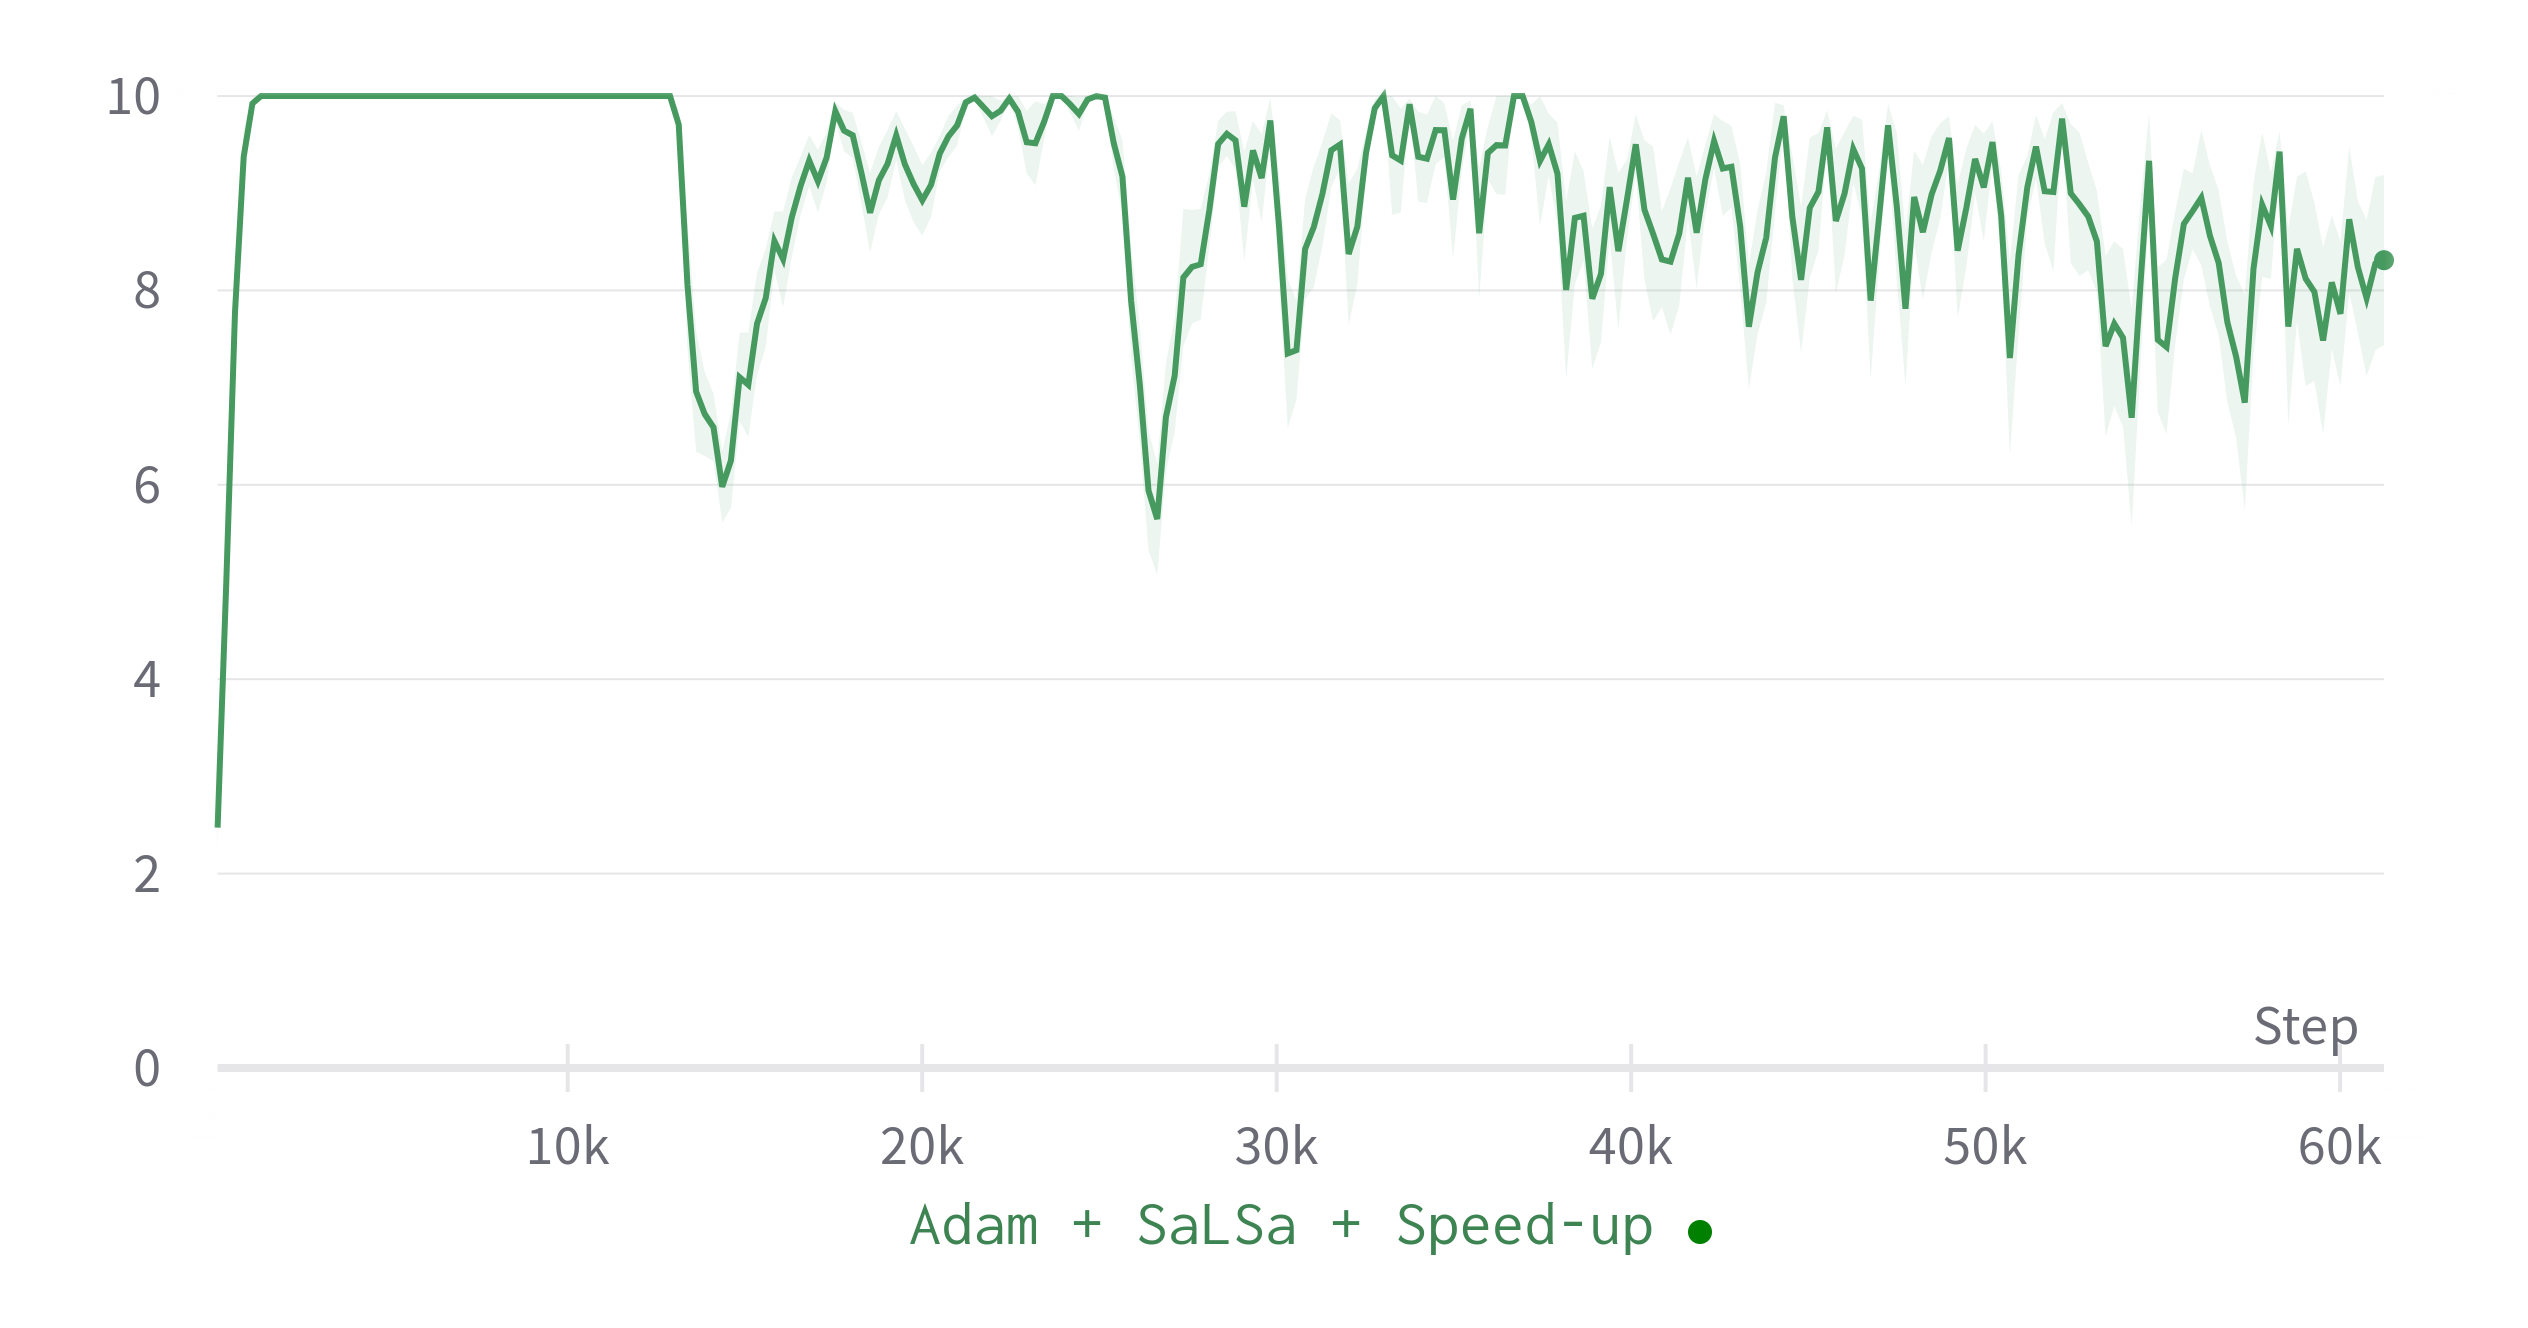}}
\subfloat[step size]{\includegraphics[width = 0.48\textwidth]{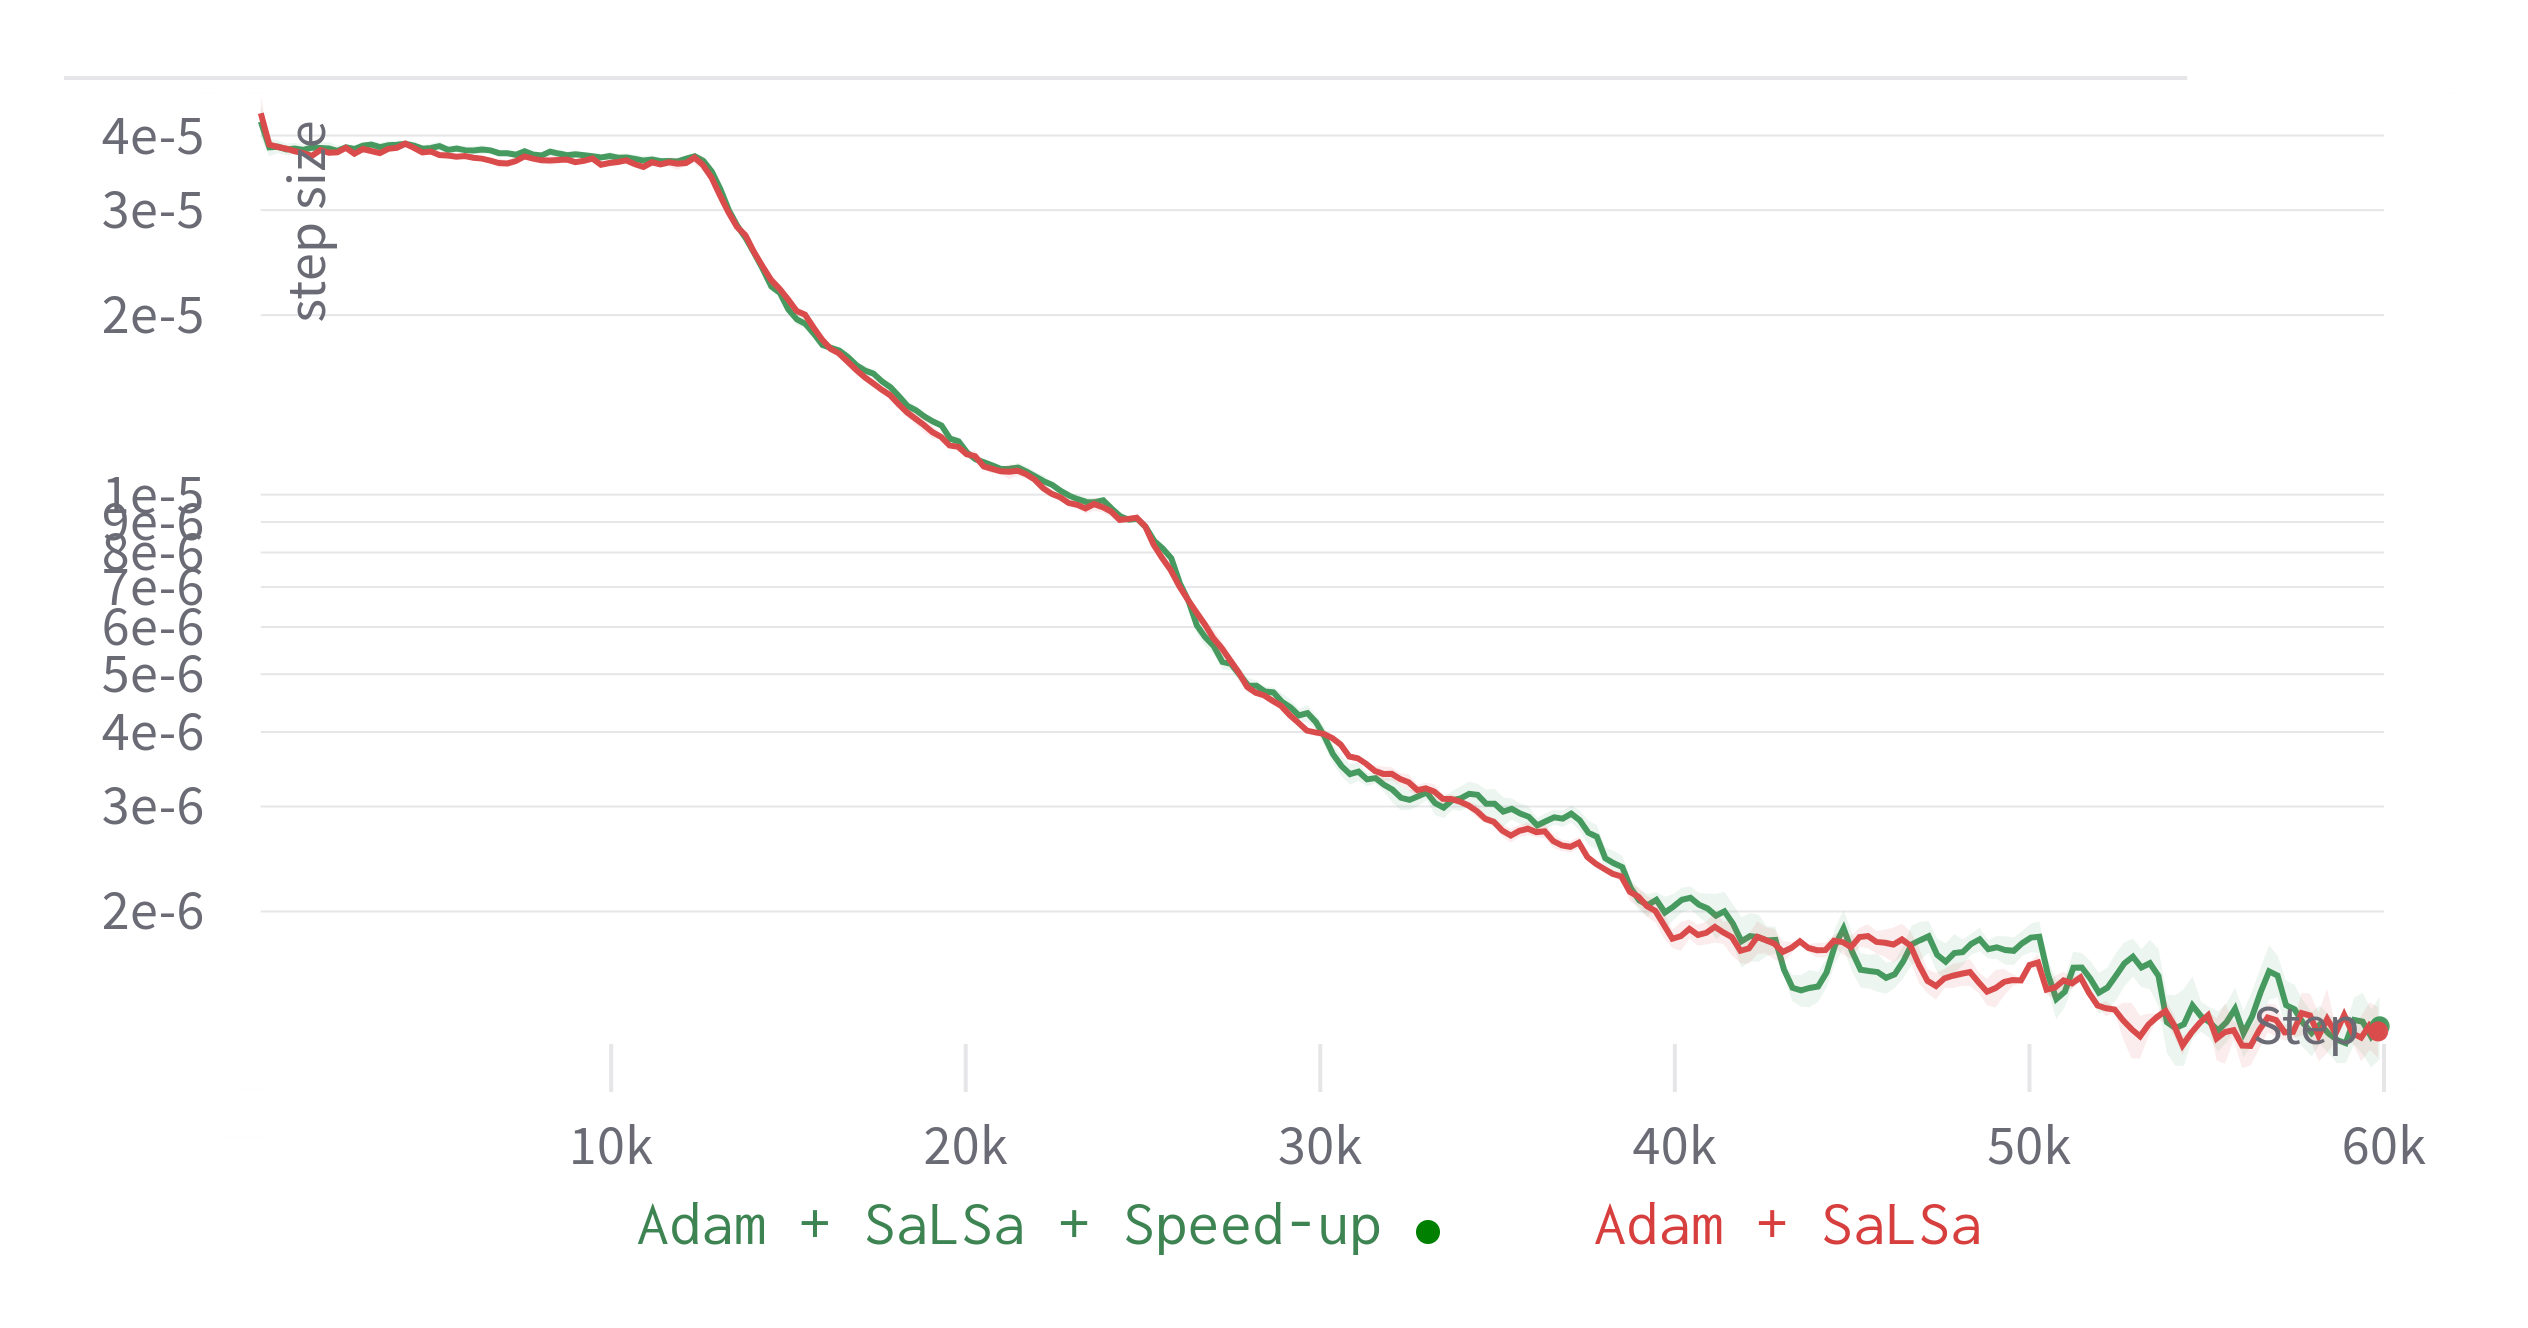}}

\caption{$L_k$ and step size curves with standard error indicated of training on the MNLI dataset over 5 runs with the SaLSa + ADAM + Speed-up optimizer}
\label{fig:speedup}
\end{figure}

\begin{figure}[h!]
\centering
\includegraphics[width = 0.48\textwidth]{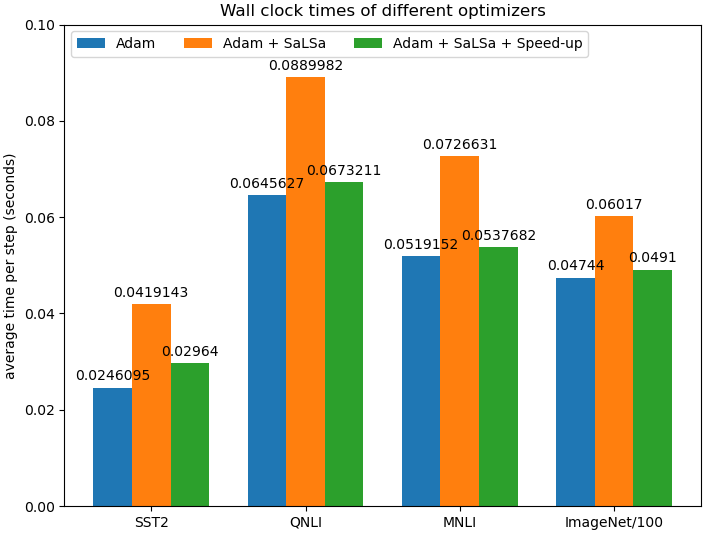}

\caption{Wall clock running times for different optimization methods and datasets. All experiments done on a single A40 GPU. ImageNet times are scaled down by a factor of 100.}
\label{fig:wallclock}
\end{figure}
